# Supplementary material for: Detection of adaptive shifts on phylogenies using shifted stochastic processes on a tree
Source: arXiv:1508.00225 source file (2016-07-13)
Supplement: Supplementary file 1 [file appendix.tex]

\appendix
\section{Technical Proofs of Section~3}\label{supp:proofs_identifiability}

   \begin{proof}[Proof of Proposition~\ref{prop:kernel_of_T}]
%       Let $K^i$ be a vector defined as in the proposition. Then
%       \begin{align*}
%       (TK^i)_j &= T_{ji}K^i_i + \sum_{l=1}^{L_i}T_{jd_l}K^i_{d_l}\\
%       & = T_{ji} - \sum_{l=1}^{L_i}T_{jd_l}\\
%       & = \Ibb\{i \in \Par(m+j)\} -  \sum_{l=1}^{L_i}\Ibb\{d_l \in \Par(m+j)\}
%       \end{align*}
%       If $i\notin \Par(m+j)$, then $d_l\notin \Par(m+j)$ for all $l\in \intervalleentier1{L_i}$ and $(TK^i)_j = 0$. Otherwise, $i$ is an ancestor of $m+j$. Since $i$ is internal, one of its direct descendant is also an ancestor of $m+j$, so that the sum cancels out.
Let $i\in\intervalleentier1m$ be an internal node with $L_i$ \PB{children} nodes $(d_1, \cdots, d_{L_i})$ and $\vect{K}^i$ the corresponding vector, defined as in the proposition. Then, for any $j\in \intervalleentier{1}{m+n}$:
      \[
      (\matr{U}\vect{K}^i)_j = U_{ji}K^i_i + \sum_{l=1}^{L_i}U_{jd_l}K^i_{d_l}
      %& = U_{ji} - \sum_{l=1}^{L_i}U_{jd_l}\\
       = \Ibb\{i \in \Par(j)\} -  \sum_{l=1}^{L_i}\Ibb\{d_l \in \Par(j)\}
      \]
      We can then distinguish three possibilities:
      \begin{itemize}
      \item If $i\notin \Par(j)$, then $d_l\notin \Par(j)$ for all $l\in \intervalleentier1{L_i}$ and $(\matr{T}\vect{K}^i)_j = 0$.
      \item If $j = i$, then $i \in \Par(j)$, and, by definition, $d_l \notin \Par(j)$ for any $l\in \intervalleentier1L$, so $(\matr{U}\vect{K}^i)_i = 1$.
      \item Else, if $i$ is an ancestor of $j$, with $i\neq j$, then, as $i$ is internal, one (and only one) of its \PB{child} $d_l$ is also an ancestor of $j$ (potentially $j$ itself), so that the sum cancels out.
      \end{itemize}
      This proves that 
      \begin{equation}
      \forall i \in \intervalleentier1m, \matr{U}\vect{K}^i = (\delta_{ij})_{1\leq j \leq m+n}
      \label{eq:kernel_of_T}
      \end{equation}
      %if $i \in \Par(m+j)$, then, as $m+j > i$, there is a unique $l\in\intervalleentier1{L_i}$ such that $d_l \in \Par(m+j)$, and $(TK^i)_j = 0$. 
      In particular, as $\matr{T}\vect{K}^i$ is the vector of the last $n$ coordinates of $\matr{U}\vect{K}^i$, this shows that the vectors $(\vect{K}^1, \cdots, \vect{K}^m)$ are in the kernel of $\matr{T}$.\par
      Then, as we found $m$ independent vectors in the kernel of $\matr{T}$, which is a space of dimension lower than $m$ (as the $n$ columns of $\matr{T}$ representing tips are linearly independent, and by the rank theorem), this family of vector is a basis of the kernel space.
      \end{proof}
      
            \begin{proof}[Proof of lemma~\ref{lemma:U_invertible}]
      First, $(\vect{b}_{m + 1}, \cdots, \vect{b}_{m+n})$ is a family of $n$ independent vectors of $S$ of dimension $n$, so is a basis of $S$, and $b'$ is a basis adapted to $\ker(\matr{T})\oplus S$.\par
      Let $i\in\intervalleentier{1}{m+n}$. Let's show that $\matr{U}\vect{b}'_{i} = \vect{b}_i$. If $m+1\leq i \leq m+n$, then $\vect{b}'_i = \vect{b}_i$, and $\matr{U}\vect{b}_i = \vect{b}_i$ is the $i^{th}$ column of $\matr{U}$. Otherwise, if $1\leq i \leq m$, then $\vect{b}'_i=\vect{K}^{i}${, and, from equation~\ref{eq:kernel_of_T}, $\matr{U}\vect{b}'_i = \vect{b}_i$.} This shows that $\matr{U}$ is the change of basis matrix between $b$ and $b'$.
      \end{proof}
      
                \begin{proof}[Proof of Proposition~\ref{prop:parsimony_linear_independence}]
      By contraposition, let's first assume that the vector-columns $(T_i)_{i\in\Supp(\vect{\Delta})}$ are linearly dependent, and prove that $\vect{\Delta}$ is not parsimonious. This means that we can find a vector $\vect{E}$, $\vect{E}\in\R^{m+n}$, such that $\Supp(\vect{E}) \subset \Supp(\vect{\Delta})$, and $\matr{T}\vect{E}=0$. We can hence find $j\in\Supp(\vect{\Delta})$, $j>1$, such that $E_j\neq 0$. Then if $\lambda = -\Delta_j/E_j$, the vector $\vect{\Delta}'=\vect{\Delta} + \lambda \vect{E}$ is a vector of shifts on the tree with one less non-zero coordinate than $\vect{\Delta}$ such that $\matr{T}\vect{\Delta}'=\vect{m_Y}$. Hence, $\vect{\Delta}$ is not parsimonious.\par
      Reciprocally, by contraposition, assume that $\vect{\Delta}$ is not parsimonious. Then by proposition~\ref{prop:Kshifts_K+1clusters}, it produces $p$ groups, with $p\leq K$. Hence the application associated with $(T_i)_{i\in\Supp(\vect{\Delta})}$ goes from a space of dimension $K+1$ to a space of dimension $p\leq K$, and hence is not injective, and the family $(T_i)_{i\in\Supp(\vect{\Delta})}$ is not independent.
      \end{proof}
\newpage
\section{Enumeration of Equivalence Classes}\label{supp:proofs_enumaration}

 \begin{definition}[Coloring concatenation]
       Let $i$ be a node of tree $\Tr$ with $L_i$ daughter nodes $(i_1, \cdots, i_{L_i})$, $L_i\geq 2$, and assume that the tips are colored according to the application $d\in (\Cr_K)^n$. We denote by $\Tr_i$ the sub-tree rooted at node $i$, and by $\Ar_{\Tr_i}(d)$ the set of parsimonious shifts allocations on $\Tr_i$ that produce a coloring of the tips compatible with $d$. At the root, $\Ar_{\Tr_1}(d) = \Ar_{\Tr}(d) = \phi^{-1}(d)$.
       \begin{itemize}
       \item For $k\in\Cr_K$, $S_i(k)$ is the \emph{cost} of starting from node $i$ with color $k$, \emph{i.e.} the minimal number of shifts needed to get the right coloring of the tips of $\Tr_i$, when starting with color $k$.
        \item $S_i^{tot} = \min_{k\in\Cr_K} S_i(k)$ is the minimal cost of subtree $\Tr_i$, \emph{i.e.} the number of shifts of a parsimonious coloring. $\Lr_i = \argmin_{k\in\Cr_K} S_i(k)$ is the set of colors root $i$ can take in a parsimonious coloring of sub-tree $\Tr_i$.
        \item For $k\in\Cr_K$, $\Br_{\Tr_i}^k$ is the set of colorings of $\Tr_i$ that respect the colors at the tips, have $S_i(k)$ shift, and start with color $k$.
        \item For $\Kr \subset \Cr_K$, $\Br_{\Tr_i}^\Kr = \bigcup_{k\in\Kr}\Br_{\Tr_i}^k$. Hence, $\Ar_{\Tr_i}(d) = \Br_{\Tr_i}^{\Lr_i}$, and the computation of $\Ar_{\Tr_i}(d)$ only requires the computation of $S_i(k)$ and $\Br_{\Tr_i}^k$ for any $k\in\Cr_K$.
        \item For $(p_1, \cdots, p_{L_i}) \in (\Cr_K)^{L_i}$, and $(B_1, \cdots, B_{L_i}) \in \Br_{\Tr_{i_1}}^{p_1} \times \cdots \times \Br_{\Tr_{i_{L_i}}}^{p_{L_i}}$ we define, for $k\in\Cr_K$, the concatenation 
        \(
         B = \sideset{^k}{}\bigoplus_{l=1}^{L_i} B_l, B \in \Br_{\Tr_i}^k,
        \)
        by:
        \(
         \begin{cases}
          B(i) = k\\
          B(j) = B_l(j) & \text{ if } i \in \Tr_{i_l}
         \end{cases}
        \).
  As the sub-trees $\Tr_{i_l}$, $l\in \intervalleentier1{L_i}$ do not overlap, this application is correctly defined on the nodes of $\Tr_i$.

       \end{itemize}

      \end{definition}
      
      Using these definitions, we can state the following recursion formula:
      
      \begin{proposition}[Enumeration Recursion Formula]\label{prop:recursion_eq_classes}
       Let $k\in\Cr_K$, and $i\in\intervalleentier{1}{m+n}$. If $i$ is a tip of the tree, then\\
    \begin{minipage}{0.5\textwidth}
 \[
  S_{i}(k) = \begin{cases}
           0 & \text{ if $d(i) = k$}\\
           +\infty & \text{ otherwise}
           \end{cases}
  \]
   \end{minipage}
   \begin{minipage}{0.5\textwidth}
 \[
  \Br_{\Tr_i}^{k} = \begin{cases}
           \{i\mapsto k\} & \text{ if $d(i) = k$}\\
           \emptyset & \text{ otherwise}
           \end{cases}
  \]
   \end{minipage}

       If $i$ is a node of tree $\Tr$ with ${L_i}$ daughter nodes $(i_1, \cdots, i_{L_i})$, ${L_i}\geq 2$, and assuming that $S_{i_l}(k)$ and $\Br_{\Tr_{i_l}}^k$ are known for any $l\in\intervalleentier1{L_i}$ and $k\in\Cr_K$, define, for $l\in\intervalleentier1{L_i}$:
        \[
    \Kr_k^l = \argmin_{1\leq p \leq K} \left\{ S_{i_l}(p) + \Ibb\{p \neq k\} \right\} 
	\]
	As these sets are not empty, let $(p_1, \dotsc p_{L_i}) \in \Kr_k^1 \times \dotsc \times \Kr_k^{L_i}$. Then
       \[
        S_i(k) = \sum_{l = 1}^{L_i} \left(S_{i_l}(p_l) + \Ibb\{p_l \neq k\}\right) 
        \quad \text{and} \quad
        \Br_{\Tr_i}^{k} = \left\{\sideset{^k}{}\bigoplus_{l=1}^{L_i} B_l : \forall l \in \intervalleentier{1}{L_i},  B_l \in \Br_{\Tr_{i_l}}^{\Kr_k^l}\right\}
       \]

%         \[
% 	  \forall k \in \Cr_K,~ \forall (p_1, \dotsc p_L) \in \Kr_k^1 \times \dotsc \times \Kr_k^L,~ \quad S_i(k) = \sum_{l = 1}^L \left(S_{i_l}(p_l) + \Ibb\{p_l \neq k\}\right)
% 	\]

      \end{proposition}
      
      \begin{proof}
       The actualization of $S_i(k)$ is the same as in the Sankoff algorithm \citep{sankoff1975}. The set $\Br_{\Tr_i}^{k}$ is then obtained by enumerating all the possible ways of concatenating children sets $\Br_{\Tr_{i_l}}^{\Kr_k^l}$, each of which is the ensemble of solutions for the sub-tree $\Tr_{i_l}$ that realize the minimal number of shifts when starting in state $k$.
       %For $\Br_{\Tr_i}^{k}$, we consider $\Br_{\Tr_{i_l}}^{\Kr_k^l}$ that is the ensemble of solutions for the sub-tree $\Tr_{i_l}$ that realize the minimal number of shifts when starting in state $k$. The concatenation just enumerate all the possible configurations of such optimal solutions on each sub-trees.
      \end{proof}
      
      Remarking that $T_i(k) = \card{\Br_{\Tr_i}^{k}}$, proposition \ref*{prop:size_eq_class} of the main text follows immediately.
\newpage
\section{A Vandermonde Like Identity}\label{supp:vandermonde}

\begin{proposition}

Let $(n,n') \in  N$ and $K \in \N$. With  the standard convention that
$\binom{n}{k} = 0$ if $n < k$, 
\begin{multline*}
\binom{n+n'-K}{K} = \sum_{k = 0}^K \binom{n-k}{k} \binom{n' - K + k}{K
  -k} \\ + \sum_{k = 0}^{K-1} \binom{(n-1)-k}{k} \binom{(n'-1) - (K-1) + k}{(K-1)
  -k}
\end{multline*}
which can be rewritten in a more symmetric way as:
\begin{multline}
  \label{eq:vandermonde_gen}
\binom{n+n'-K}{K}  =  \sum_{k,k'   \geq  0:  k+k'  =K}  \binom{n-k}{k}
\binom{n' - k'}{k'} \\ + \sum_{k,k' \geq 0: k+k' =K-1} \binom{(n-1)-k}{k} \binom{(n'-1) - k'}{k'}
\end{multline}

Similarly, 
\begin{multline*}
\binom{n+n'+1-K}{K} = \sum_{k = 0}^K \binom{n-k}{k} \binom{n' - K + k}{K
  -k} \\ + \sum_{k = 0}^{K-1} \binom{(n-1)-k}{k} \binom{n' - (K-1) + k}{(K-1)
  -k} + \binom{n-k}{k} \binom{(n'-1) - (K-1) + k}{(K-1) -k}
\end{multline*}
which can be rewritten in a more symmetric way as:
\begin{multline}
  \label{eq:vandermonde_gen_2}
\binom{n+n'+1-K}{K}  =  \sum_{k,k'   \geq  0:  k+k'  =K}  \binom{n-k}{k}
\binom{n'   -   k'}{k'}  \\   +   \sum_{k,k'   \geq   0:  k+k'   =K-1}
\binom{(n-1)-k}{k} \binom{n' - k'}{k'} + \binom{n-k}{k} \binom{(n'-1) - k'}{k'}
\end{multline}

\end{proposition}

Note that Eq~(\ref{eq:vandermonde_gen}) generalizes in some way the Vandermonde identity which states 
\begin{equation}
\label{eq:vandermonde}
\binom{n+n'}{K} = \sum_{k = 0}^K \binom{n}{k} \binom{n'}{K -k}
\end{equation}

Although  several  proofs  of   the  Vandermonde  identity  are  known
(geometric, algebraic and combinatorial),  we only provide a geometric
proof of this Vandermonde-like identity. 

Consider  a grid  of size  $(n+n') \times  K$.  We  are  interested in
grid-valued paths  that can move either  by $(1,0)$ or  by $(2,1)$. In
other words, if the $k^\text{th}$  position of a path is $(x_k, y_k)$,
then its next position $(x_{k+1}, y_{k+1})$ is either $(x_k + 1, y_k)$
or  $(x_k +  2, y_k  +1)$.   We are  interested in  paths starting  at
$(0,0)$ and ending at $(n+n', K)$.

Such a path consists of $K$ moves of type $(2,1)$ and $n+n'-2K$ moves of type
$(1, 0)$ and  is uniquely determined by the positions  of the moves of
the former type. There are $\binom {n+n'-2K + K}{K} = \binom
{n+n'-K}{K}$ distinct positions and therefore as many such paths. 

We now sort the paths according to the value $i$ they take when either
reaching  the line $x  = n$  or reaching  the line  $x =  n+1$ without
reaching the line  $x = n$ first.  We refer to  the latter paths as crossing
the line  $x = n$. Note that  this sorting induces a  partition of all
paths (see Figure~\ref{fig:vandermonde_1})

A path  reaching $x =  n$ at position  $i$ uniquely gives rise  to two
paths: one  from $(0,0)$ to $(n,  i)$ and one from  $(n,i)$ to $(n+n',
K)$  or equivalently  from $0$  to  $(n',K-i)$. There  are $\binom  {n
  -i}{i}$  different  paths  of  the  first kind  and  $\binom  {n'  -
  K-i}{K-i}$  of the second.   There are  therefore $\binom  {n -i}{i}
\binom {n' - K + i}{K - i}$ paths that pass through $(n,i)$.

A path crossing  the line $x=n$ and reaching the line  $x= n+1$ at $i$
must do so  with a last move of type $(2,  1)$.  It therefore uniquely
defines a path  from $(0,0)$ to $(n-1,i-1)$ and  a path from $(n+1,i)$
to $(n+n', K)$, or equivalently  from $(0, 0)$ to $(n'-1, K-i)$. There
are therefore $\binom {n -  i}{i - 1} \binom {n' - 1 -  K + i}{K - i}$
paths that cross the line $x = n$ and pass through $(n+1, i)$. 

Putting everything together, we get:
\begin{eqnarray*}
\binom{n+n'-K}{K} & = & \sum_{i = 0}^K \binom{n-i}{i} \binom{n'-K+i}{K-i}
+ \sum_{i = 0}^K \binom{n-i}{i - 1} \binom{n'- 1 - K+i}{K-i} \\ 
 & = & \sum_{i = 0}^K \binom{n-i}{i} \binom{n'-K+i}{K-i}
+ \sum_{i = 0}^{K-1} \binom{(n-1) -i}{i} \binom{(n'- 1) - (K-1) +i}{(K-1)-i}
\end{eqnarray*}
which is exactly Eq.~(\ref{eq:vandermonde_gen}). 

\begin{figure}
  \begin{center}    
    \includegraphics[width = 0.6\linewidth]{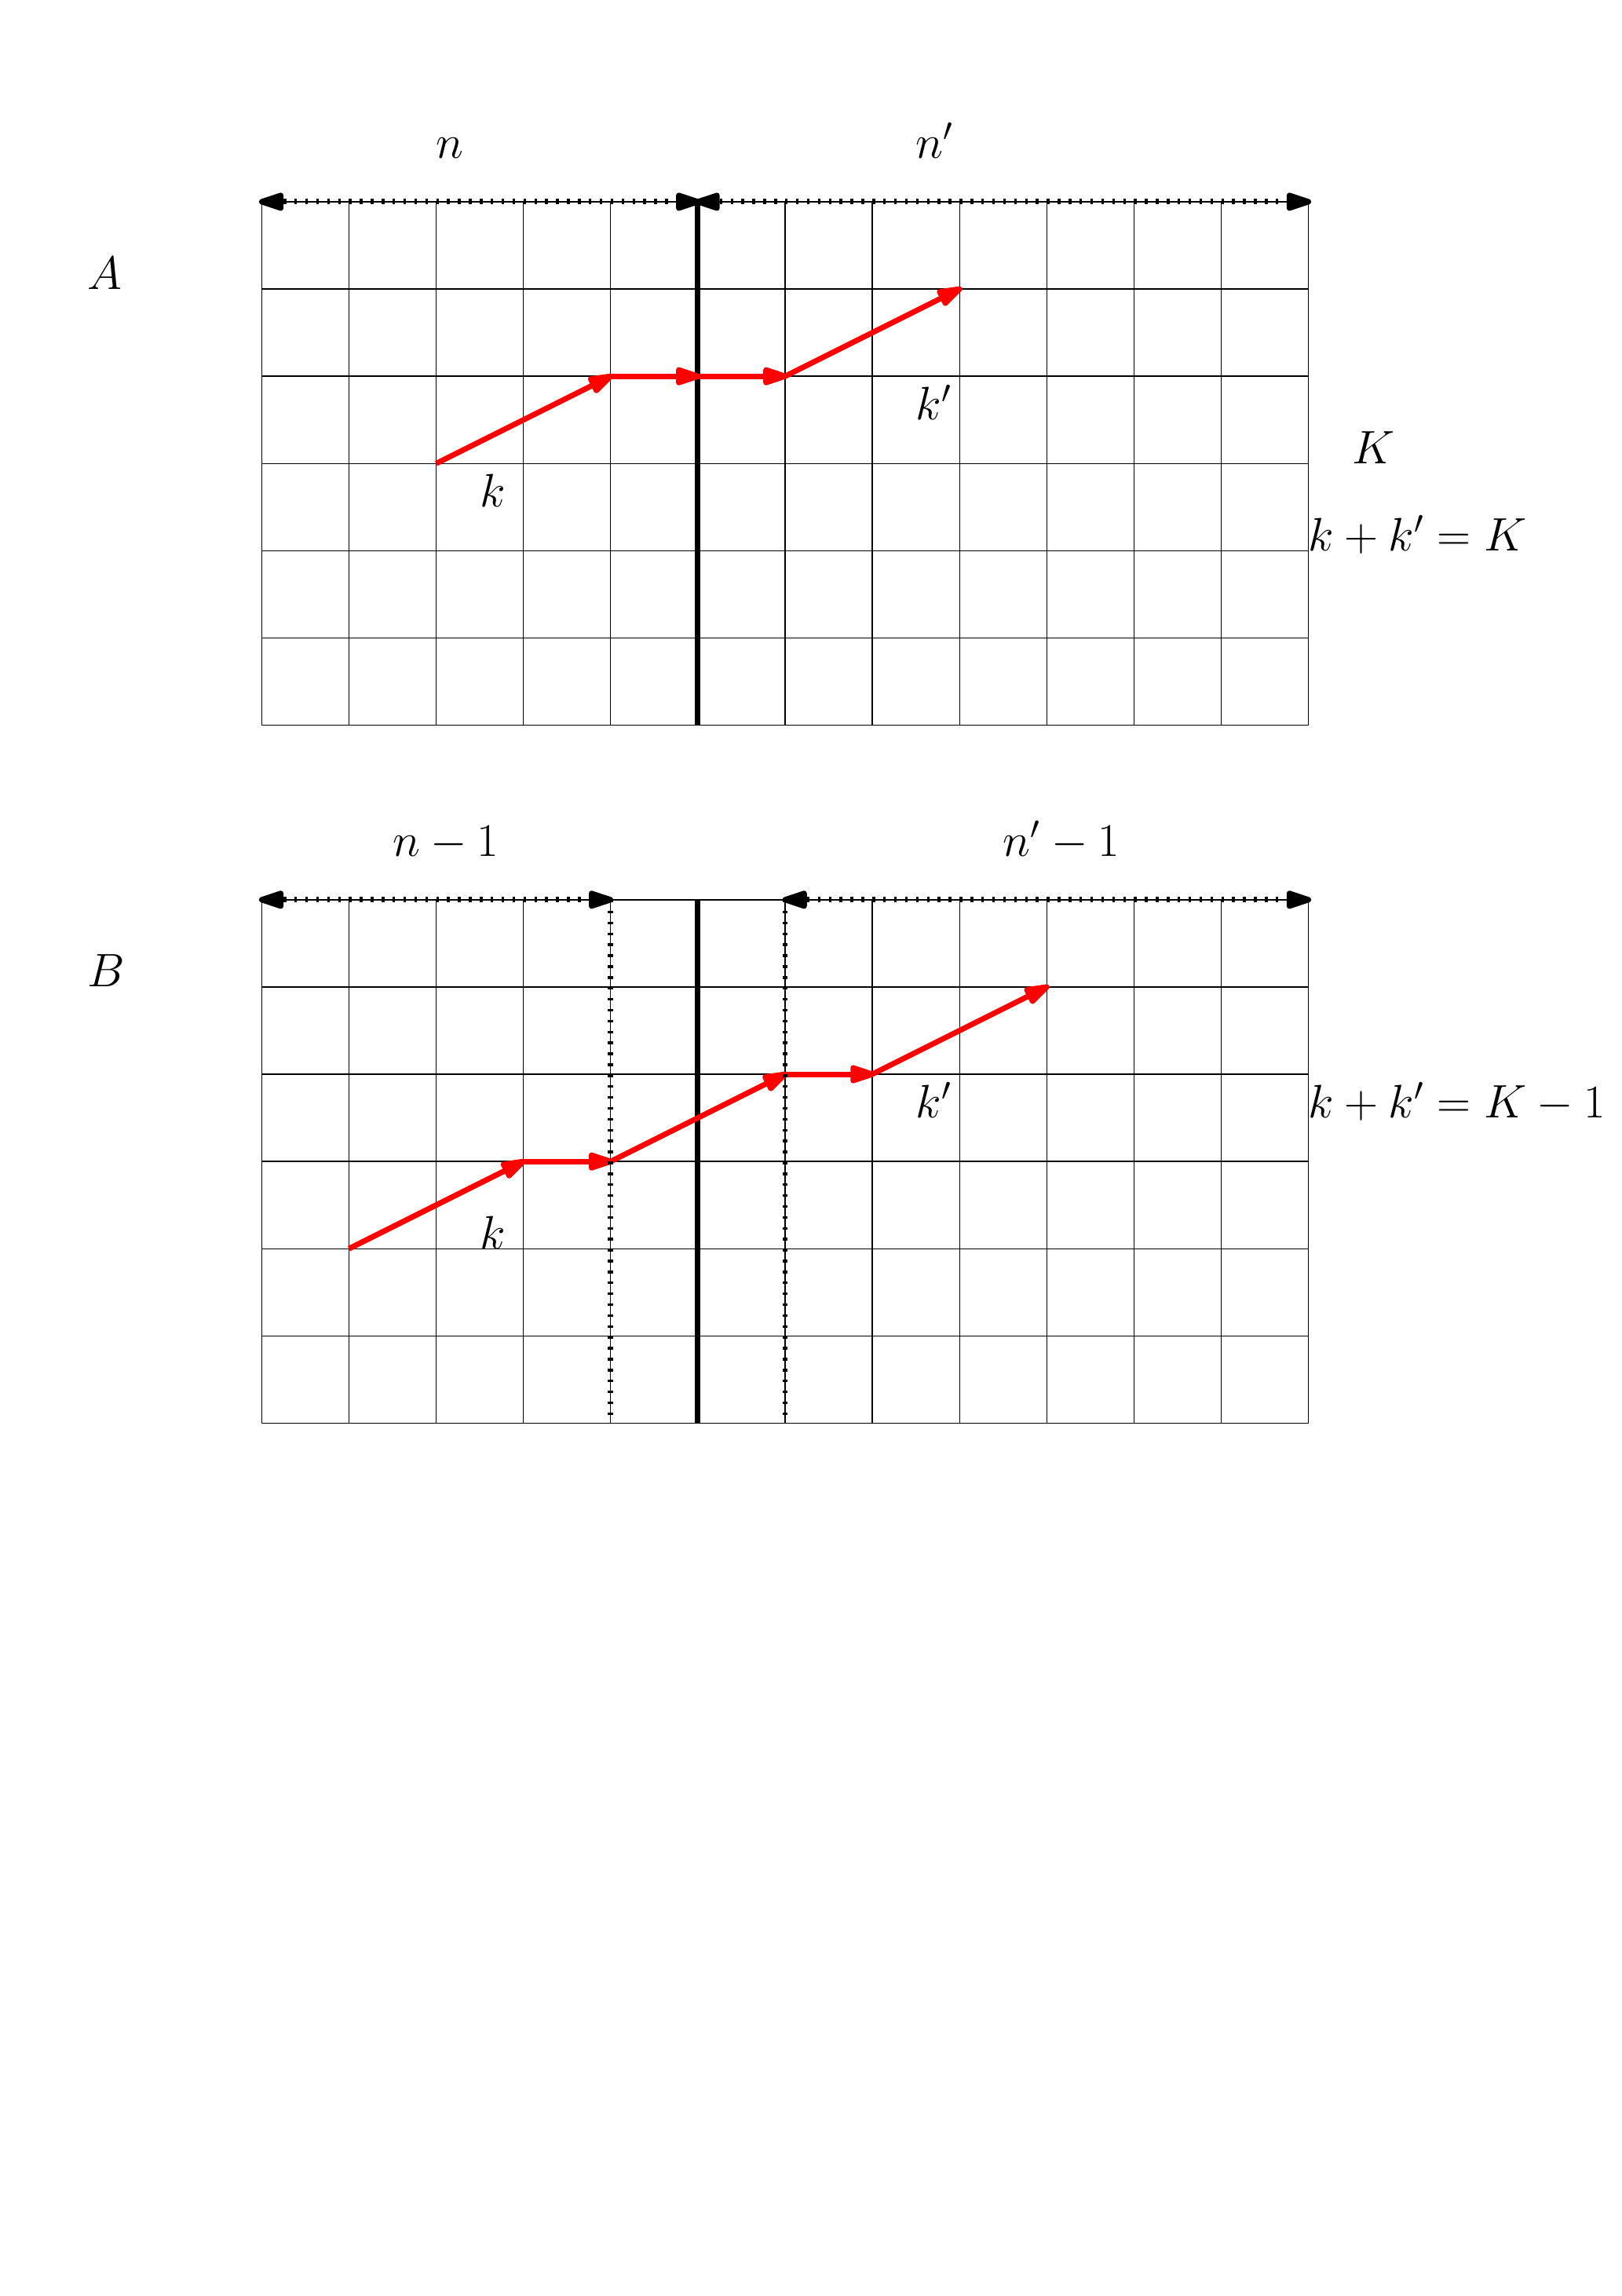}
    \caption{\label{fig:vandermonde_1}  Partition of paths  according to
      whether they reach (A) or cross (B) the line $x=n$}
  \end{center}
\end{figure}

To  prove Eq.~(\ref{eq:vandermonde_gen_2}),  we start  from a  grid of
size  $(n+n'+1)  \times K$  and  are  again  interested in  the  paths
starting from  the bottom  left corner and  ending in the  upper right
corner using  only (2, 1) and  (1, 0) moves. These  paths have exactly
$K$ moves  of type  (2, 1)  and there are  $\binom{n+n'+1 -  K}{K}$ of
them. This time, we partition paths upon the move observed between $x = n$
and $x=(n+1)$.

The move can be (see also Figure~\ref{fig:vandermonde_2}):
\begin{itemize}
\item (1, 0), in which case $k$ (resp. $k'$) moves of type $(2, 1)$
  are used in  the interval $[1, n]$ (resp.  $[n+1, n+n'1]$) such that
  $k + k' = K$;
\item (2, 1) starting from $x=n$ and therefore ending at $x=n+2$, in which case $k$
  (resp. $k'$)  moves of type $(2,  1)$ are used in  the interval $[1,
  n]$ (resp.  $[n+2, n+n'1]$) such that $k + k' = K - 1$ (one move (2,
  1) has already been consumed);
\item (2, 1) ending at $x=n+1$ and therefore starting from $x = n-1$ in which case $k$
  (resp. $k'$)  moves of type $(2,  1)$ are used in  the interval $[1,
  n-1]$ (resp.  $[n+1, n+n'1]$) such that $k + k' = K - 1$ (one move (2,
  1) has already been consumed);
\end{itemize}

Wrapping everything  together and using the same  arguments as before,
we get Eq.~(\ref{eq:vandermonde_gen_2}). 

\begin{figure}
  \begin{center}
    \includegraphics[width = 0.6\linewidth]{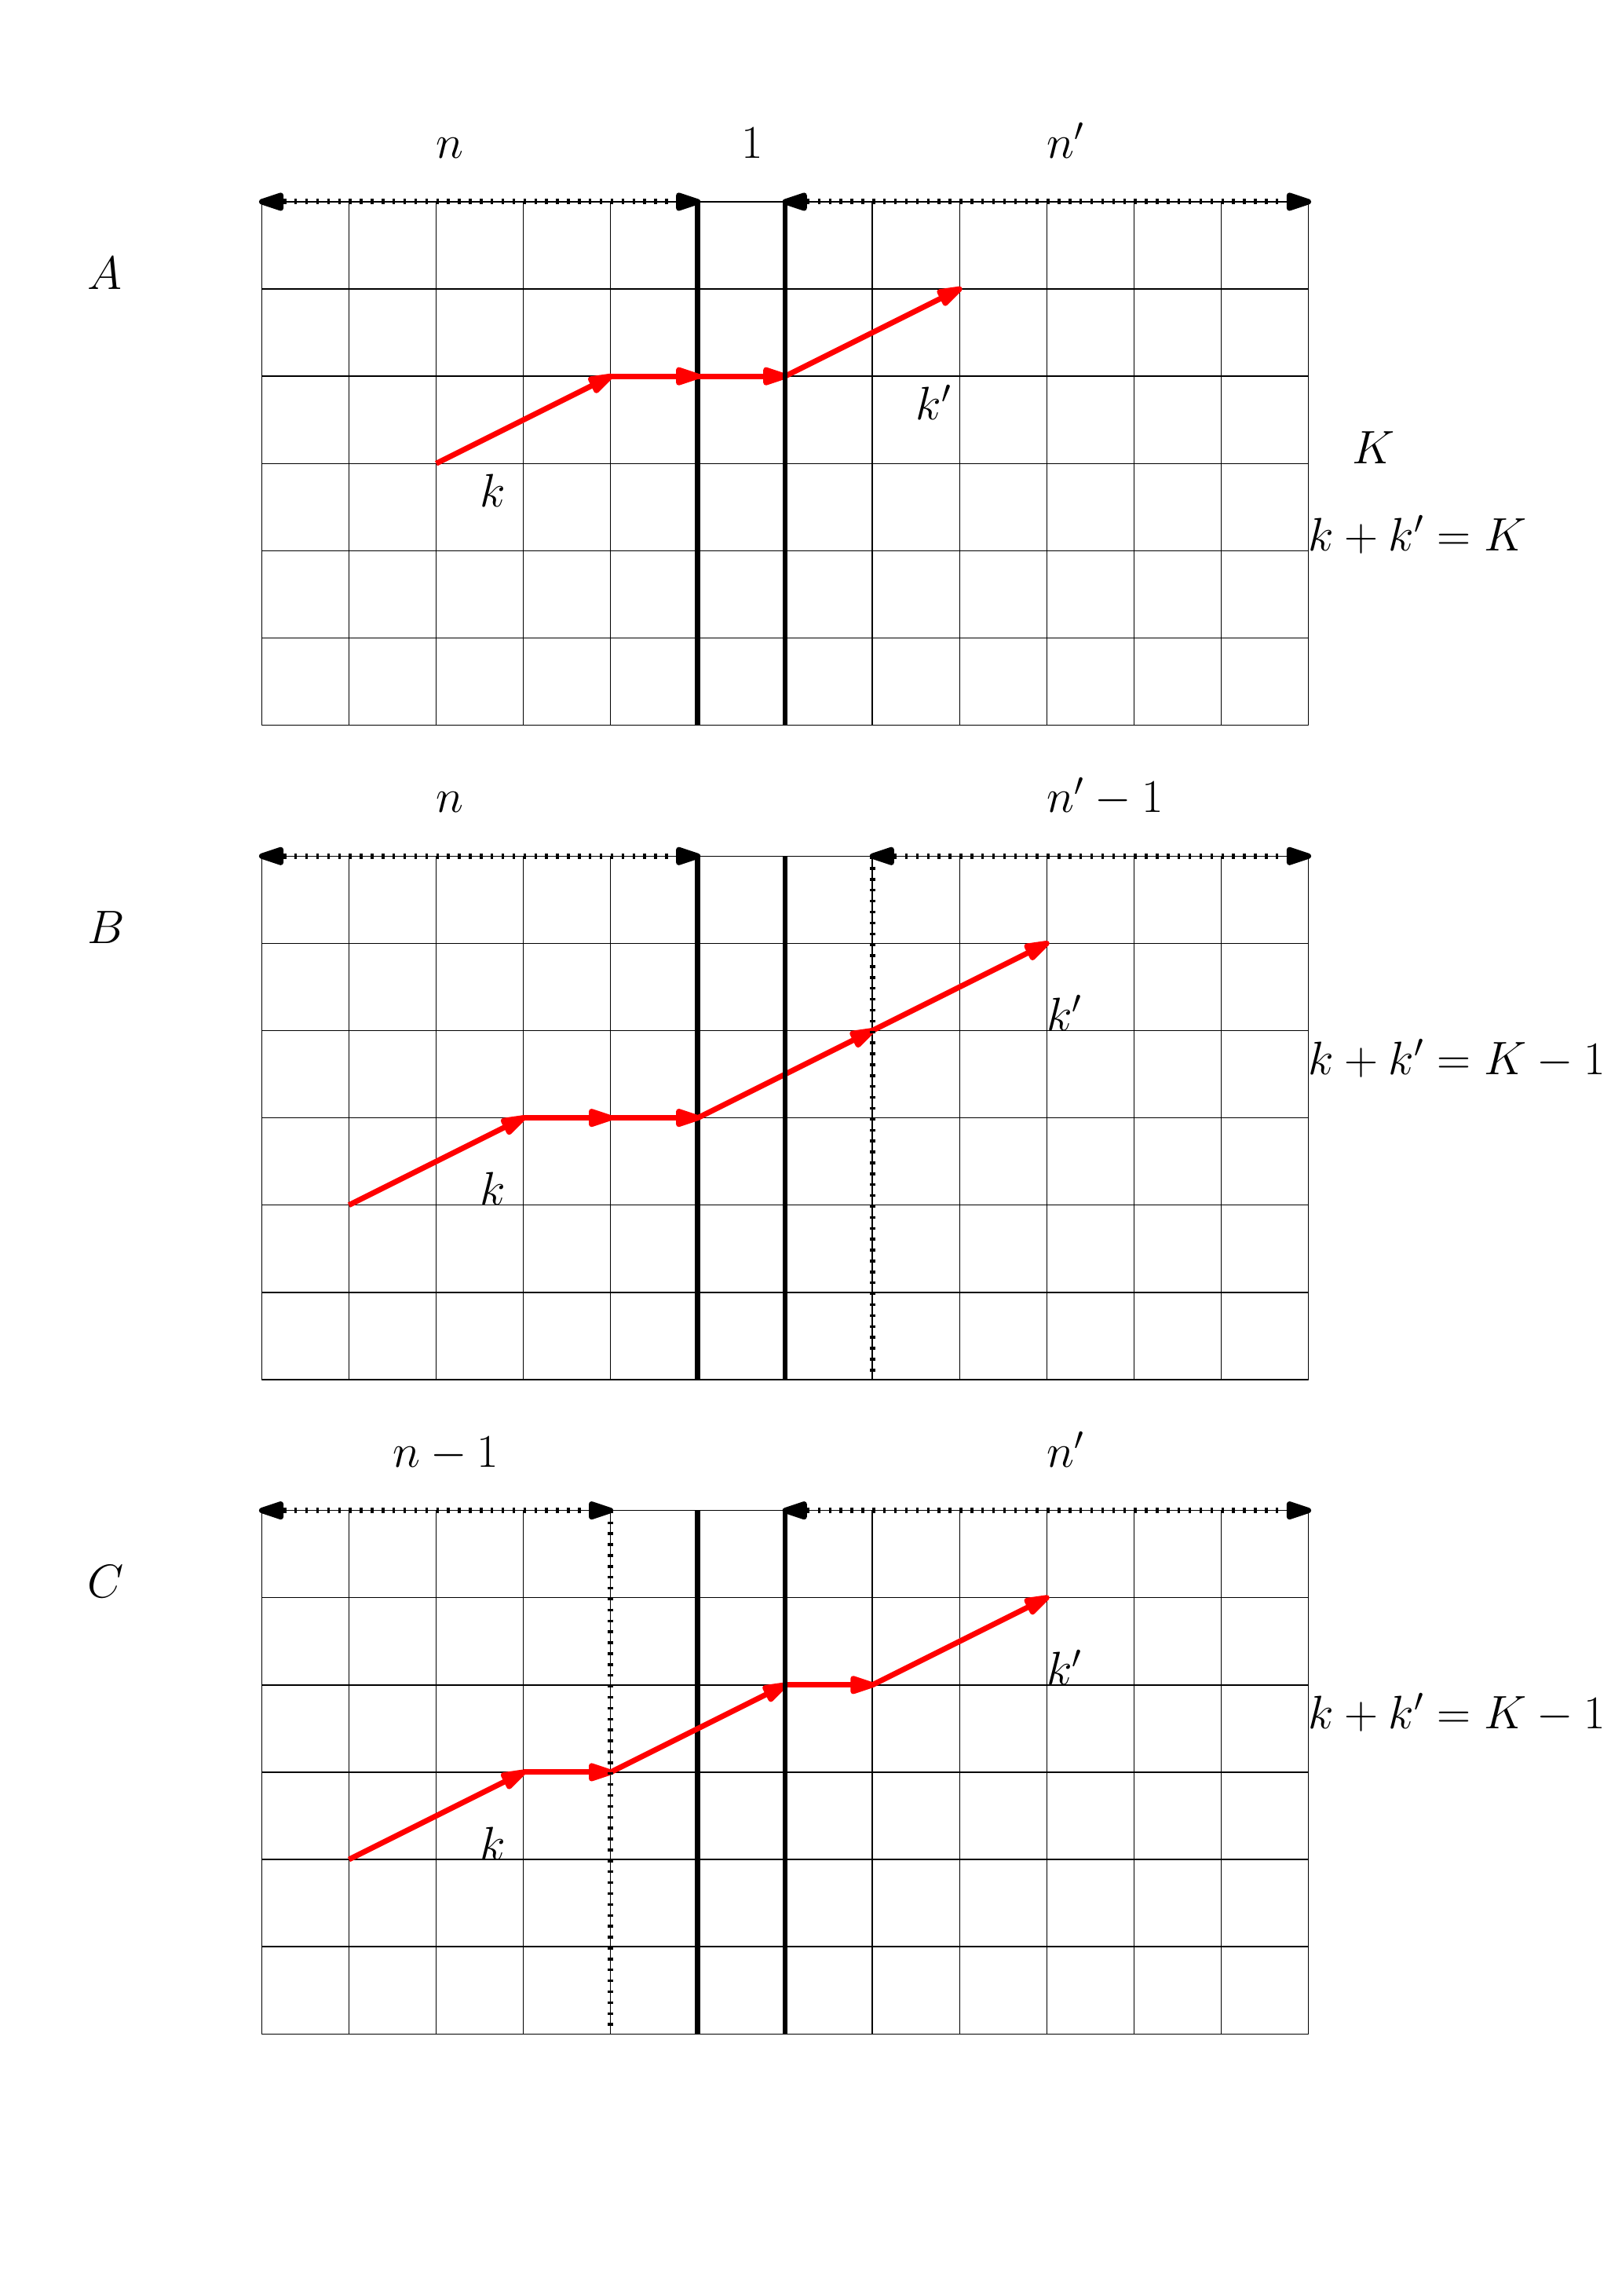}
    \caption{\label{fig:vandermonde_2}  Partition of paths  according to
      whether to  the move  used between $x=n$  and $x=n+1$. Cases  A, B
      and C correspond to the items listed in the main text.}
  \end{center}
\end{figure}

\newpage
%%%%%%%%%%%%%%%%%%%%%%%%%%%%%%%%%%%%%%%%%%%%%%%%%%%%%%%%%%%%%%%%%%%%%%%
%%%%%%%%%%%%%%%%%%%%%%%%%%%%%%%%%%%%%%%%%%%%%%%%%%%%%%%%%%%%%%%%%%%%%%%
\section{Technical Details of the EM} \label{supp:EM}
%%%%%%%%%%%%%%%%%%%%%%%%%%%%%%%%%%%%%%%%%%%%%%%%%%%%%%%%%%%%%%%%%%%%%%%
%%%%%%%%%%%%%%%%%%%%%%%%%%%%%%%%%%%%%%%%%%%%%%%%%%%%%%%%%%%%%%%%%%%%%%%

%%%%%%%%%%%%%%%%%%%%%%%%%%%%%%%%%%%%%%%%%%%%%%%%%%%%%%%%%%%%%%%%%%%%%%%
\subsection{E Step}\label{supp:E_step}

Given a set of parameters $\vvect{\theta}^{(h)}$, we have:
     \[
      \vect{X} = (\vect{Z}, \vect{Y}) \sim \Normal \left(  \vect{m}^{(h)} = \left(\begin{array}{c} \vect{m}^{(h)}_\vect{Z} \\ \vect{m}^{(h)}_\vect{Y} \end{array} \right) ~,~ \matr{\Sigma}^{(h)} = \left(\begin{array}{cc} \matr{\Sigma}^{(h)}_{\vect{Z}\vect{Z}} & \matr{\Sigma}^{(h)}_{\vect{Y}\vect{Z}} \\ \matr{\Sigma}^{(h)}_{\vect{Z}\vect{Y}} & \matr{\Sigma}^{(h)}_{\vect{Y}\vect{Y}} \end{array} \right)\right)
    \]
    hence:
    \[
    \begin{split}
    \sachant{\vect{Z}}{\vect{Y}} \sim \Normal \big(& \vect{m}^{(h)}_{\sachant{\vect{Z}}{\vect{Y}}} = \vect{m}^{(h)}_\vect{Z} + \matr{\Sigma}^{(h)}_{\vect{Z}\vect{Y}} (\matr{\Sigma}^{(h)}_{\vect{Y}\vect{Y}})^{-1} (\vect{Y} - \vect{m}^{(h)}_\vect{Y})
    ,\\
    & \matr{\Sigma}_{\sachant{\vect{Z}}{\vect{Y}}} = \matr{\Sigma}^{(h)}_{\vect{Z}\vect{Z}} - \matr{\Sigma}^{(h)}_{\vect{Z}\vect{Y}} (\matr{\Sigma}^{(h)}_{\vect{Y}\vect{Y}})^{-1} \matr{\Sigma}^{(h)}_{\vect{Y}\vect{Z}} \big)
    \end{split}
    \]
    
    \begin{remark}
    We can see that this approach forces us to invert $\matr{\Sigma}^{(h)}_{\vect{Y}\vect{Y}}$, a $n\times n$ matrix, which is a costly operation, of order $O(n^3)$. It also computes the complete matrix  $\matr{\Sigma}_{\sachant{\vect{Z}}{\vect{Y}}}$ whereas we only need a linear number of its coefficients: conditional variances and covariances of the form $\Covasq{\vect{Z}_{i}}{\vect{Z}_{\pa(i)}}{\vect{Y}}$. Due to the tree structure and to the Gaussian nature of the processes studied, it is possible to compute all the quantities needed in a linear time, using a ``forward-backward''-like algorithm (here,  ``upward-downward'', see \citet{lartillot2014} for a similar algorithm.). The upward step is similar to the pruning algorithm described in \citet[chap. 23]{felsenstein2004}. See also \citet{hoane2013b} for an algorithm linear in the number of iterations.
    \end{remark}

%%%%%%%%%%%%%%%%%%%%%%%%%%%%%%%%%%%%%%%%%%%%%%%%%%%%%%%%%%%%%%%%%%%%%%%
\subsection{Complete Likelihood Computation}\label{supp:likelihood}

Using the incomplete data model described in section \ref{subsec:latent_model}, we can write:
    \[
    p_{\vvect{\theta}}(\vect{X}) = p_{\vvect{\theta}}(X_1)\prod_{j=2}^{m+n}p_{\vvect{\theta}}\left(\sachant{X_j}{X_{\pa(j)}}\right)
    \]
    Taking the expectation, we get for the BM:
%     \begin{equation}\label{eq:BM_completed_log_lik}
%     \begin{split}
%     -2\log p_{\vvect{\theta}}(\vect{X}) = & (m+n)\log(2\pi) + 2\sum_{j=2}^{m+n}\log(\ell_j) + \log \gamma^2 + (m+n-1) \log \sigma^2 \\
%       & + \frac1{\gamma^2} \left(X_1 - \mu\right)^2 + \frac1{\sigma^2} \sum_{j = 2}^{m+n} \ell_j^{-1} \left(X_j - X_{\pa(j)}- \sum_k \Ibb\{\tau_k = b_j\} \delta_k\right)^2 \\
%     \end{split}
%     \end{equation}
%     and, for the OUsun:
%     \begin{equation}\label{eq:OU_completed_log_lik}
%       \begin{split}
%       -2\log p_{\vvect{\theta}}(\vect{X}) = &  (m+n)\log(2\pi) + 2\sum_{j=2}^{m+n}\logc_j(\alpha) + (m+n) \log (\gamma^2) \\
%   & + \frac1{\gamma^2} \left(X_1 - \mu\right)^2 + \frac{1}{\gamma^2} \sum_{j=2}^{m+n} c_j(\alpha)^{-1}  \left(  X_j - X_{\pa(j)}e^{-\alpha \ell_j} - \beta^{j}\left(1 - e^{-\alpha \ell_j}\right)\right)^2\\
%       \end{split}
%      \end{equation}
%     Taking the expectation, we get:
    \begin{equation} \label{eq:BM_expectation_completed_log_lik}
      \begin{split}
	-2\Espesq{\log p_{\vvect{\theta}}(\vect{X})}{\vect{Y}}
	 & =  A + \log \gamma^2 + \frac{1}{\gamma^2} \left( \Varisq{X_1}{\vect{Y}} + \left(\Espesq{X_1}{\vect{Y}} - \mu\right)^2\right) \\
	  & + (m+n-1) \log \sigma^2 + \frac1{\sigma^2} \sum_{j=2}^{m+n} \ell_j^{-1} \Varisq{X_j - X_{\pa(j)}}{\vect{Y}}\\
	  % & + \frac1{\sigma^2} \sum_{j=2}^{m+n} C_j^{BM}(\vvect{\tau}, \vvect{\delta}) \\
	  & + \frac1{\sigma^2} \sum_{j=2}^{m+n} C_j^{BM}(\PB{\vect{\Delta}}) \\
	\end{split}
%  \raisetag{-2.5 cm}
    \end{equation}
    and, for the OUsun:
    \begin{equation}\label{eq:OU_expectation_completed_log_lik}
      \begin{split}
	-2\Espesq{\log p_{\vvect{\theta}}(\vect{X})}{\vect{Y}} & = B + \sum_{j=2}^{m+n}\log c_j(\alpha) + \frac{1}{\gamma^2} \Varisq{X_1}{\vect{Y}} + (m+n) \log \gamma^2\\
	  & + \frac{1}{\gamma^2} \sum_{j=2}^{m+n} c_j(\alpha)^{-1} \Varisq{X_j - X_{\pa(j)}e_j}{\vect{Y}}\\
%	  & + \frac{1}{\gamma^2}\left(\Espesq{X_1}{\vect{Y}} - \beta_0\right)^2 + \frac{1}{\gamma^2} \sum_{j=2}^{m+n} C_j^{OU}(\vvect{\tau}, \vvect{\delta}, \beta_0, \alpha)
	 & + \frac{1}{\gamma^2}\left(\Espesq{X_1}{\vect{Y}} - \beta_0\right)^2 + \frac{1}{\gamma^2} \sum_{j=2}^{m+n} C_j^{OU}(\alpha, \PB{\vect{\Delta}})
	\end{split}
%  \raisetag{-2.5 cm}
     \end{equation}
    where $A$ and $B$ are constants, and for each node $j$, $j \in \intervalleentier{2}{m+n}$, we define an actualization factor $c_j(\alpha) = 1-e_j(\alpha)^2$, with $e_j(\alpha) = e^{-\alpha\ell_j}$, and $C_j^{BM}$ and $C_j^{OU}$ are \emph{costs} associated with branch $b_j$:
    \[
      \left\{
	\begin{aligned}
%	 C_j^{BM}(\vvect{\tau}, \vvect{\delta}) & = \frac{1}{\ell_j} \left(\Espesq{X_j}{\vect{Y}} - \Espesq{X_{\pa(j)}}{\vect{Y}} - \sum_{k=1}^K \Ibb\{\tau_k = b_j\} \delta_k\right)^2\\
%	 C_j^{OU}(\vvect{\tau}, \vvect{\delta}, \beta_0, \alpha) &= \frac{1}{c_j(\alpha)} \Bigg(\Espesq{X_j}{\vect{Y}} - e_j\Espesq{X_{\pa(j)}}{\vect{Y}} - \beta_{j}\left(1 - e_j\right) \Bigg)^2
	 C_j^{BM}(\PB{\vect{\Delta}}) & = \frac{1}{\ell_j} \left(\Espesq{X_j}{\vect{Y}} - \Espesq{X_{\pa(j)}}{\vect{Y}} - \PB{\Delta_i}\right)^2\\
	 C_j^{OU}(\alpha, \PB{\vect{\Delta}}) &= \frac{1}{c_j(\alpha)} \Bigg(\Espesq{X_j}{\vect{Y}} - e_j\Espesq{X_{\pa(j)}}{\vect{Y}} - \beta_{j}\left(1 - e_j\right) \Bigg)^2
	\end{aligned}
      \right.
    \]

%%%%%%%%%%%%%%%%%%%%%%%%%%%%%%%%%%%%%%%%%%%%%%%%%%%%%%%%%%%%%%%%%%%%%%%
\subsection{M step}\label{supp:M_step}
Assuming that $p_{\vvect{\theta}^{(h)}}(\sachant{\vect{Z}}{\vect{Y}})$ is known, we need to compute $\vvect{\theta}^{(h+1)}$ by maximizing $\Esp_{\vvect{\theta}^{(h)}}[\sachant{\log p_{\vvect{\theta}}(\vect{Z},\vect{Y})}{\vect{Y}}]$. We have to deal with parameters of different nature, discrete or continuous. 
    %To choose the location $\vvect{\tau}^{(h+1)}$ and intensity $\vvect{\delta}^{(h+1)}$ of the $K$ shifts, we use a segmentation algorithm, as described below. 
    For a given \PB{vector $\vect{\Delta}^{(h+1)}$ of $K$ non-zero shifts,}
%     location $\vvect{\tau}^{(h+1)}$ and intensity $\vvect{\delta}^{(h+1)}$ of the $K$ shifts, 
we can exhibit closed formulas for $\mu^{(h+1)}$, $\sigma^{(h+1)}$ and $\gamma^{(h+1)}$, for the BM:
    \begin{equation*}
      \left\{
  \begin{aligned}
	  \mu^{(h+1)} & =  \Esp^{(h)}[ Z_1 \mid \vect{Y}] \\
	  \gamma^{2(h+1)} & =  \Var^{(h)}[Z_1 \mid \vect{Y}] \\
	  \sigma^{2(h+1)} & =
%	  	  \frac1{m+n-1} \left[ \sum_{j=2}^{m+n} \ell_j^{-1} \Var^{(h)} \left[X_j - X_{\pa(j)} \mid \vect{Y} \right] + C_j^{BM}\left(\vvect{\tau}^{(h+1)}, \vvect{\delta}^{(h+1)}\right) \right]
	  \frac1{m+n-1} \left[ \sum_{j=2}^{m+n} \ell_j^{-1} \Var^{(h)} \left[X_j - X_{\pa(j)} \mid \vect{Y} \right] + C_j^{BM}\left( \PB{\vect{\Delta}^{(h+1)}}\right) \right]
	\end{aligned}
      \right.
     \end{equation*}
    and, for the OUsun:
     \[
     \begin{split}
	(m+n) \gamma^{2(h+1)} &= \Var^{(h)}[X_1 \mid \vect{Y}]  + \sum_{j=2}^{m+n} c_j(\alpha)^{-1} \Var^{(h)} \left[X_j - X_{\pa(j)}e^{-\alpha \ell_j} \mid \vect{Y} \right]\\
%		  & + \left(\Esp^{(h)}\left[\sachant{X_1}{\vect{Y}}\right] - \beta^{(h+1)}_0\right)^2 + \sum_{j=2}^{m+n} C_j^{OU}\left(\vvect{\tau}^{(h+1)},\vvect{\delta}^{(h+1)}, \beta^{(h+1)}_0, \alpha^{(h)}\right)\\
	  & + \left(\Esp^{(h)}\left[\sachant{X_1}{\vect{Y}}\right] - \beta^{(h+1)}_0\right)^2 + \sum_{j=2}^{m+n} C_j^{OU}\left(\alpha^{(h)},  \PB{\vect{\Delta}^{(h+1)}}\right)\\
      \end{split}
      \]
    There is no such closed formula for $\alpha$. In the implementation we propose, this parameter is actualized after all the others, by doing a numerical maximization of the objective function.\par
    Finally, the \PB{vector $\vect{\Delta}^{(h+1)}$ of $K$ non-zero shifts}
%     location $\vvect{\tau}^{(h+1)}$ and intensity $\vvect{\delta}^{(h+1)}$ of the $K$ shifts
      can be chosen in an optimal way for the BM thanks to a simple algorithm explained below. In the OUsun case, we can only increase the objective function, and not maximize it. In that case, we hence use a Generalized EM algorithm \citep[GEM, see][]{dempster1977}.
    
    \paragraph{Optimal Shift Location for the BM} We want to minimize the sum of costs: 
%    \[C^{BM}(\vvect{\tau}, \vvect{\delta}) = \sum_{j=2}^{m+n}C_j^{BM}(\vvect{\tau}, \vvect{\delta})\] 
%    Each cost is associated to a branch $b_j$, $j\in\intervalleentier{2}{m+n}$, and, when the sum is minimal, $C_j^{BM}(\vvect{\tau}, \vvect{\delta})$ can only take two values: 
%    \begin{equation*}
%    \begin{cases}
%    \tilde{C}_j^{BM} = \ell_j^{-1} \left(\Esp^{(h)}\left[\sachant{X_j}{\vect{Y}}\right] - \Esp^{(h)}\left[\sachant{X_{\pa(j)}}{\vect{Y}}\right]\right)^2 & \text{if no shift on branch $b_j$} \\
%    0 & \text{if one shift on branch $b_j$}
%    \end{cases}
%    \end{equation*}
        \[C^{BM}(\vect{\Delta}) = \sum_{j=2}^{m+n}C_j^{BM}(\PB{\vect{\Delta}})\] 
    Each cost is associated to a branch $b_j$, $j\in\intervalleentier{2}{m+n}$, and, when the sum is minimal, $C_j^{BM}(\PB{\vect{\Delta}})$ can only take two values: 
    \begin{equation*}
    \begin{cases}
    \tilde{C}_j^{BM} = \ell_j^{-1} \left(\Esp^{(h)}\left[\sachant{X_j}{\vect{Y}}\right] - \Esp^{(h)}\left[\sachant{X_{\pa(j)}}{\vect{Y}}\right]\right)^2 & \text{if no shift on branch $b_j$} \\
    0 & \text{if one shift on branch $b_j$}
    \end{cases}
    \end{equation*}
%     either $\tilde{C}_j^{BM}(\vvect{\tau}, \vvect{\delta}) = \ell_j^{-1} \left(\Esp^{(h)}\left[\sachant{X_j}{\vect{Y}}\right] - \Esp^{(h)}\left[\sachant{X_{\pa(j)}}{\vect{Y}}\right]\right)^2$ if there is no shift on branch $b_j$, or $0$ if there is a shift of the right intensity (see below) on branch $b_j$.
    The sum can hence be minimized in the following way:
    \begin{enumerate}
     \item Compute $\tilde{C}_j^{BM}$ for all $j\in\intervalleentier{2}{m+n}$.
     \item Find the $K$ highest costs $(j_1, \cdots, j_K)\in\intervalleentier{2}{m+n}^K$.
%     \item Set $b^{(h+1)}_k = b_{j_k}$ and $\vvect{\delta}^{(h+1)}_k = \Esp^{(h)}\left[\sachant{X_j}{\vect{Y}}\right] - \Esp^{(h)}\left[\sachant{X_{\pa(j)}}{\vect{Y}}\right]$ for all $k\in\intervalleentier1K$.
     \item \PB{Set $\Delta^{(h+1)}_{j_k} = \Esp^{(h)}\left[\sachant{X_{j_k}}{\vect{Y}}\right] - \Esp^{(h)}\left[\sachant{X_{\pa(j_k)}}{\vect{Y}}\right]$ for all $k\in\intervalleentier1K$, and $\Delta^{(h+1)}_{j} = 0$ if $j \notin \{j_1, \cdots, j_K\}$.}
    \end{enumerate}
    This exact and fast algorithm works for the BM because all the costs are independent. Note that it would work for any Levy Process without memory, such as those proposed in \citet{landis2013} to model evolution of quantitative traits. %that can be used to model the evolution of a quantitative trait \citep[see][]{landis2013}
    
    \paragraph{GM Step for Shifts Locations for the OU} With $\alpha^{(h)}$ fixed, we want to minimize the sum of costs:
%        \[C^{OU}(\vvect{\tau}, \vvect{\delta}, \beta_0, \alpha^{(h)}) = \left(\Esp^{(h)}\left[\sachant{X_{1}}{\vect{Y}}\right] - \beta_0\right)^2 + \sum_{j=2}^{m+n}C_j^{OU}(\vvect{\tau}, \vvect{\delta}, \beta_0, \alpha^{(h)})\]
    \[C^{OU}(\alpha^{(h)}, \PB{\vect{\Delta}}) = \left(\Esp^{(h)}\left[\sachant{X_{1}}{\vect{Y}}\right] - \beta_0\right)^2 + \sum_{j=2}^{m+n}C_j^{OU}(\alpha^{(h)}, \PB{\vect{\Delta}})\]
    The previous algorithm does not work, because the costs are not independent. Solving the problem exactly would require to visit all the possible configurations, and the complexity would be too high, of order $O\left(\binom{m+n}{K}\right) = O(n^K)$. To reduce the execution time of the algorithm, we use heuristics to lower, if not minimize, the sum of costs. We use the following formulation:
%    \[
%     C^{OU}(\vvect{\tau}, \vvect{\delta}, \beta_0, \alpha^{(h)}) = \norm{\vect{F}^{(h)} - \matr{A}^{(h)}\matr{U}\vect{\Delta}}^2
%    \]
    \[
     C^{OU}(\alpha^{(h)}, \PB{\vect{\Delta}}) = \norm{\vect{F}^{(h)} - \matr{A}^{(h)}\matr{U}\vect{\Delta}}^2
    \]
    where 
    %$\vect{\Delta}$ is the vector of shifts described in subsection \ref{subsec:probabilistic_model}, 
    $\matr{U}$ the complete tree matrix given in subsection \ref{subsec:linear_model}, $\matr{A}^{(h)} = \Diag\left(1, \sqrt{\frac{1-e^{-\alpha^{(h)}\ell_j}}{1+e^{-\alpha^{(h)}\ell_j}}}; 2\leq j \leq m+n \right)$ a diagonal matrix depending on $\alpha^{(h)}$, and $\vect{F}^{(h)}$ a vector of expectations, with 
    $F^{(h)}_1 = \Esp^{(h)}\left[\sachant{X_{1}}{\vect{Y}}\right]$, and, for $2 \leq j \leq m+n$, \[F^{(h)}_j = \left(1-e^{-2\alpha^{(h)}\ell_j}\right)^{-1/2}\left(\Esp^{(h)}\left[\sachant{X_j}{\vect{Y}}\right] - \Esp^{(h)}\left[\sachant{X_{\pa(j)}}{\vect{Y}}\right]e^{-\alpha^{(h)}\ell_j}\right)\]
    We can then use a Lasso algorithm to impose sparsity constraints on $\vect{\Delta}$. If $\vect{\Delta}_{-1}$ is the vector of shifts without the initial value (intercept), then a Lasso estimator is given by, for $\lambda \geq 0$:
    \[
      \hat{\vect{\Delta}}_\lambda = \argmin_{\vect{\Delta}} \left\{ \norm{\vect{F}^{(h)} - \matr{A}^{(h)}\matr{U}\vect{\Delta}}^2 + \lambda \abs{\vect{\Delta}_{-1}}_1 \right\}
    \]
    The estimated vectors $\hat{\vect{\Delta}}_\lambda$ have a support that is sparser when $\lambda$ becomes higher. One then only need to find the right penalty factor $\lambda$ that ensure that the support has exactly $K$ non zero coordinates, plus the initial value. %The Lasso regression is done here thanks to an algorithm implemented in the \printR{R} package \printR{quadrupen} \citep{chiquet2012}.
We ensure that the $K$ shifts are allocated in a parsimonious way by checking their linear independence, using proposition \ref{prop:parsimony_linear_independence}.\par
    An other method is to take the previous solution $\vect{\Delta}^{(h)}$, and test all the configurations where only one shift has moved, and take the best one. In both methods, one also has to ensure that the objective function is increased by the new choice of shifts, so that the GEM algorithm works correctly. This step is generally the longest one in one iteration of the EM.

%%%%%%%%%%%%%%%%%%%%%%%%%%%%%%%%%%%%%%%%%%%%%%%%%%%%%%%%%%%%%%%%%%%%%%%
\subsection{Initialization}\label{supp:initialization}
Initialization is always a crucial step when using an EM algorithm. The vector of shifts $\vect{\Delta}$ is initialized thanks to a Lasso procedure. To do that, we use the linear formulation \ref{eq:BM_lin_def_X} or \ref{eq:OU_lin_def} of the main text, and we calibrate the penalty so that the initialization vector has a non zero first coordinate (initial value), and $K$ other non-zero coordinates. The variance-covariance matrix is initialized with defaults parameters, and is taken into account thanks to a Cholesky decomposition.\par
    We also initialize the selection strength $\alpha$. We use the following property: if $Y_i$ and $Y_j$ are two tips in the same group, then, under an OUsun, \( \Espe{(Y_i-Y_j)^2} = 2\gamma^2(1-e^{-\alpha d_{ij}}) \). Using regression techniques, we can get an initial estimation of $\alpha$ and $\gamma^2$ from all these couples. In practice, we first initialize the position of the shifts, and then use only pairs of tips from the same estimated group. Then, as the groups are only approximated, some of the selected pairs $(Y_i, Y_j)$ might not share the same expectation, and we use a robust regression to get more accurate initial estimates.
\newpage
\section{Proof of Proposition~\ref{prop:model_selection} for Model Selection} \label{supp:proof_model_selection}

\PB{We prove the proposition using the linear formulation $\vect{s} + \gamma \vect{E}$, with $\vect{E} \sim \Normal(0, \matr{V})$, as derived in the main text for the OUsun (with $\vect{s} = \matr{T}\matr{W}(\alpha)\vect{\Delta}$, $\gamma^2 = \sigma^2/(2\alpha)$, and $V_{ij} = e^{-\alpha d_{ij}}$, see Formula~(\ref{eq:OU_lin_def_X})). Note that this framework also holds for the BM with a fixed root (with $\vect{s} = \matr{T}\vect{\Delta}$, $\gamma = \sigma$, and $V_{ij} = t_{ij}$, see Formula~(\ref{eq:BM_lin_def_X})).}

We first handle the case where there are no correlations (\PB{$\matr{V}$ diagonal}), and then use a Cholesky decomposition to handle the general case. \PB{Note that the case $\matr{V}$ diagonal can be seen as the limit of the OUsun when $\alpha = +\infty$, or as a BM on a star tree.}
    
    \emph{Case \PB{$\matr{V}$ diagonal}}
    
    In the iid case, we just need to check the conditions of theorem~\ref{th:model_selection_baraud2009}. This paragraph is highly inspired by the derivation of the bound for the detection of non-zero mean components exposed in \citet{baraud2009} (sub-section 5.2). Assume that $D_\eta = K_\eta + 1 \leq p \leq n-7$ for all $\eta\in\Mr$. The estimator is defined by $\vect{\hat{s}}_{\hat{K}}$, with:
    \[
    \hat{K} = \argmin_{0\leq K \leq p-1} \mahanorm{\vect{Y} - \vect{\hat{s}}_K}{V}^2 \left( 1 + \frac{\pen_{A, \Lr}(K)}{n-K-1}\right)
    \]
    From the definition of $\vect{\hat{s}}_K$, and as the penalty depends on the model only through its number of shifts, we get that $\vect{\hat{s}}_{\hat{K}} = \vect{\hat{s}}_{\hat{\eta}}$ the minimizer of the criterion of theorem~\ref{th:model_selection_baraud2009} (with $N_\eta = n-D_\eta = n - K_\eta - 1$).
    We then have:
    \[
     \Omega' =  \sum_{\eta \in \Mr} (D_\eta + 1) e^{-L_\eta}= \sum_{K = 0}^{p-1} \card{\Sr_{K}^{PI}} (K + 2) e^{-L_K}
    \]
     With the weights $L_K$ defined in equation~\ref{eq:L_K} of the proposition, we get:
    \[
     \Omega' =  \sum_{K = 0}^{p-1} \frac{1}{K+2} \leq \log(p) \leq \log(n)
    \]
    As:
     \begin{align*}
      L_K \leq \log \binom{n+m-1}{K} + 2\log(K+2) &\leq K\log(n+m-1) + 2\log(K+2)\\
      & \leq K\log(2n-2) + 2(K+1)\\
      & \leq (K+1)(2 + \log(2) + \log(n))\\
      & \leq p(2 + \log(2) + \log(n))
     \end{align*}
      if
      \(p \leq \min\left(\frac{\kappa n}{2 + \log(2) + \log(n)}, n-7\right)\), then  $\max(L_\eta, D_\eta) \leq \kappa n$ for any $\eta\in\Mr$, and we get the announced bound from the second proposition of theorem~\ref{th:model_selection_baraud2009}.
      
      \emph{Case \PB{$\matr{V}$ not diagonal}}
      
      Using a Cholesky decomposition, we can find a lower triangular matrix $\matr{L}$ such that $\matr{V} = \matr{L}\matr{L}^T$. Then, denoting $\vect{Y}' = \matr{L}^{-1}\vect{Y}$, $\vect{s}'=\matr{L}^{-1}\vect{s}$, and $\vect{E}' = \matr{L}^{-1}\vect{E}$, we have \(\vect{Y}' = \vect{s}' + \gamma \vect{E}'\), with $\vect{E}'\sim\Normal(0, \matr{I_n})$, and we can apply theorem~\ref{th:model_selection_baraud2009} as above. As we changed the metric, the estimators are projections on the linear spaces $S'_\eta=\matr{L}^{-1}S_\eta$ for $\eta \in \Mr$, and we have:
      \begin{align*}
      \vect{\hat{s}}'_\eta &= \Proj_{S'_\eta}\vect{Y}' = \argmin_{\vect{a}' \in S'_\eta} \norm{\vect{Y}'-\vect{a}'}^2 = \argmin_{\vect{a}' \in S'_\eta} \norm{\matr{L}^{-1}\vect{Y}-\matr{L}^{-1}\matr{L}\vect{a}'}^2\\
      &= \argmin_{\vect{a}' \in S'_\eta} \mahanorm{\vect{Y} - \matr{L}\vect{a}'}{V}^2 = \matr{L}^{-1}\argmin_{\vect{a} \in S_\eta} \mahanorm{\vect{Y} - \vect{a}}{V}^2 = \matr{L}^{-1}\vect{\hat{s}}_\eta
      \end{align*}
      So $\mahanorm{\vect{s} - \vect{\hat{s}}_{\hat{\eta}}}{V}^2 = \norm{\vect{s}' - \vect{\hat{s}}'_{\hat{\eta}}}^2$ and $\mahanorm{\vect{Y} - \vect{\hat{s}}_\eta}{V}^2 = \norm{\vect{Y}' - \vect{\hat{s}}'_\eta}^2$, and, as the form of the penalty does not depend on $V$, by minimizing:
      \[
      \Crit_{LS}(K) = \norm{\vect{Y}' - \vect{\hat{s}}'_K}^2 \left( 1 + \frac{\pen_{A, \Lr}(K)}{n - K - 1}\right) = \mahanorm{\vect{Y} - \vect{\hat{s}}_K}{V}^2 \left( 1 + \frac{\pen_{A, \Lr}(K)}{n - K -1}\right)
      \]
      we get the announced bound on $\Espe{\frac{\mahanorm{\vect{s} - \vect{\hat{s}}_{\hat{K}}}{V}^2}{\gamma^2}} = \Espe{\frac{\norm{\vect{s}' - \vect{\hat{s}}'_{\hat{K}}}^2}{\gamma^2}}$.
\newpage
%%%%%%%%%%%%%%%%%%%%%%%%%%%%%%%%%%%%%%%%%%%%%%%%%%%%%%%%%%%%%%%%%%%%%%%
%%%%%%%%%%%%%%%%%%%%%%%%%%%%%%%%%%%%%%%%%%%%%%%%%%%%%%%%%%%%%%%%%%%%%%%
\section{Supplementary Figures} \label{supp:SimulationAnalysis}
%%%%%%%%%%%%%%%%%%%%%%%%%%%%%%%%%%%%%%%%%%%%%%%%%%%%%%%%%%%%%%%%%%%%%%%
%%%%%%%%%%%%%%%%%%%%%%%%%%%%%%%%%%%%%%%%%%%%%%%%%%%%%%%%%%%%%%%%%%%%%%%

%%%%%%%%%%%%%%%%%%%%%%%%%%%%%%%%%%%%%%%%%%%%%%%%%%%%%%%%%%%%%%%%%%%%%%%
%%% Definition of Knitr
%%%%%%%%%%%%%%%%%%%%%%%%%%%%%%%%%%%%%%%%%%%%%%%%%%%%%%%%%%%%%%%%%%%%%%%

%%%%%%%%%%%%%%%%%%%%%%%%%%%%%%%%%%%%%%%%%%%%%%%%%%%%%%%%%%%%%%%%%%%%%%%

  %%%%%%%%%%%%%%%%%%%%%%%%%%%%%%%%%%%%%
  \subsection{Simulation Study: Sensitivity and False Positive Rate}
    \paragraph{Definition of the Scores}
    We denote by $TP$ the number of True Positives, i.e. the predicted edges on which a shift actually occurred, and $FP$ the number of False Positives.
    The sensitivity $\frac{TP}{K_t}$ is the proportion of well predicted shifts among all shifts to be predicted, and the False Positive Rate (FPR) $\frac{FP}{n + m - K_t}$ is the proportion of false positive among all edges with no shifts.\par
    Note that here, due to the possible lack of identifiability, the position of the shifts on the tree is not well defined, as a shift can be on a particular edge for one of the equivalent solutions, but not on the others (see Section \ref{subsec:identifiability}). These two scores are hence ill defined for our problem. To avoid such problems, we restrict ourselves to the $91\%$ of unambiguous configurations \PB{that occurred during the simulations}.
    %Here, $TP$ denotes the True Positives (predicted edges on which a shift actually occurred) and $FP$, $TN$, $FN$, respectively, the False Positive, True Negative, False Negative. We have $TP + FN = K_t$ the true number of shifts, and $FP + TN = n + m - 1 - K_t$ the number of edges without any shift. Similarly, $TP + FP = K_s$ the selected number of shifts, and $FN + TN = n+m-1-K_s$ the number of edges without predicted shifts.
%     \begin{itemize}
%     \item The sensitivity : $\frac{TP}{K_t}$ (proportion of well predicted shifts among all shifts to be predicted)
%     \item The False Positive Rate (FPR) : $\frac{FP}{n + m - K_t}$ (proportion of false positive among all edges with no shifts). %FPR = 1 - specificity.
%     \end{itemize}

\paragraph{Interpretation of Results}
 Figure \ref{simus:fpr} shows that the FPR are systematically worse when using the true number of shifts, indicating that the additional shifts found when compared to the selected number are misplaced. The FPR remains very low, as only a small number of shifts is to be found. Unsurprisingly, the Sensitivity is on the contrary improved when taking the real number of shifts, as shown Figure \ref{simus:sensitivity}. In addition, the sensitivity is highly degraded when $\alpha$ is small or $\gamma^2$ is high, but does not exhibit a clear tendency in the real number of shifts, and the knowledge of the true value of $\alpha$ does not seem to matter.
    
    \begin{figure}[hp]
    \begin{center}
\begin{knitrout}
\definecolor{shadecolor}{rgb}{0.969, 0.969, 0.969}\color{fgcolor}
\includegraphics[width=\maxwidth,height=0.4\textheight]{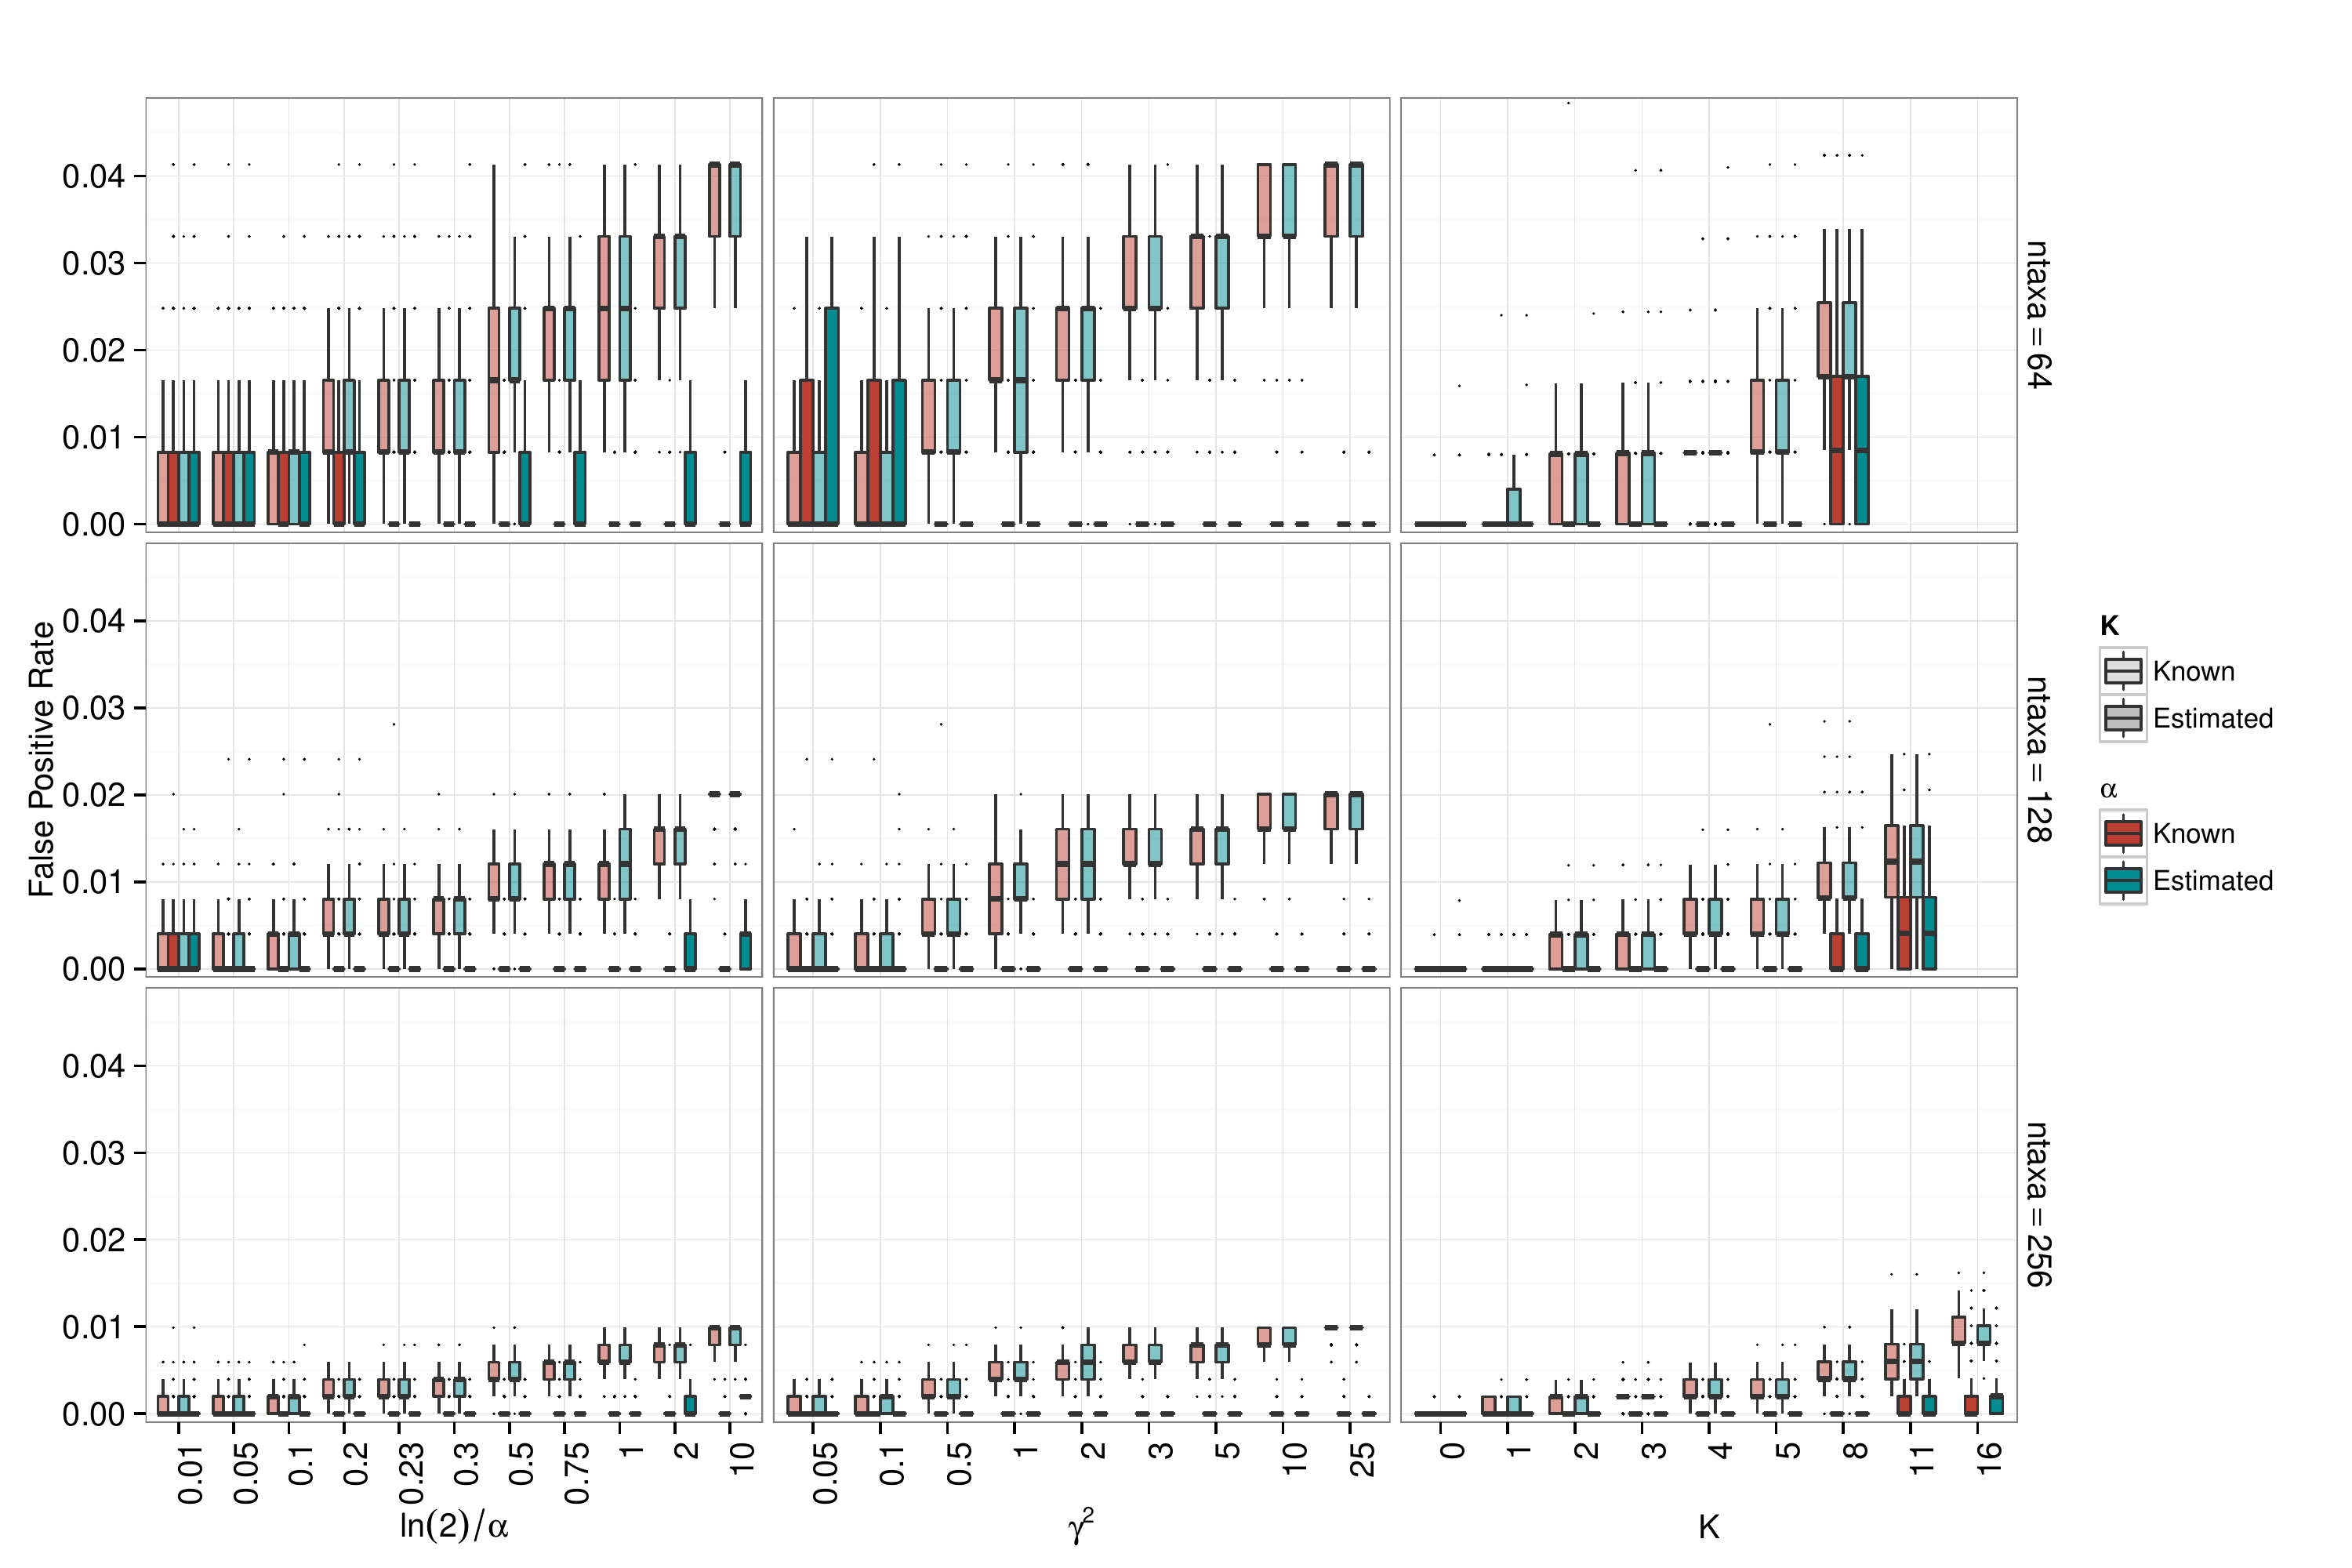} 

\end{knitrout}
    \caption{False Positive Rate computed for the different configurations. Note the $y$ scale, that only goes to $0.05$.}\label{simus:fpr}
    \end{center}

    \begin{center}
\begin{knitrout}
\definecolor{shadecolor}{rgb}{0.969, 0.969, 0.969}\color{fgcolor}
\includegraphics[width=\maxwidth,height=0.4\textheight]{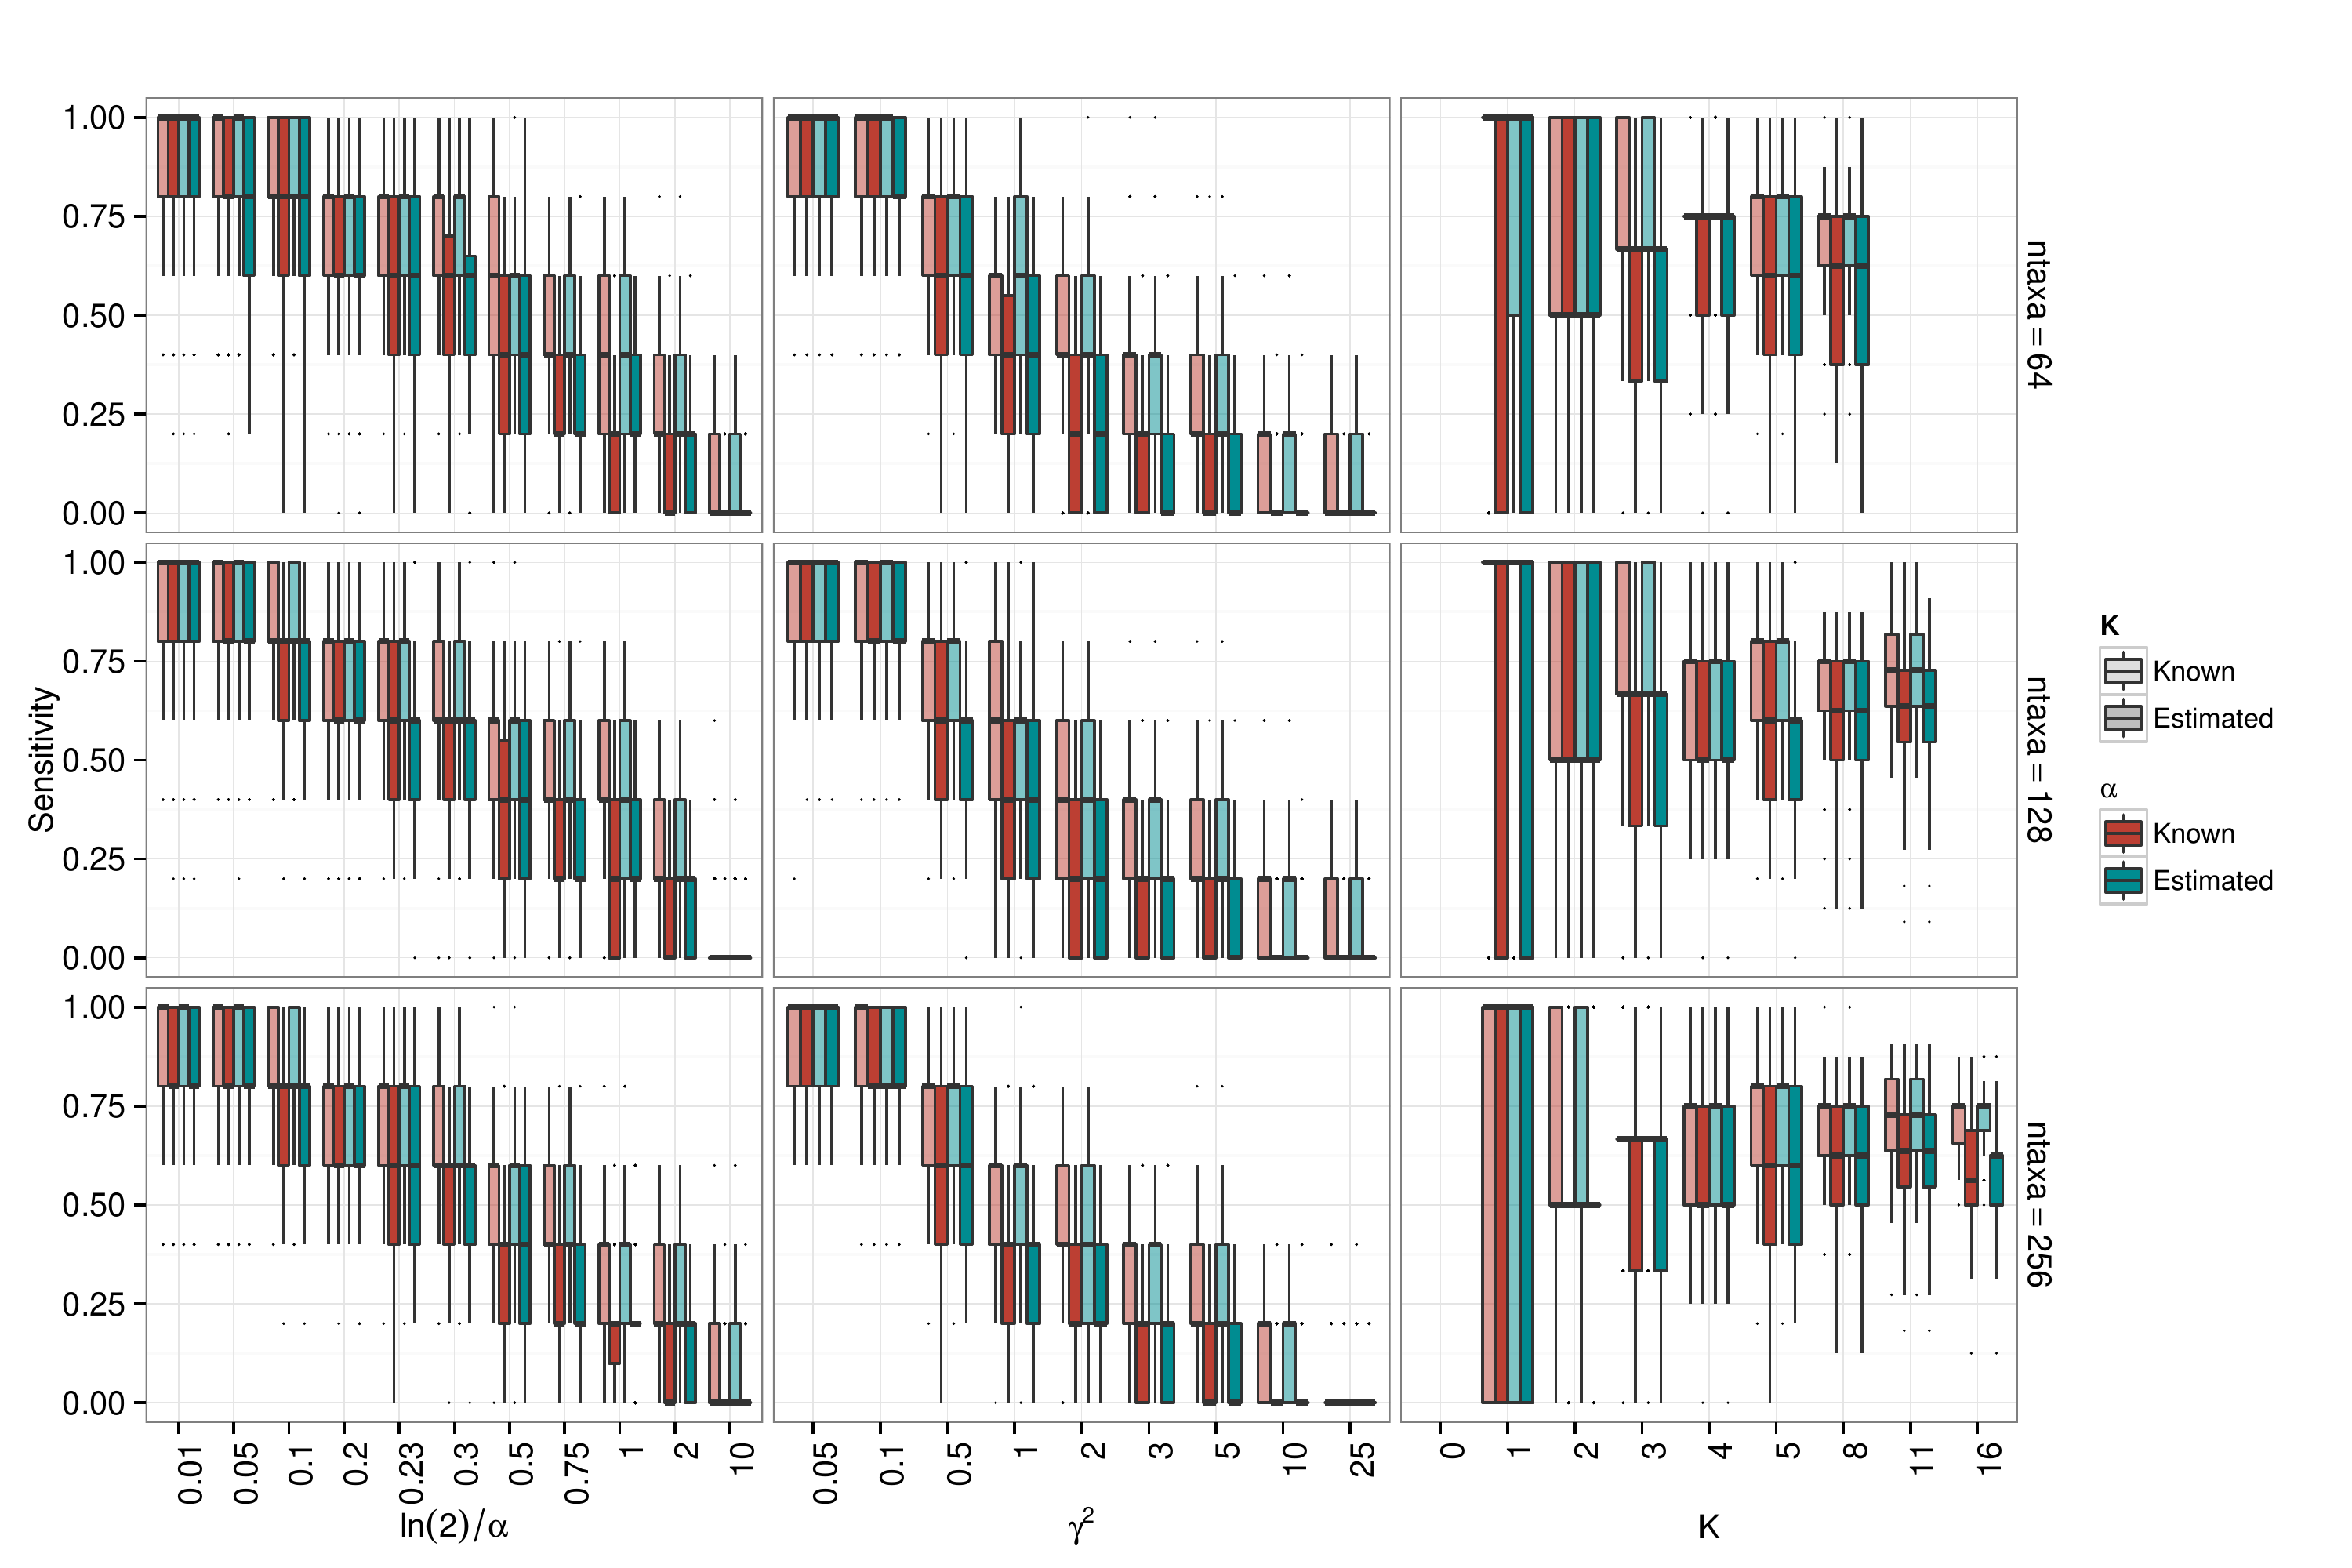} 

\end{knitrout}
    \caption{Sensitivity computed for the different configurations, with box-plots over the repetitions. 
    %The line represents a smoothing thanks to a local polynomial regression fitting.
    }\label{simus:sensitivity}
    \end{center}
    \end{figure}
    
%%%%%%%%%%%%%%%%%%%%%%%%%%%%%%%%%%%%%%%%%%%%%%%%%%%%%%%%%%%%%%%%%%%%%%%%%%%%%%%%%%
 \subsection{Simulation Study: Complementary Analysis}
 To complete the analysis conducted in the main text, 
 %we present here the \comment{complementary} plots of Figures~\ref{fig:ll_t_gamma} and~\ref{fig:beta_K_ARI}. Here, 
 Figure~\ref{fig:ll_t_gamma_rev} presents the variations of the log-likelihood, phylogenetic half-life, and root variance when $\alpha$ is estimated, and the number of shifts is known or estimated. We can see here that the likelihood is slightly higher when the number of shifts is fixed, which is coherent with the behavior of our model selection procedure, that tends to under-estimate the true number of shifts (see Figure~\ref{fig:beta_K_ARI} of the main text). We also note that knowing the true number of shifts has not a great influence on the estimation of $\alpha$ and $\gamma$, making the later worse, if anything.\par
 
 Figure~\ref{fig:beta_K_ARI_rev} shows the variations of the estimations of $\beta_1$, the number of shifts and the ARI when the number of shifts is estimated, and $\alpha$ is fixed or estimated. This confirms our earlier statement, that not knowing $\alpha$ with precision does not have a great impact on the model selection procedure \citep[see also][]{cressler2015}.
 
 \begin{figure}[hp]
\begin{center}

\includegraphics[width=\linewidth]{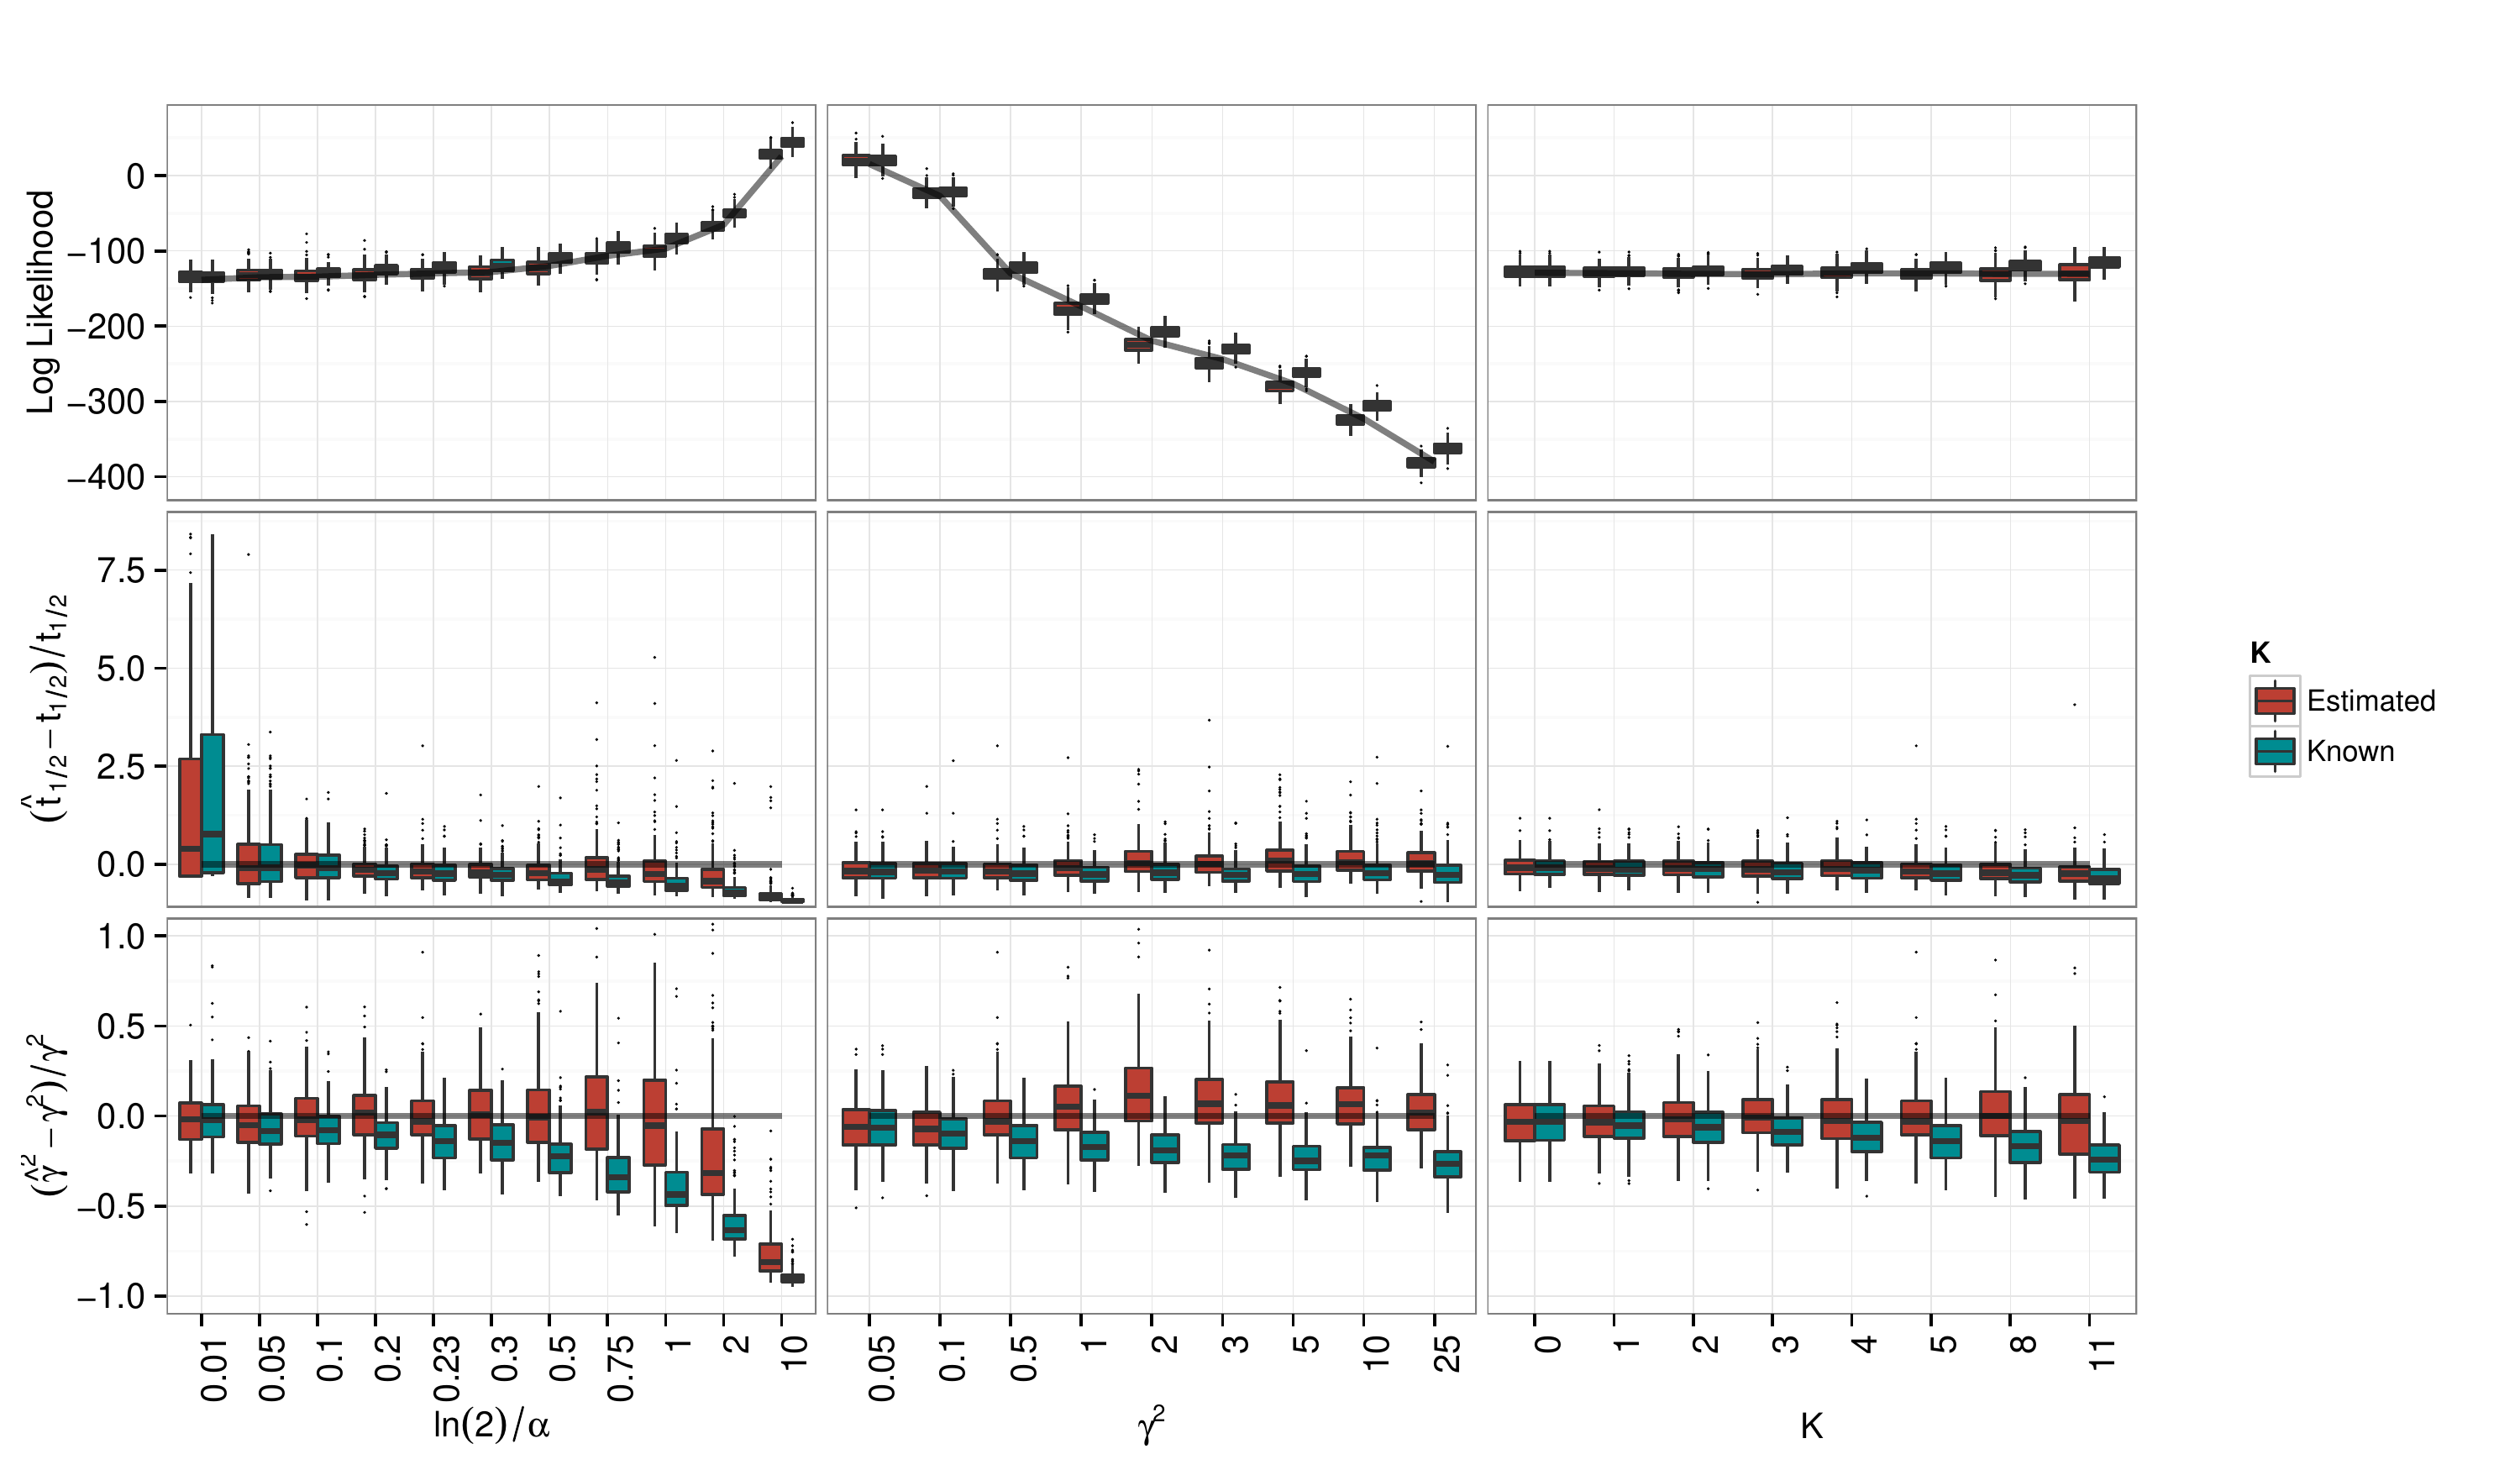} 

\caption{Box plots over the $200$ repetitions of each set of parameters, for the log-likelihood (top), phylogenetic half-life (middle) and root variance (bottom) with $\alpha$ estimated, and $K$ fixed or estimated, on a tree with $128$ taxa.}\label{fig:ll_t_gamma_rev}
\end{center}

\begin{center}

\includegraphics[width=\linewidth]{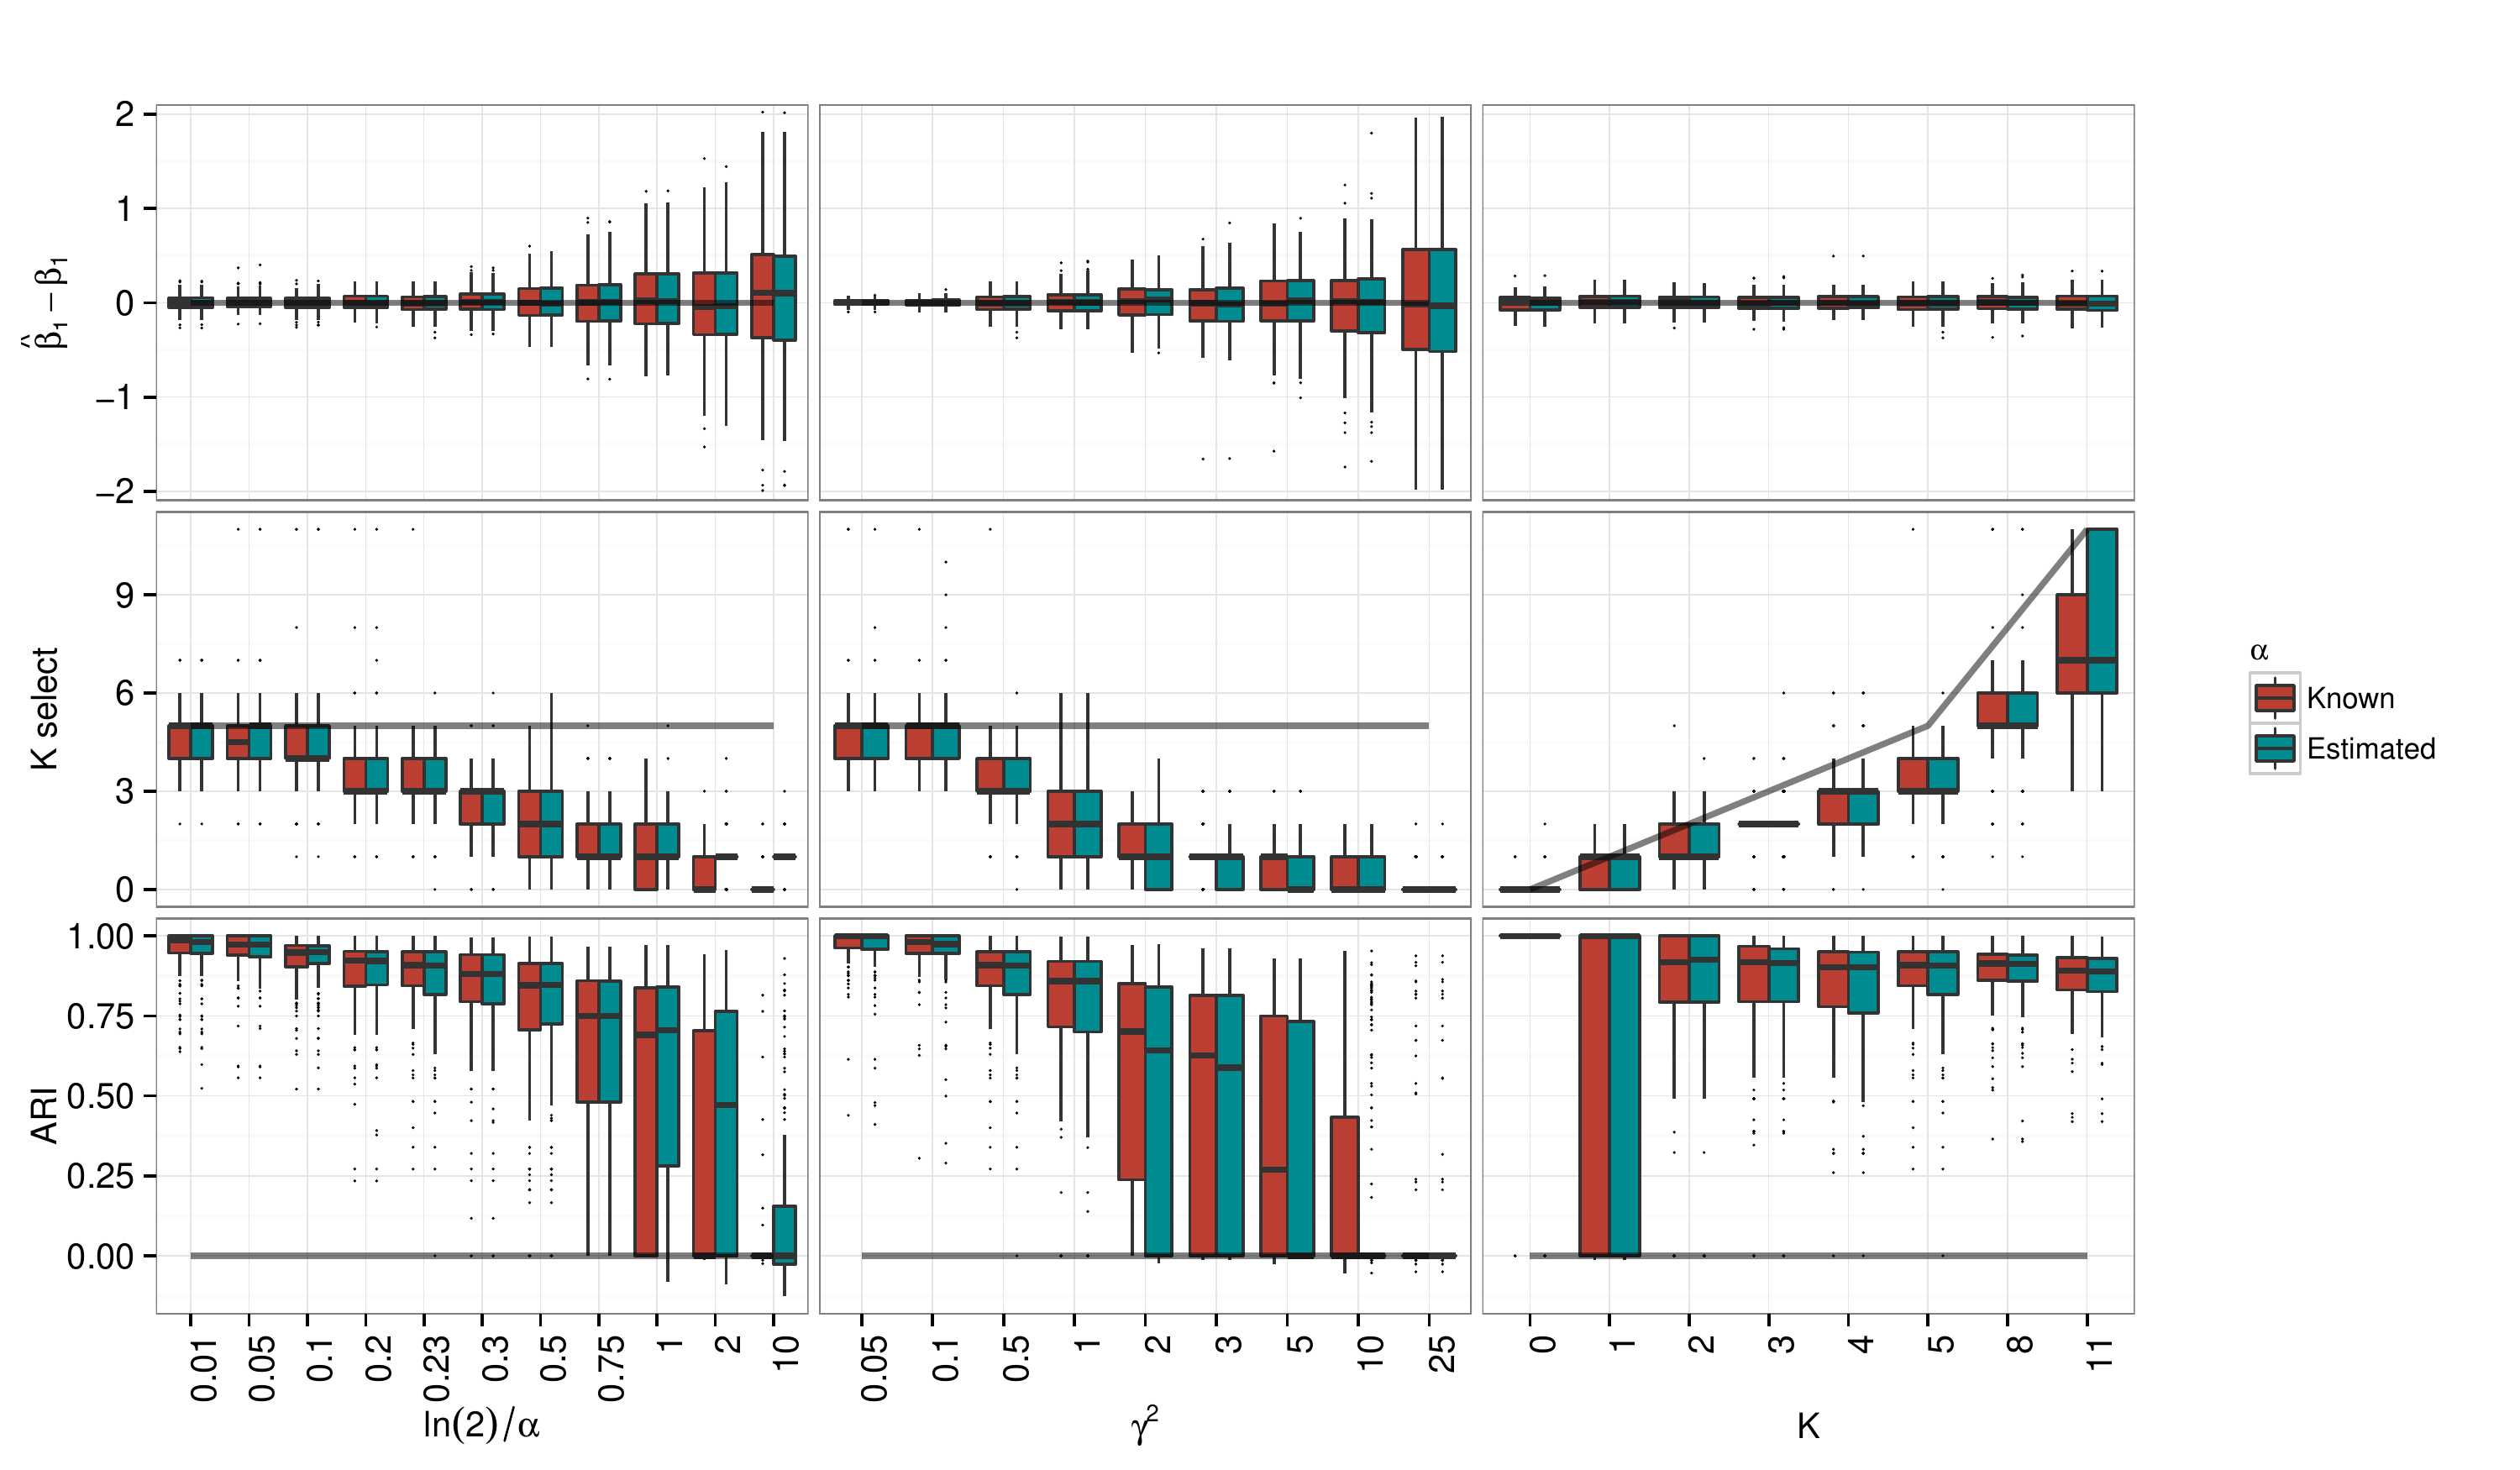} 

\caption{Same for $\beta_1$ (top), the number of shifts (middle) and ARI (bottom), with $K$ estimated, and $\alpha$ fixed or estimated.}
%Box plots for $\beta_1$ (top), the number of shifts (middle) and ARI (bottom) with the number of shifts fixed or estimated, on a tree with $128$ taxa.}
\label{fig:beta_K_ARI_rev}
\end{center}
\begin{flushleft}
For better legibility, strips with $t_{1/2}$, $\gamma^2$ and $\beta_1$ on these two figures were re-scaled, omitting some outliers (respectively, $0.21\%$, $0.27\%$ and $0.27\%$ of points are omitted). The whisker of the first box for $t_{1/2}$ goes up to $7.5$.
\end{flushleft}
\end{figure}
 
 %%%%%%%%%%%%%%%%%%%%%%%%%%%%%%%%%%%%%%%%%%%%%%%%%%%%%%%%%%%%%%%%%%%%%%%%%%%%%%%%%
 \subsection{Chelonia Dataset: Comparison of Inferred Shift Locations}\label{supp:chelonia}

  On Figure~\ref{fig:chelonia_sol_bayou}, we present and compare the shift locations found by our method, and methods \printR{bayou} and \printR{SURFACE}. The differences found are explored deeper in the main text (Section~\ref{sec:chelonia_comparison}).
 
 \paragraph{Details on the methods} In this paragraph, we give more details on the $4$ already existing methods that we compared to ours in the dataset.
 We first fitted an OU$_{habitat}$ model with fixed regimes as in \citet{jaffe2011}, using the \printR{R} package \printR{OUwie} \citep{beaulieu2012}. We tested all of the $48$ possible ways of allocating internal nodes, and took the solution with the highest likelihood. Using the package \printR{bayou} \citep{uyeda2014}, we reproduced the Bayesian analysis of the data, using two independent chains of $500000$ generations each, discarding the first $150000$ generations as burning. We assigned the priors that were used in the original study on the parameters, namely: $P(\alpha) \sim \text{LogNormal}(\ln \mu = -5, \ln \sigma = 2.5)$, $P(\sigma^2)\sim \text{LogNormal}(\ln \mu = 0, \ln \sigma = 2)$, $P(\beta_i)\sim \text{Normal}(\mu = 3.5, \sigma = 1.5)$, $P(K)\sim \text{Conditional Poisson}(\lambda = 15, K_{max} = 113)$. The computations took around $2.3$ hours of CPU time.
  \PB{We also} ran the stepwise-AIC method \citeR{SURFACE}, that relies on a forward-backward procedure. This took around $11$ hours of CPU time.
  \PB{Finally, we ran the function \printR{OUshifts} from the package \printR{phylolm}, that uses a modified BIC criterion and a heuristic stepwise procedure to detect shifts \citep{hoane2014}. Thanks to an efficient linear algorithm, detailed in \citet{hoane2013b}, this function is pretty fast, taking only about $8$ minutes of CPU time.}
  Note that the model used in these last \PB{three} methods (\printR{bayou}, \printR{SURFACE} and \printR{OUshifts}) are slightly different from ours, as they assume that the root is fixed to the ancestral optimum state, 
%  and not \PB{randomly drawn} in the stationary state.\par
\PB{and not drawn from its stationary distribution.} \par
 
   \paragraph{Note on Computation Times}
   We found that the running time for our method was similar to the running time of previous algorithms (see Table~\ref{table:chelonia} in the main text). However, our computations can be highly parallelized, as each run for a fixed number of shift is independent from the others.
  %Using \printR{R} packages \citeR{foreach} and \citeR{doParallel}, this can be easily done.
  For instance, in the previous example, the computation time could be divided by $6$, each estimation for a fixed $\alpha$ running on a different core. On the contrary, the \printR{SURFACE} method cannot be parallelized at all, and only independent chains can be parallelized for Bayesian methods, so that the computation time can only be divided by $2$ in our example.
  
 \begin{figure}[!hp]
    \begin{center} 
        \begin{minipage}{0.45\textwidth}

\includegraphics[width=\maxwidth,height=0.45\textheight]{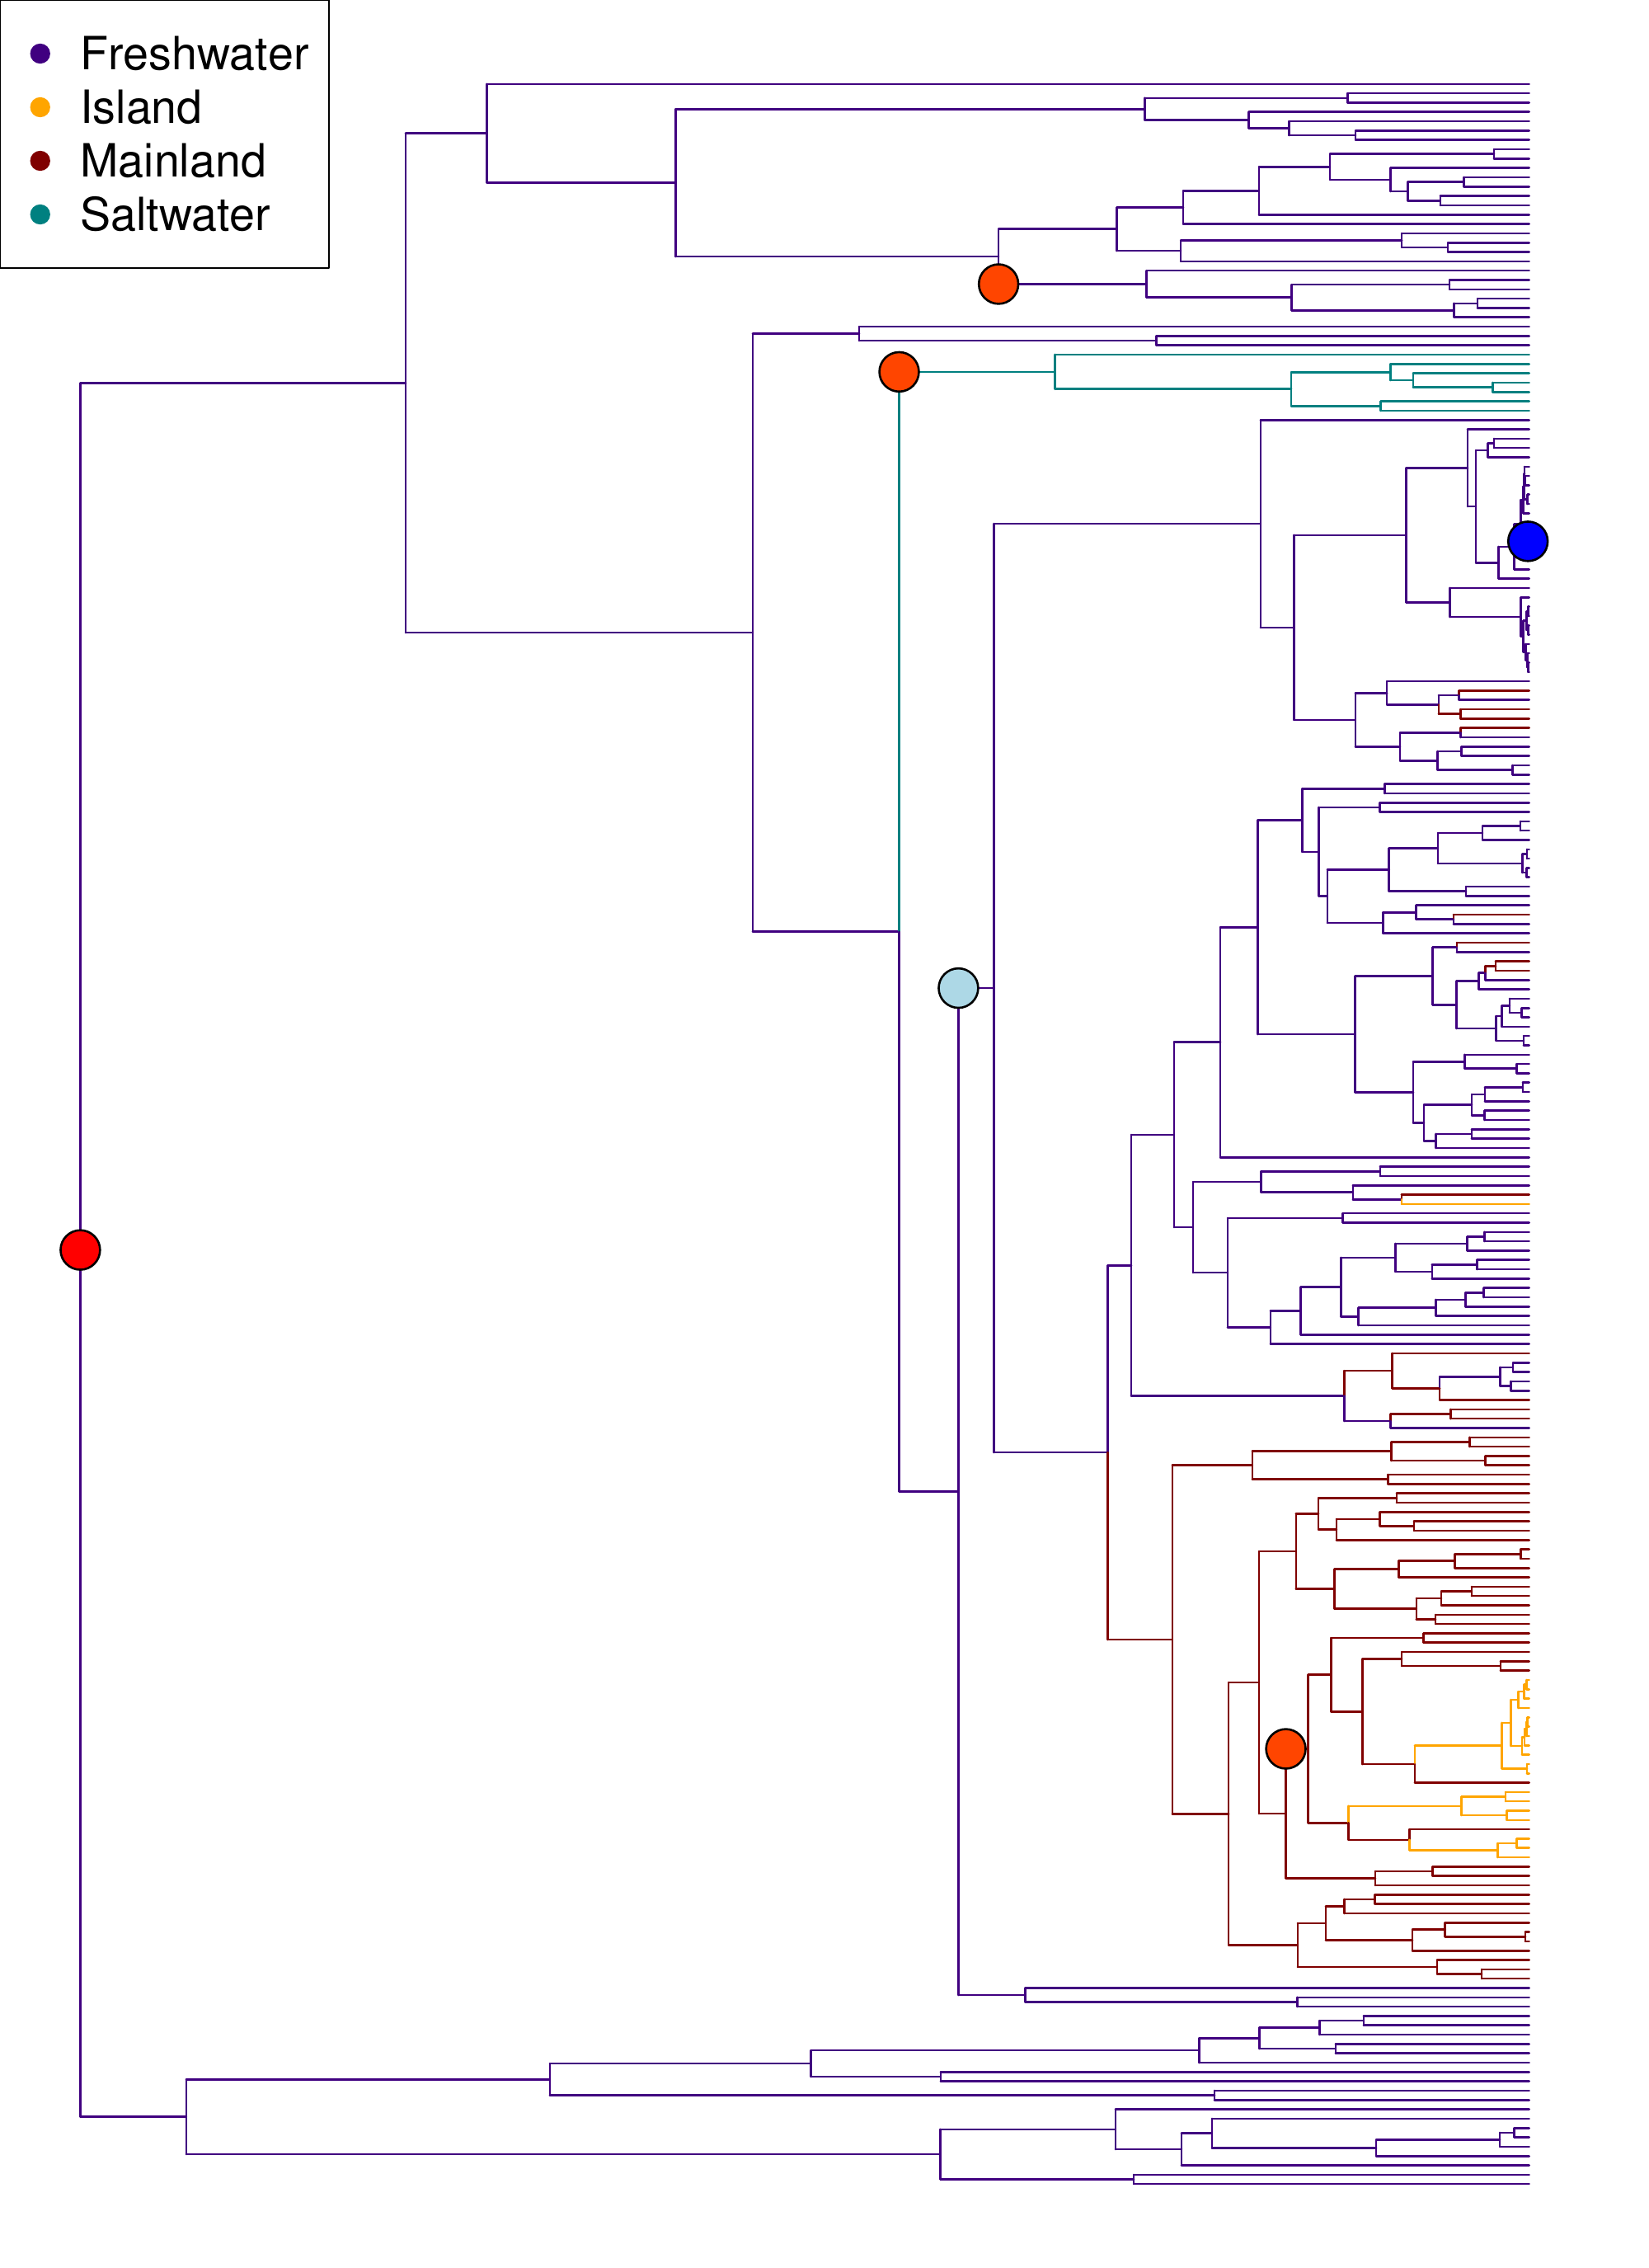} 

     {\sf \vskip -0.5cm \qquad EM}
    \end{minipage}
% \vskip - 0.5 cm
    \begin{minipage}{0.45\textwidth}

\includegraphics[width=\maxwidth,height=0.45\textheight]{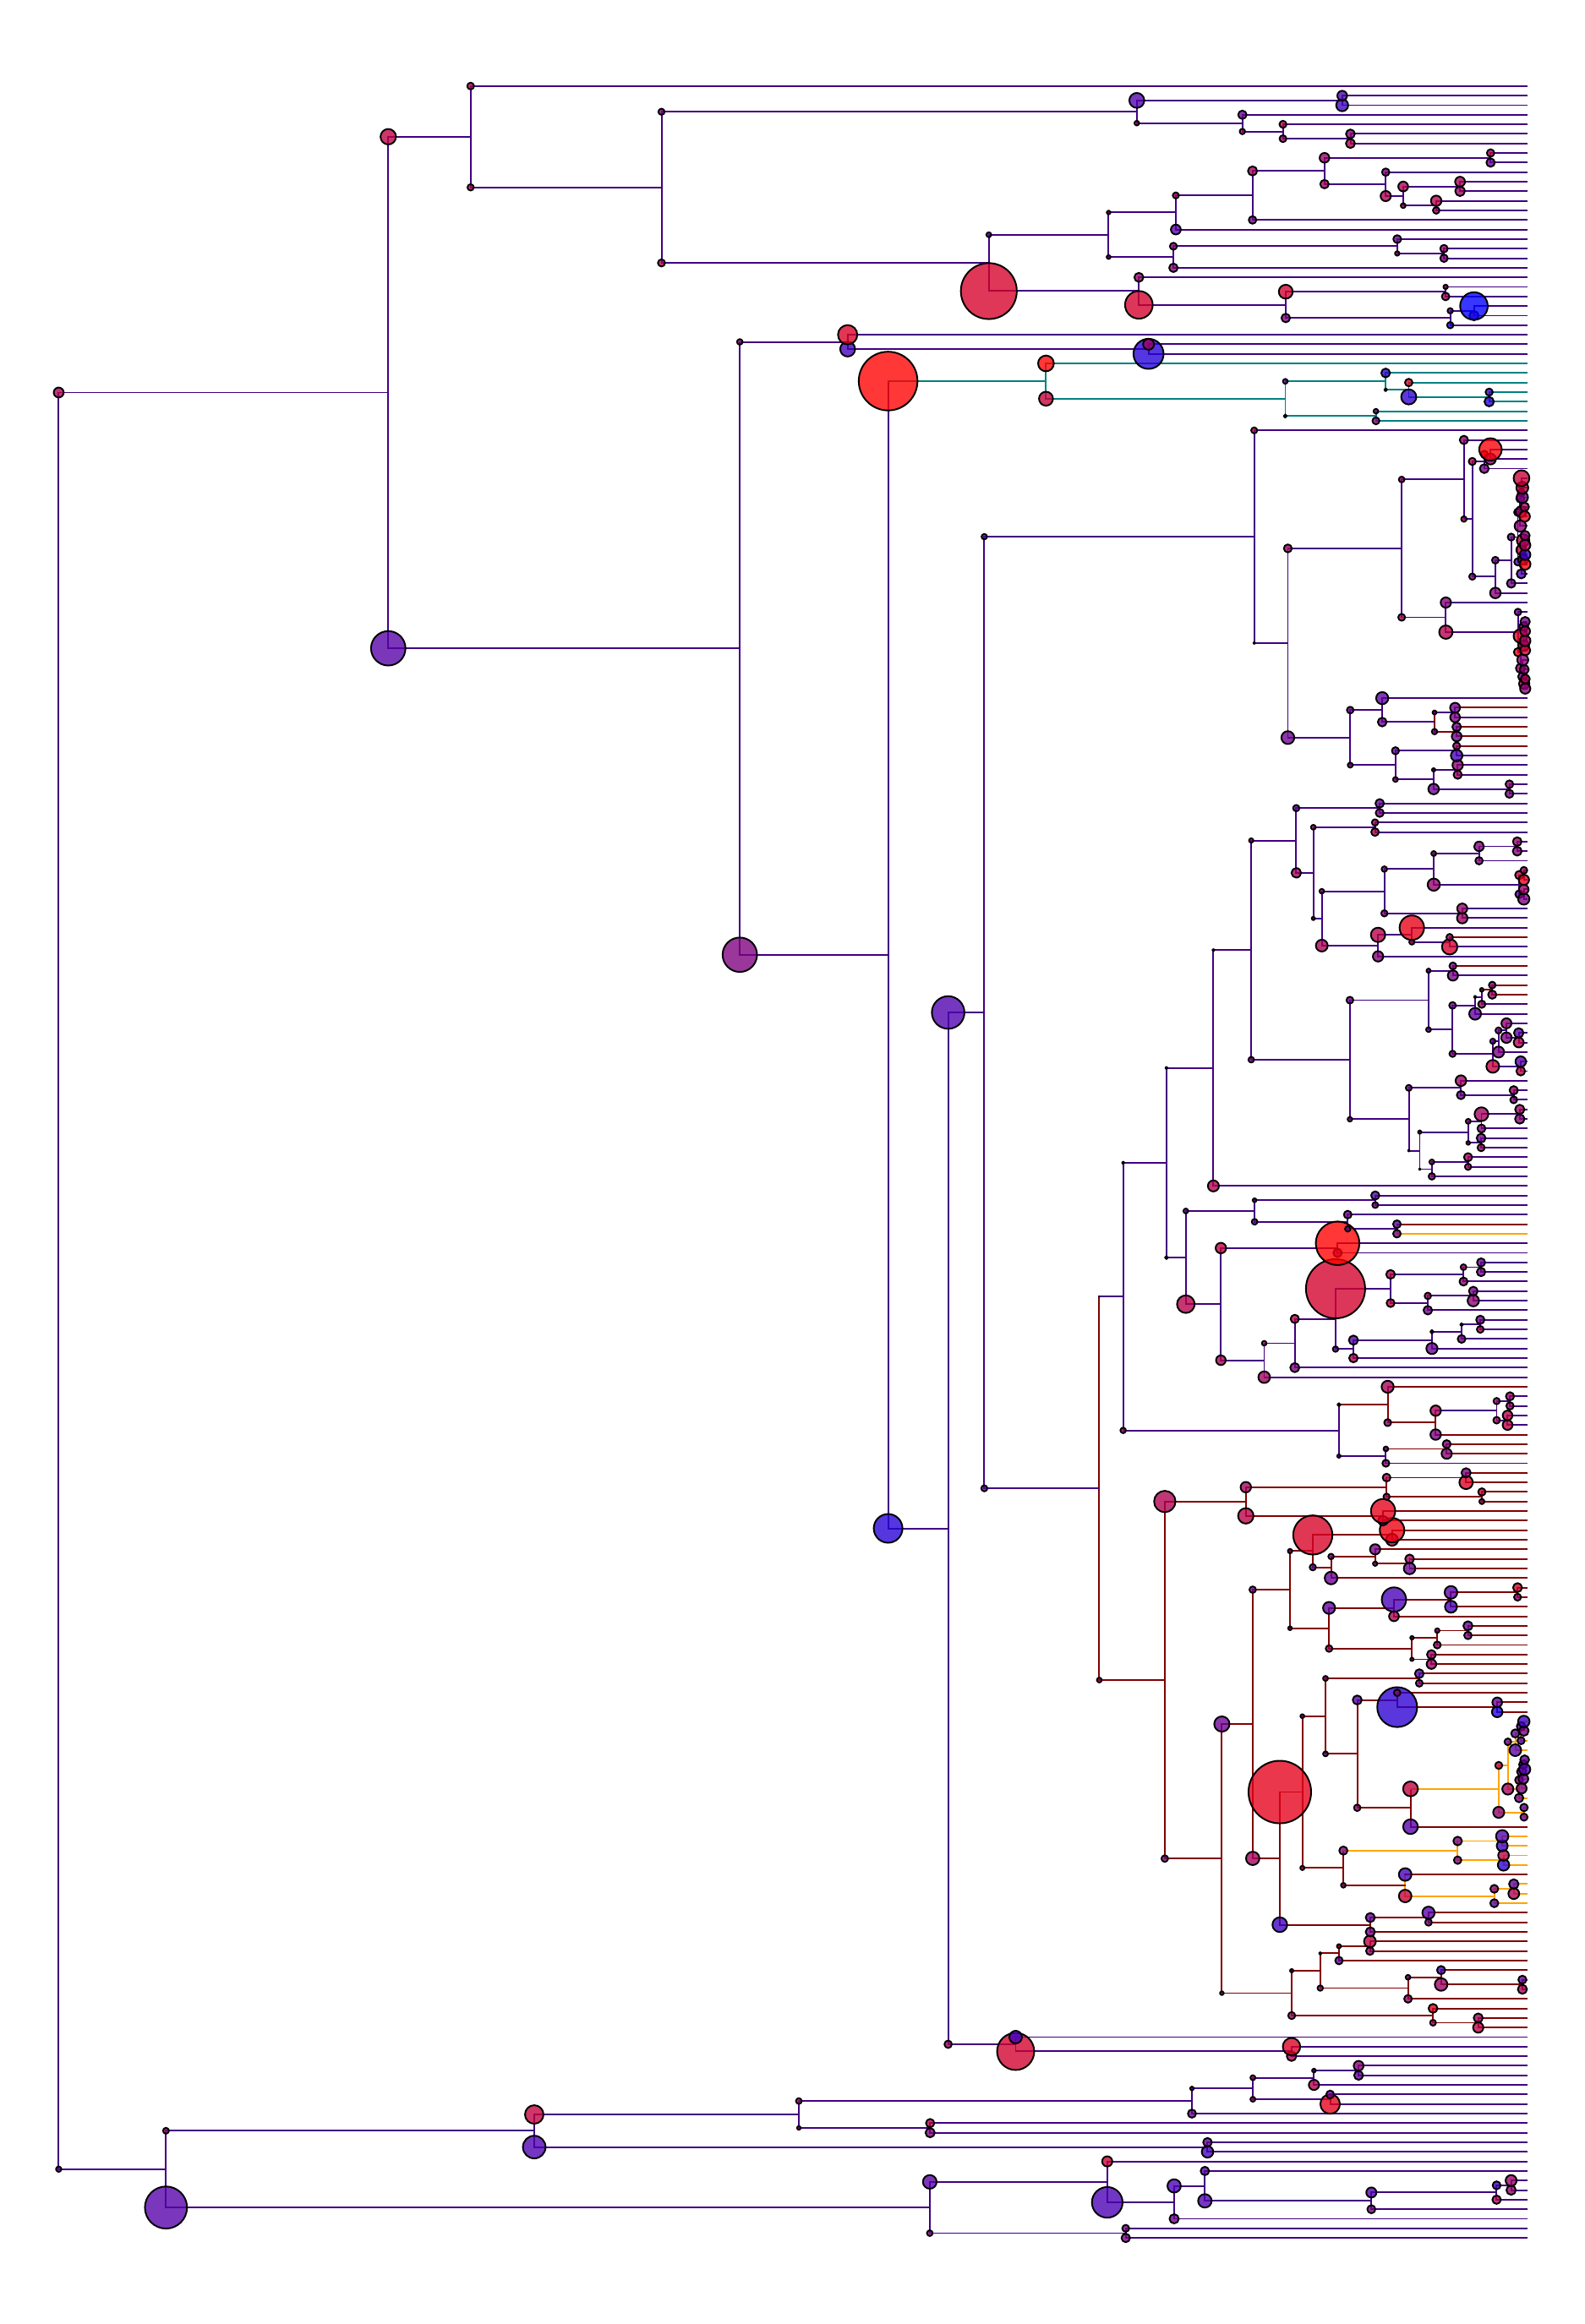} 

     {\sf \vskip -0.5cm \qquad bayou}
    %\caption{Result of the methods \printR{bayou} (circles at nodes) and \printR{SURFACE} (branch coloring). The size of the circles are proportional to their posterior probability, and their colors represents their values, from blue (negative) to red (positive). The $13$ colors on the edges represent the regimes found after convergence.}\label{fig:chelonia_sol_bayou}
\end{minipage}

    \begin{minipage}{0.45\textwidth}

\includegraphics[width=\maxwidth,height=0.45\textheight]{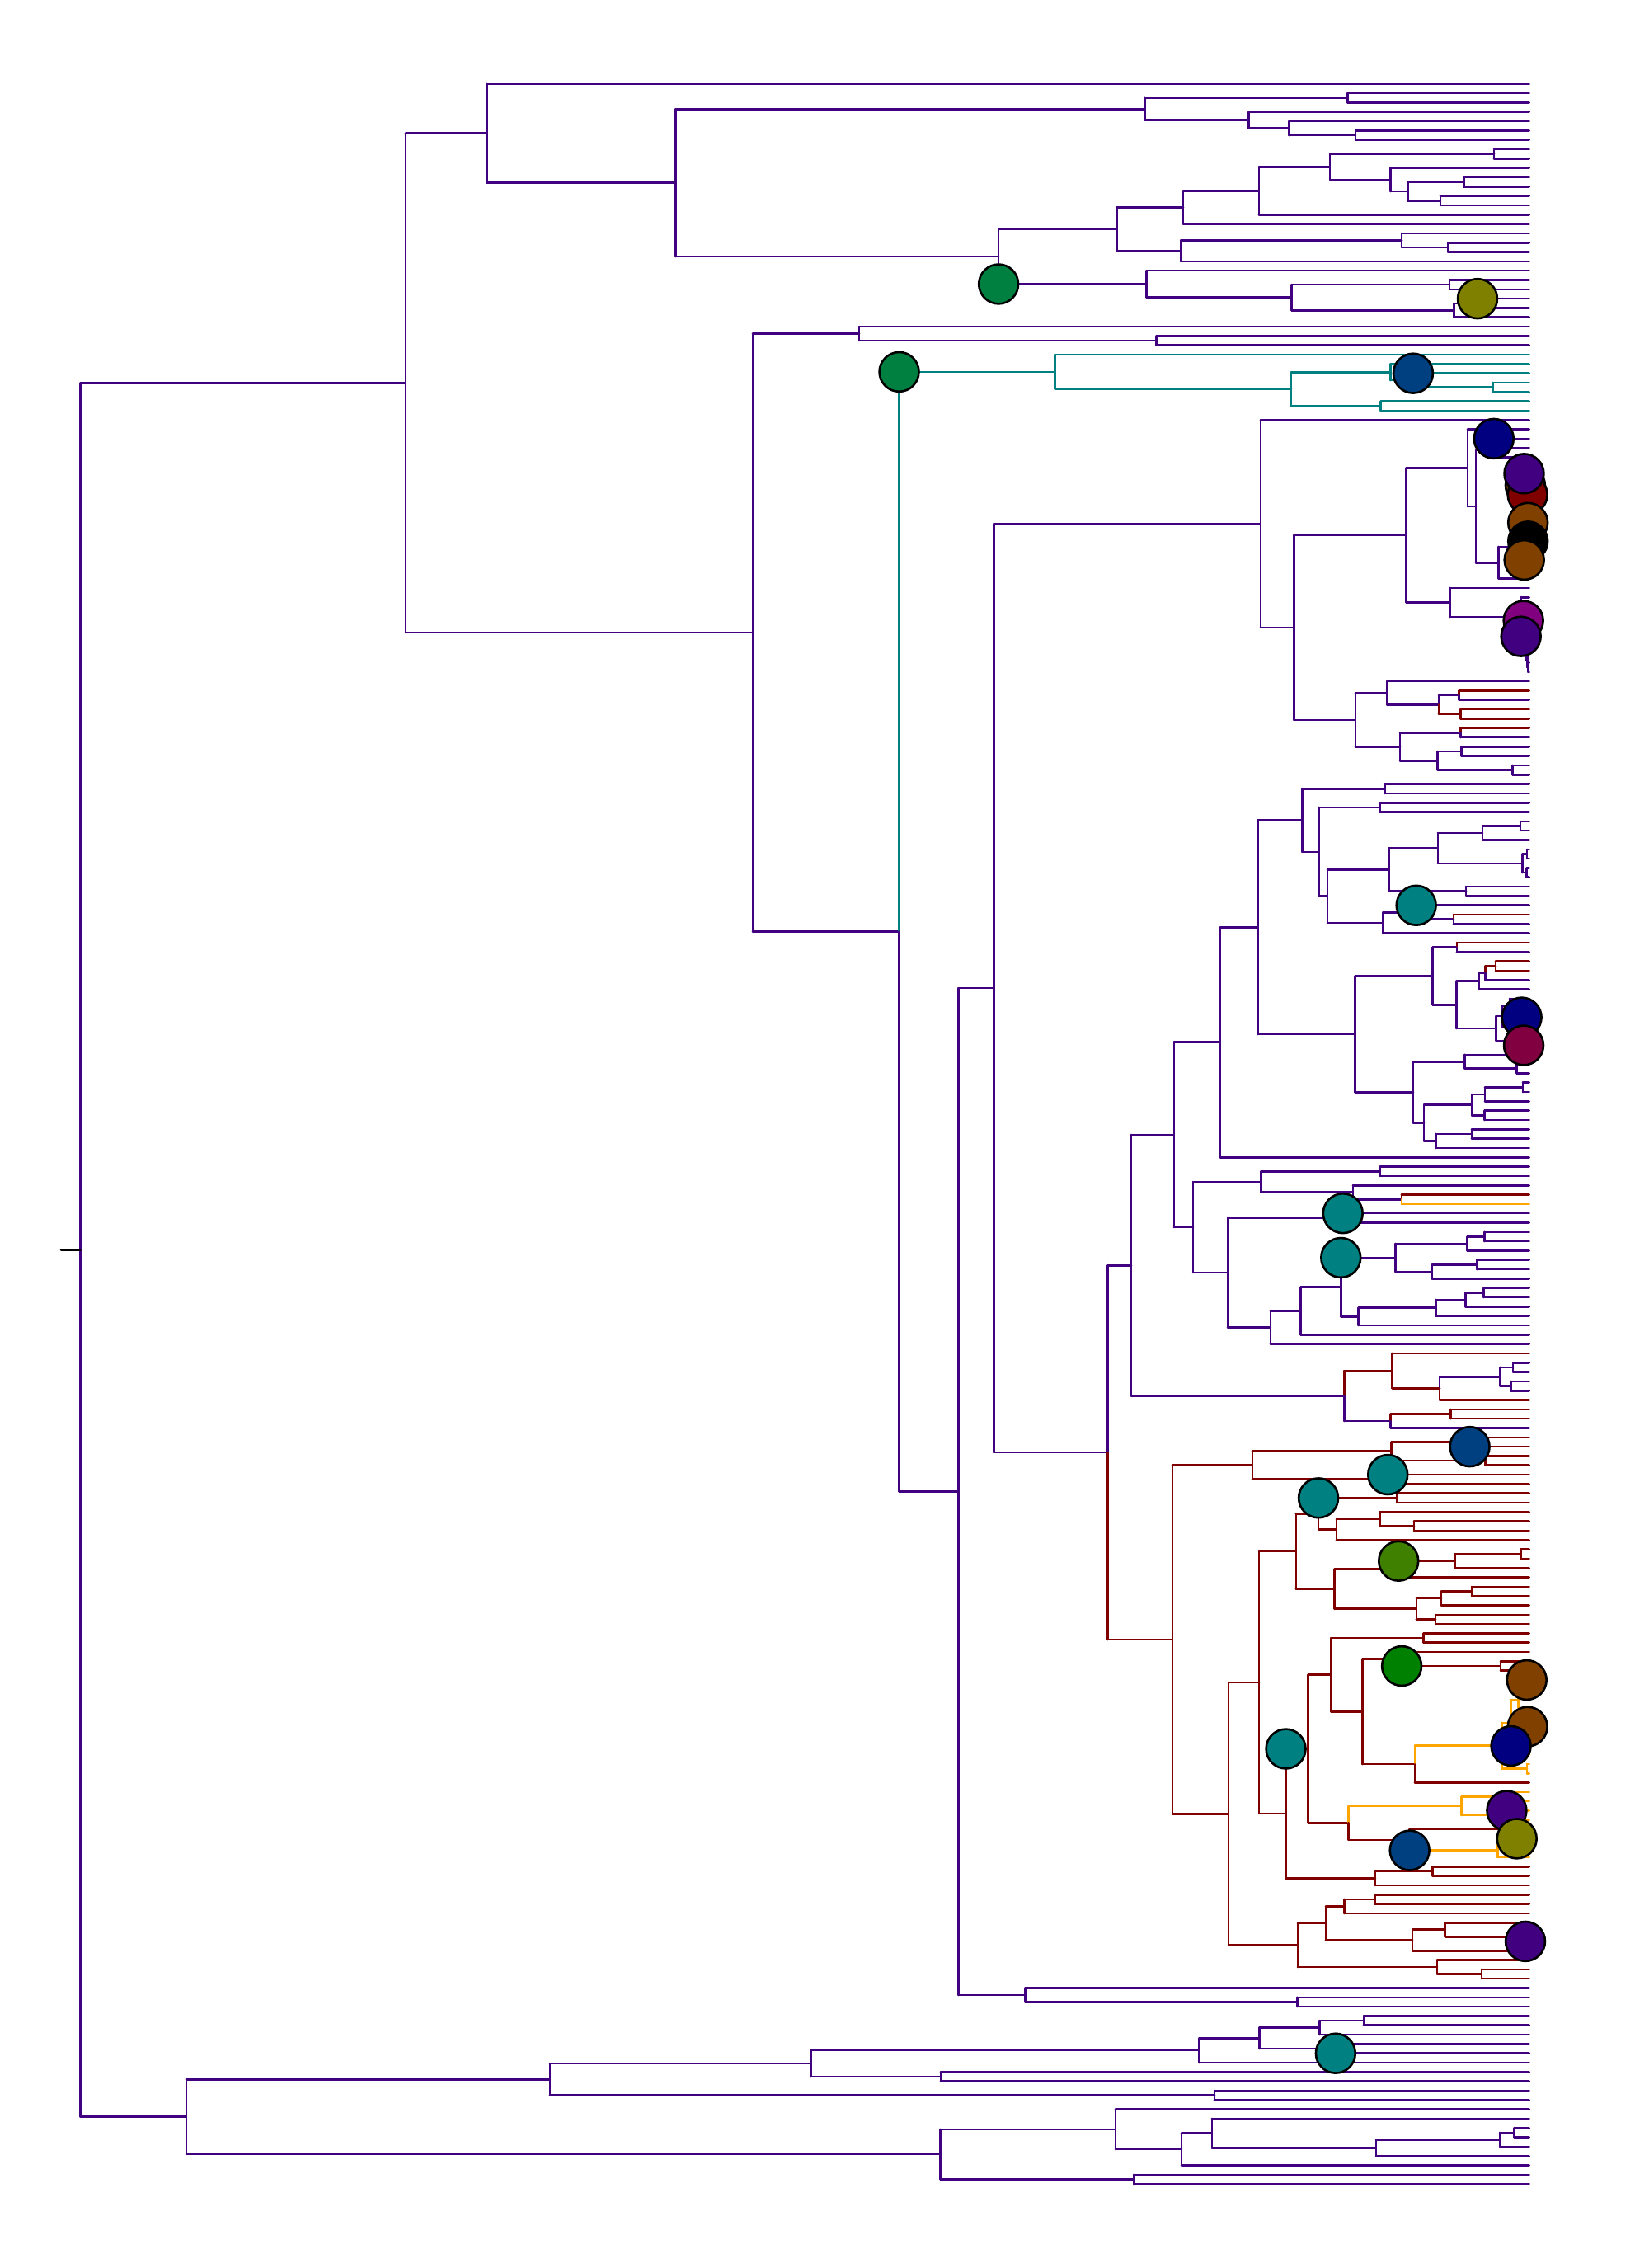} 

     {\sf \vskip -0.5cm \qquad SURFACE}
 \end{minipage}
 \begin{minipage}{0.45\textwidth}
%'     \vskip - 0.5 cm

\includegraphics[width=\maxwidth,height=0.45\textheight]{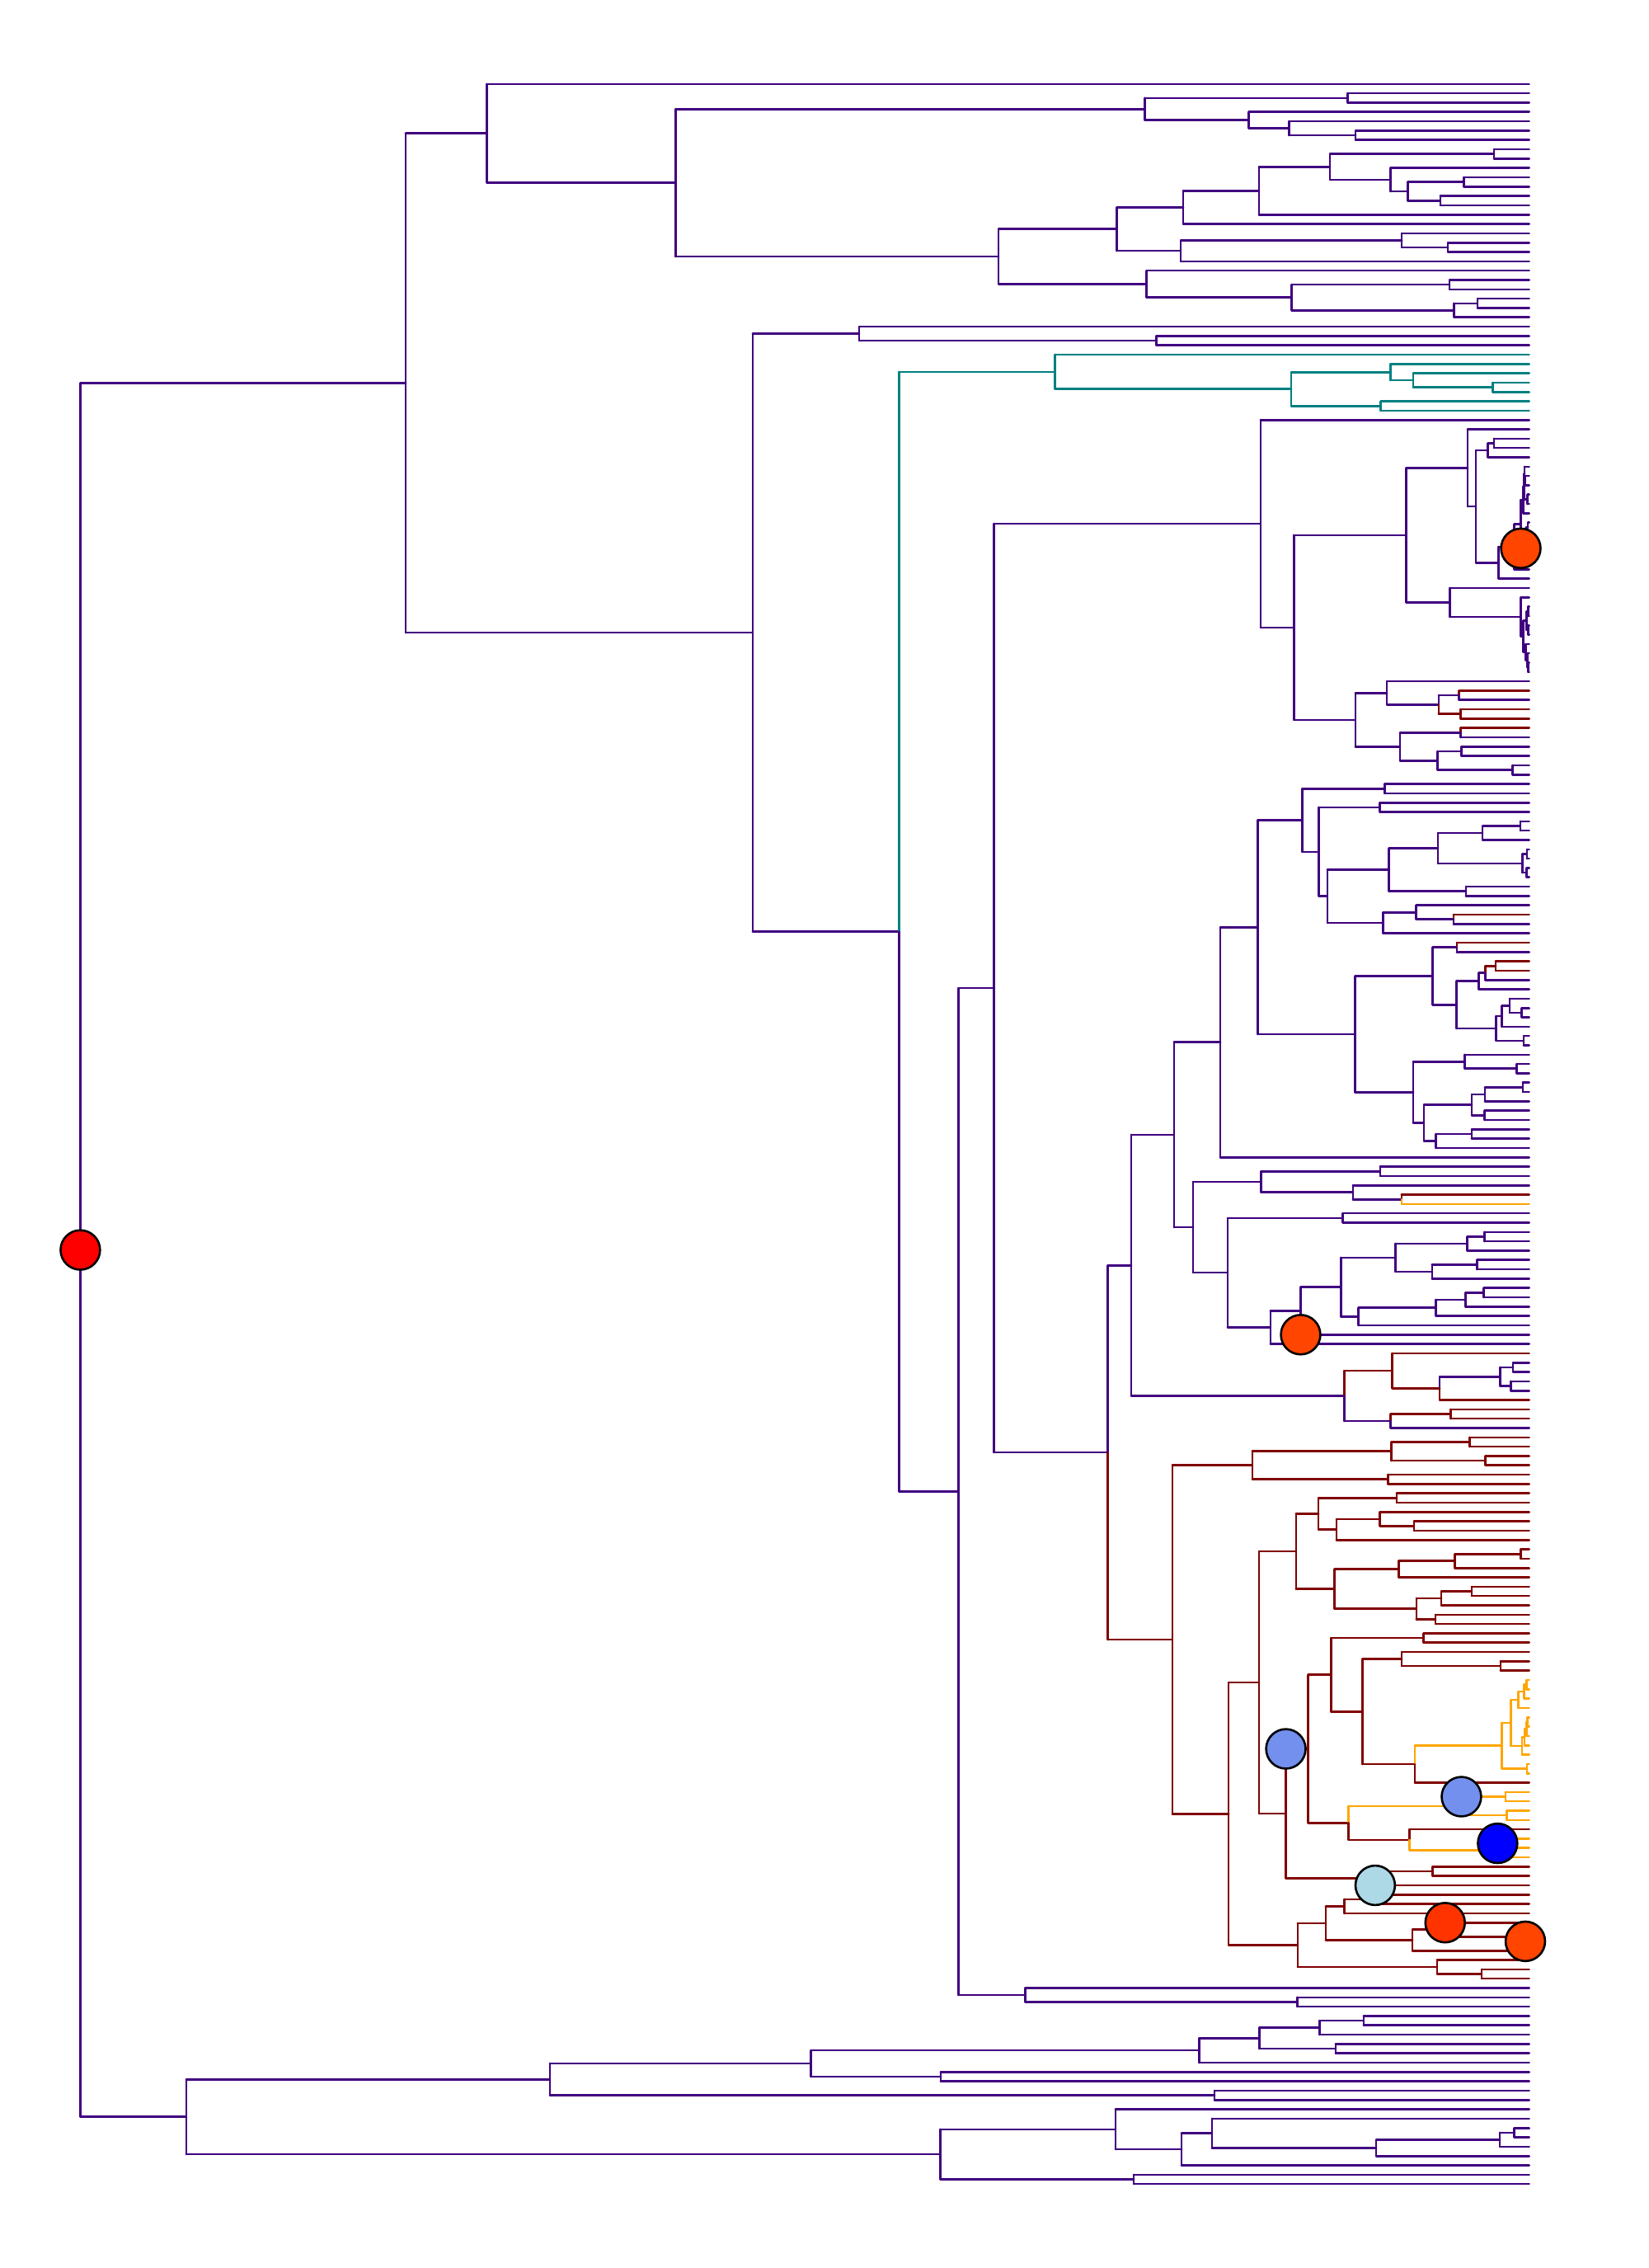} 

     {\sf \vskip -0.5cm \qquad OUshifts}
    \end{minipage}
        \caption{Solutions found by the EM (top left), \printR{bayou} (top right), \printR{SURFACE} (bottom left) and \printR{OUshifts} (bottom right). The branch coloring represents the habitats. For the EM, \printR{bayou} and \printR{OUshifts}, the shifts coloring represents their values, from blue (negative) to red (positive). For \printR{bayou}, the size of the circles are proportional to their posterior probability. For \printR{SURFACE}, the $13$ colors of the shifts represent the regimes.
}\label{fig:chelonia_sol_bayou}
 %   \caption{From top to bottom, solutions found by our method, \printR{bayou} and \printR{SURFACE}. The branch coloring represents the habitats. For our method and \printR{bayou}, the shift coloring represents their values, from blue (negative) to red (positive). For \printR{bayou}, the size of the circles are proportional to their posterior probability. For \printR{SURFACE}, the $13$ colors of the shifts represents the regimes.}

    \end{center}
  \end{figure}

\newpage
\section{Practical Implementation}\label{supp:practical_implementaion}

The statistical method described here was implemented on the statistical software \citeR{R}, and the code is freely available on GitHub (\url{https://github.com/pbastide/Phylogenetic-EM}). Phylogenetic trees were handled thanks to the package \citeR{ape}. Packages \citeR{TreeSim}, \citeR{robustbase} and \printR{quadrupen} \citep{chiquet2012} were used, respectively, for random tree generation, robust regression and Lasso regression. The penalty described in proposition~\ref{prop:model_selection} is implemented in package \citeR{LINselect}.\par
Parallelization was achieved thanks to \printR{R} packages \citeR{foreach} and \citeR{doParallel}.\par
Package \citeR{mclust} was used for ARI computations. Plots were made thanks to packages \citeR{ggplot2} and \citeR{reshape2}.
