# Supplementary material for: Detection of adaptive shifts on phylogenies using shifted stochastic processes on a tree
Source: arXiv:1508.00225 source file (2016-07-13)
Supplement: Supplementary file 2 [file enumeration.tex]

\section{Enumeration of Equivalence Classes}\label{supp:proofs_enumaration}

 \begin{definition}[Coloring concatenation]
       Let $i$ be a node of tree $\Tr$ with $L_i$ daughter nodes $(i_1, \cdots, i_{L_i})$, $L_i\geq 2$, and assume that the tips are colored according to the application $d\in (\Cr_K)^n$. We denote by $\Tr_i$ the sub-tree rooted at node $i$, and by $\Ar_{\Tr_i}(d)$ the set of parsimonious shifts allocations on $\Tr_i$ that produce a coloring of the tips compatible with $d$. At the root, $\Ar_{\Tr_1}(d) = \Ar_{\Tr}(d) = \phi^{-1}(d)$.
       \begin{itemize}
       \item For $k\in\Cr_K$, $S_i(k)$ is the \emph{cost} of starting from node $i$ with color $k$, \emph{i.e.} the minimal number of shifts needed to get the right coloring of the tips of $\Tr_i$, when starting with color $k$.
        \item $S_i^{tot} = \min_{k\in\Cr_K} S_i(k)$ is the minimal cost of subtree $\Tr_i$, \emph{i.e.} the number of shifts of a parsimonious coloring. $\Lr_i = \argmin_{k\in\Cr_K} S_i(k)$ is the set of colors root $i$ can take in a parsimonious coloring of sub-tree $\Tr_i$.
        \item For $k\in\Cr_K$, $\Br_{\Tr_i}^k$ is the set of colorings of $\Tr_i$ that respect the colors at the tips, have $S_i(k)$ shift, and start with color $k$.
        \item For $\Kr \subset \Cr_K$, $\Br_{\Tr_i}^\Kr = \bigcup_{k\in\Kr}\Br_{\Tr_i}^k$. Hence, $\Ar_{\Tr_i}(d) = \Br_{\Tr_i}^{\Lr_i}$, and the computation of $\Ar_{\Tr_i}(d)$ only requires the computation of $S_i(k)$ and $\Br_{\Tr_i}^k$ for any $k\in\Cr_K$.
        \item For $(p_1, \cdots, p_{L_i}) \in (\Cr_K)^{L_i}$, and $(B_1, \cdots, B_{L_i}) \in \Br_{\Tr_{i_1}}^{p_1} \times \cdots \times \Br_{\Tr_{i_{L_i}}}^{p_{L_i}}$ we define, for $k\in\Cr_K$, the concatenation 
        \(
         B = \sideset{^k}{}\bigoplus_{l=1}^{L_i} B_l, B \in \Br_{\Tr_i}^k,
        \)
        by:
        \(
         \begin{cases}
          B(i) = k\\
          B(j) = B_l(j) & \text{ if } i \in \Tr_{i_l}
         \end{cases}
        \).
  As the sub-trees $\Tr_{i_l}$, $l\in \intervalleentier1{L_i}$ do not overlap, this application is correctly defined on the nodes of $\Tr_i$.

       \end{itemize}

      \end{definition}
      
      Using these definitions, we can state the following recursion formula:
      
      \begin{proposition}[Enumeration Recursion Formula]\label{prop:recursion_eq_classes}
       Let $k\in\Cr_K$, and $i\in\intervalleentier{1}{m+n}$. If $i$ is a tip of the tree, then\\
    \begin{minipage}{0.5\textwidth}
 \[
  S_{i}(k) = \begin{cases}
           0 & \text{ if $d(i) = k$}\\
           +\infty & \text{ otherwise}
           \end{cases}
  \]
   \end{minipage}
   \begin{minipage}{0.5\textwidth}
 \[
  \Br_{\Tr_i}^{k} = \begin{cases}
           \{i\mapsto k\} & \text{ if $d(i) = k$}\\
           \emptyset & \text{ otherwise}
           \end{cases}
  \]
   \end{minipage}

       If $i$ is a node of tree $\Tr$ with ${L_i}$ daughter nodes $(i_1, \cdots, i_{L_i})$, ${L_i}\geq 2$, and assuming that $S_{i_l}(k)$ and $\Br_{\Tr_{i_l}}^k$ are known for any $l\in\intervalleentier1{L_i}$ and $k\in\Cr_K$, define, for $l\in\intervalleentier1{L_i}$:
        \[
    \Kr_k^l = \argmin_{1\leq p \leq K} \left\{ S_{i_l}(p) + \Ibb\{p \neq k\} \right\} 
	\]
	As these sets are not empty, let $(p_1, \dotsc p_{L_i}) \in \Kr_k^1 \times \dotsc \times \Kr_k^{L_i}$. Then
       \[
        S_i(k) = \sum_{l = 1}^{L_i} \left(S_{i_l}(p_l) + \Ibb\{p_l \neq k\}\right) 
        \quad \text{and} \quad
        \Br_{\Tr_i}^{k} = \left\{\sideset{^k}{}\bigoplus_{l=1}^{L_i} B_l : \forall l \in \intervalleentier{1}{L_i},  B_l \in \Br_{\Tr_{i_l}}^{\Kr_k^l}\right\}
       \]

%         \[
% 	  \forall k \in \Cr_K,~ \forall (p_1, \dotsc p_L) \in \Kr_k^1 \times \dotsc \times \Kr_k^L,~ \quad S_i(k) = \sum_{l = 1}^L \left(S_{i_l}(p_l) + \Ibb\{p_l \neq k\}\right)
% 	\]

      \end{proposition}
      
      \begin{proof}
       The actualization of $S_i(k)$ is the same as in the Sankoff algorithm \citep{sankoff1975}. The set $\Br_{\Tr_i}^{k}$ is then obtained by enumerating all the possible ways of concatenating children sets $\Br_{\Tr_{i_l}}^{\Kr_k^l}$, each of which is the ensemble of solutions for the sub-tree $\Tr_{i_l}$ that realize the minimal number of shifts when starting in state $k$.
       %For $\Br_{\Tr_i}^{k}$, we consider $\Br_{\Tr_{i_l}}^{\Kr_k^l}$ that is the ensemble of solutions for the sub-tree $\Tr_{i_l}$ that realize the minimal number of shifts when starting in state $k$. The concatenation just enumerate all the possible configurations of such optimal solutions on each sub-trees.
      \end{proof}
      
      Remarking that $T_i(k) = \card{\Br_{\Tr_i}^{k}}$, proposition \ref*{prop:size_eq_class} of the main text follows immediately.
