# Supplementary material for: Detection of adaptive shifts on phylogenies using shifted stochastic processes on a tree
Source: arXiv:1508.00225 source file (2016-07-13)
Supplement: Supplementary file 3 [file practical_implementation.tex]

\section{Practical Implementation}\label{supp:practical_implementaion}

The statistical method described here was implemented on the statistical software \citeR{R}, and the code is freely available on GitHub (\url{https://github.com/pbastide/Phylogenetic-EM}). Phylogenetic trees were handled thanks to the package \citeR{ape}. Packages \citeR{TreeSim}, \citeR{robustbase} and \printR{quadrupen} \citep{chiquet2012} were used, respectively, for random tree generation, robust regression and Lasso regression. The penalty described in proposition~\ref{prop:model_selection} is implemented in package \citeR{LINselect}.\par
Parallelization was achieved thanks to \printR{R} packages \citeR{foreach} and \citeR{doParallel}.\par
Package \citeR{mclust} was used for ARI computations. Plots were made thanks to packages \citeR{ggplot2} and \citeR{reshape2}.
