# Supplementary material for: Detection of adaptive shifts on phylogenies using shifted stochastic processes on a tree
Source: arXiv:1508.00225 source file (2016-07-13)
Supplement: Supplementary file 4 [file proof_model_selection.tex]

\section{Proof of Proposition~\ref{prop:model_selection} for Model Selection} \label{supp:proof_model_selection}

\PB{We prove the proposition using the linear formulation $\vect{s} + \gamma \vect{E}$, with $\vect{E} \sim \Normal(0, \matr{V})$, as derived in the main text for the OUsun (with $\vect{s} = \matr{T}\matr{W}(\alpha)\vect{\Delta}$, $\gamma^2 = \sigma^2/(2\alpha)$, and $V_{ij} = e^{-\alpha d_{ij}}$, see Formula~(\ref{eq:OU_lin_def_X})). Note that this framework also holds for the BM with a fixed root (with $\vect{s} = \matr{T}\vect{\Delta}$, $\gamma = \sigma$, and $V_{ij} = t_{ij}$, see Formula~(\ref{eq:BM_lin_def_X})).}

We first handle the case where there are no correlations (\PB{$\matr{V}$ diagonal}), and then use a Cholesky decomposition to handle the general case. \PB{Note that the case $\matr{V}$ diagonal can be seen as the limit of the OUsun when $\alpha = +\infty$, or as a BM on a star tree.}
    
    \emph{Case \PB{$\matr{V}$ diagonal}}
    
    In the iid case, we just need to check the conditions of theorem~\ref{th:model_selection_baraud2009}. This paragraph is highly inspired by the derivation of the bound for the detection of non-zero mean components exposed in \citet{baraud2009} (sub-section 5.2). Assume that $D_\eta = K_\eta + 1 \leq p \leq n-7$ for all $\eta\in\Mr$. The estimator is defined by $\vect{\hat{s}}_{\hat{K}}$, with:
    \[
    \hat{K} = \argmin_{0\leq K \leq p-1} \mahanorm{\vect{Y} - \vect{\hat{s}}_K}{V}^2 \left( 1 + \frac{\pen_{A, \Lr}(K)}{n-K-1}\right)
    \]
    From the definition of $\vect{\hat{s}}_K$, and as the penalty depends on the model only through its number of shifts, we get that $\vect{\hat{s}}_{\hat{K}} = \vect{\hat{s}}_{\hat{\eta}}$ the minimizer of the criterion of theorem~\ref{th:model_selection_baraud2009} (with $N_\eta = n-D_\eta = n - K_\eta - 1$).
    We then have:
    \[
     \Omega' =  \sum_{\eta \in \Mr} (D_\eta + 1) e^{-L_\eta}= \sum_{K = 0}^{p-1} \card{\Sr_{K}^{PI}} (K + 2) e^{-L_K}
    \]
     With the weights $L_K$ defined in equation~\ref{eq:L_K} of the proposition, we get:
    \[
     \Omega' =  \sum_{K = 0}^{p-1} \frac{1}{K+2} \leq \log(p) \leq \log(n)
    \]
    As:
     \begin{align*}
      L_K \leq \log \binom{n+m-1}{K} + 2\log(K+2) &\leq K\log(n+m-1) + 2\log(K+2)\\
      & \leq K\log(2n-2) + 2(K+1)\\
      & \leq (K+1)(2 + \log(2) + \log(n))\\
      & \leq p(2 + \log(2) + \log(n))
     \end{align*}
      if
      \(p \leq \min\left(\frac{\kappa n}{2 + \log(2) + \log(n)}, n-7\right)\), then  $\max(L_\eta, D_\eta) \leq \kappa n$ for any $\eta\in\Mr$, and we get the announced bound from the second proposition of theorem~\ref{th:model_selection_baraud2009}.
      
      \emph{Case \PB{$\matr{V}$ not diagonal}}
      
      Using a Cholesky decomposition, we can find a lower triangular matrix $\matr{L}$ such that $\matr{V} = \matr{L}\matr{L}^T$. Then, denoting $\vect{Y}' = \matr{L}^{-1}\vect{Y}$, $\vect{s}'=\matr{L}^{-1}\vect{s}$, and $\vect{E}' = \matr{L}^{-1}\vect{E}$, we have \(\vect{Y}' = \vect{s}' + \gamma \vect{E}'\), with $\vect{E}'\sim\Normal(0, \matr{I_n})$, and we can apply theorem~\ref{th:model_selection_baraud2009} as above. As we changed the metric, the estimators are projections on the linear spaces $S'_\eta=\matr{L}^{-1}S_\eta$ for $\eta \in \Mr$, and we have:
      \begin{align*}
      \vect{\hat{s}}'_\eta &= \Proj_{S'_\eta}\vect{Y}' = \argmin_{\vect{a}' \in S'_\eta} \norm{\vect{Y}'-\vect{a}'}^2 = \argmin_{\vect{a}' \in S'_\eta} \norm{\matr{L}^{-1}\vect{Y}-\matr{L}^{-1}\matr{L}\vect{a}'}^2\\
      &= \argmin_{\vect{a}' \in S'_\eta} \mahanorm{\vect{Y} - \matr{L}\vect{a}'}{V}^2 = \matr{L}^{-1}\argmin_{\vect{a} \in S_\eta} \mahanorm{\vect{Y} - \vect{a}}{V}^2 = \matr{L}^{-1}\vect{\hat{s}}_\eta
      \end{align*}
      So $\mahanorm{\vect{s} - \vect{\hat{s}}_{\hat{\eta}}}{V}^2 = \norm{\vect{s}' - \vect{\hat{s}}'_{\hat{\eta}}}^2$ and $\mahanorm{\vect{Y} - \vect{\hat{s}}_\eta}{V}^2 = \norm{\vect{Y}' - \vect{\hat{s}}'_\eta}^2$, and, as the form of the penalty does not depend on $V$, by minimizing:
      \[
      \Crit_{LS}(K) = \norm{\vect{Y}' - \vect{\hat{s}}'_K}^2 \left( 1 + \frac{\pen_{A, \Lr}(K)}{n - K - 1}\right) = \mahanorm{\vect{Y} - \vect{\hat{s}}_K}{V}^2 \left( 1 + \frac{\pen_{A, \Lr}(K)}{n - K -1}\right)
      \]
      we get the announced bound on $\Espe{\frac{\mahanorm{\vect{s} - \vect{\hat{s}}_{\hat{K}}}{V}^2}{\gamma^2}} = \Espe{\frac{\norm{\vect{s}' - \vect{\hat{s}}'_{\hat{K}}}^2}{\gamma^2}}$.
