# Supplementary material for: Detection of adaptive shifts on phylogenies using shifted stochastic processes on a tree
Source: arXiv:1508.00225 source file (2016-07-13)
Supplement: Supplementary file 5 [file proofs_identifiability.tex]

\section{Technical Proofs of Section~3}\label{supp:proofs_identifiability}

   \begin{proof}[Proof of Proposition~\ref{prop:kernel_of_T}]
%       Let $K^i$ be a vector defined as in the proposition. Then
%       \begin{align*}
%       (TK^i)_j &= T_{ji}K^i_i + \sum_{l=1}^{L_i}T_{jd_l}K^i_{d_l}\\
%       & = T_{ji} - \sum_{l=1}^{L_i}T_{jd_l}\\
%       & = \Ibb\{i \in \Par(m+j)\} -  \sum_{l=1}^{L_i}\Ibb\{d_l \in \Par(m+j)\}
%       \end{align*}
%       If $i\notin \Par(m+j)$, then $d_l\notin \Par(m+j)$ for all $l\in \intervalleentier1{L_i}$ and $(TK^i)_j = 0$. Otherwise, $i$ is an ancestor of $m+j$. Since $i$ is internal, one of its direct descendant is also an ancestor of $m+j$, so that the sum cancels out.
Let $i\in\intervalleentier1m$ be an internal node with $L_i$ \PB{children} nodes $(d_1, \cdots, d_{L_i})$ and $\vect{K}^i$ the corresponding vector, defined as in the proposition. Then, for any $j\in \intervalleentier{1}{m+n}$:
      \[
      (\matr{U}\vect{K}^i)_j = U_{ji}K^i_i + \sum_{l=1}^{L_i}U_{jd_l}K^i_{d_l}
      %& = U_{ji} - \sum_{l=1}^{L_i}U_{jd_l}\\
       = \Ibb\{i \in \Par(j)\} -  \sum_{l=1}^{L_i}\Ibb\{d_l \in \Par(j)\}
      \]
      We can then distinguish three possibilities:
      \begin{itemize}
      \item If $i\notin \Par(j)$, then $d_l\notin \Par(j)$ for all $l\in \intervalleentier1{L_i}$ and $(\matr{T}\vect{K}^i)_j = 0$.
      \item If $j = i$, then $i \in \Par(j)$, and, by definition, $d_l \notin \Par(j)$ for any $l\in \intervalleentier1L$, so $(\matr{U}\vect{K}^i)_i = 1$.
      \item Else, if $i$ is an ancestor of $j$, with $i\neq j$, then, as $i$ is internal, one (and only one) of its \PB{child} $d_l$ is also an ancestor of $j$ (potentially $j$ itself), so that the sum cancels out.
      \end{itemize}
      This proves that 
      \begin{equation}
      \forall i \in \intervalleentier1m, \matr{U}\vect{K}^i = (\delta_{ij})_{1\leq j \leq m+n}
      \label{eq:kernel_of_T}
      \end{equation}
      %if $i \in \Par(m+j)$, then, as $m+j > i$, there is a unique $l\in\intervalleentier1{L_i}$ such that $d_l \in \Par(m+j)$, and $(TK^i)_j = 0$. 
      In particular, as $\matr{T}\vect{K}^i$ is the vector of the last $n$ coordinates of $\matr{U}\vect{K}^i$, this shows that the vectors $(\vect{K}^1, \cdots, \vect{K}^m)$ are in the kernel of $\matr{T}$.\par
      Then, as we found $m$ independent vectors in the kernel of $\matr{T}$, which is a space of dimension lower than $m$ (as the $n$ columns of $\matr{T}$ representing tips are linearly independent, and by the rank theorem), this family of vector is a basis of the kernel space.
      \end{proof}
      
            \begin{proof}[Proof of lemma~\ref{lemma:U_invertible}]
      First, $(\vect{b}_{m + 1}, \cdots, \vect{b}_{m+n})$ is a family of $n$ independent vectors of $S$ of dimension $n$, so is a basis of $S$, and $b'$ is a basis adapted to $\ker(\matr{T})\oplus S$.\par
      Let $i\in\intervalleentier{1}{m+n}$. Let's show that $\matr{U}\vect{b}'_{i} = \vect{b}_i$. If $m+1\leq i \leq m+n$, then $\vect{b}'_i = \vect{b}_i$, and $\matr{U}\vect{b}_i = \vect{b}_i$ is the $i^{th}$ column of $\matr{U}$. Otherwise, if $1\leq i \leq m$, then $\vect{b}'_i=\vect{K}^{i}${, and, from equation~\ref{eq:kernel_of_T}, $\matr{U}\vect{b}'_i = \vect{b}_i$.} This shows that $\matr{U}$ is the change of basis matrix between $b$ and $b'$.
      \end{proof}
      
                \begin{proof}[Proof of Proposition~\ref{prop:parsimony_linear_independence}]
      By contraposition, let's first assume that the vector-columns $(T_i)_{i\in\Supp(\vect{\Delta})}$ are linearly dependent, and prove that $\vect{\Delta}$ is not parsimonious. This means that we can find a vector $\vect{E}$, $\vect{E}\in\R^{m+n}$, such that $\Supp(\vect{E}) \subset \Supp(\vect{\Delta})$, and $\matr{T}\vect{E}=0$. We can hence find $j\in\Supp(\vect{\Delta})$, $j>1$, such that $E_j\neq 0$. Then if $\lambda = -\Delta_j/E_j$, the vector $\vect{\Delta}'=\vect{\Delta} + \lambda \vect{E}$ is a vector of shifts on the tree with one less non-zero coordinate than $\vect{\Delta}$ such that $\matr{T}\vect{\Delta}'=\vect{m_Y}$. Hence, $\vect{\Delta}$ is not parsimonious.\par
      Reciprocally, by contraposition, assume that $\vect{\Delta}$ is not parsimonious. Then by proposition~\ref{prop:Kshifts_K+1clusters}, it produces $p$ groups, with $p\leq K$. Hence the application associated with $(T_i)_{i\in\Supp(\vect{\Delta})}$ goes from a space of dimension $K+1$ to a space of dimension $p\leq K$, and hence is not injective, and the family $(T_i)_{i\in\Supp(\vect{\Delta})}$ is not independent.
      \end{proof}
