# Supplementary material for: Detection of adaptive shifts on phylogenies using shifted stochastic processes on a tree
Source: arXiv:1508.00225 source file (2016-07-13)
Supplement: Supplementary file 6 [file suppEM.tex]

%%%%%%%%%%%%%%%%%%%%%%%%%%%%%%%%%%%%%%%%%%%%%%%%%%%%%%%%%%%%%%%%%%%%%%%
%%%%%%%%%%%%%%%%%%%%%%%%%%%%%%%%%%%%%%%%%%%%%%%%%%%%%%%%%%%%%%%%%%%%%%%
\section{Technical Details of the EM} \label{supp:EM}
%%%%%%%%%%%%%%%%%%%%%%%%%%%%%%%%%%%%%%%%%%%%%%%%%%%%%%%%%%%%%%%%%%%%%%%
%%%%%%%%%%%%%%%%%%%%%%%%%%%%%%%%%%%%%%%%%%%%%%%%%%%%%%%%%%%%%%%%%%%%%%%

%%%%%%%%%%%%%%%%%%%%%%%%%%%%%%%%%%%%%%%%%%%%%%%%%%%%%%%%%%%%%%%%%%%%%%%
\subsection{E Step}\label{supp:E_step}

Given a set of parameters $\vvect{\theta}^{(h)}$, we have:
     \[
      \vect{X} = (\vect{Z}, \vect{Y}) \sim \Normal \left(  \vect{m}^{(h)} = \left(\begin{array}{c} \vect{m}^{(h)}_\vect{Z} \\ \vect{m}^{(h)}_\vect{Y} \end{array} \right) ~,~ \matr{\Sigma}^{(h)} = \left(\begin{array}{cc} \matr{\Sigma}^{(h)}_{\vect{Z}\vect{Z}} & \matr{\Sigma}^{(h)}_{\vect{Y}\vect{Z}} \\ \matr{\Sigma}^{(h)}_{\vect{Z}\vect{Y}} & \matr{\Sigma}^{(h)}_{\vect{Y}\vect{Y}} \end{array} \right)\right)
    \]
    hence:
    \[
    \begin{split}
    \sachant{\vect{Z}}{\vect{Y}} \sim \Normal \big(& \vect{m}^{(h)}_{\sachant{\vect{Z}}{\vect{Y}}} = \vect{m}^{(h)}_\vect{Z} + \matr{\Sigma}^{(h)}_{\vect{Z}\vect{Y}} (\matr{\Sigma}^{(h)}_{\vect{Y}\vect{Y}})^{-1} (\vect{Y} - \vect{m}^{(h)}_\vect{Y})
    ,\\
    & \matr{\Sigma}_{\sachant{\vect{Z}}{\vect{Y}}} = \matr{\Sigma}^{(h)}_{\vect{Z}\vect{Z}} - \matr{\Sigma}^{(h)}_{\vect{Z}\vect{Y}} (\matr{\Sigma}^{(h)}_{\vect{Y}\vect{Y}})^{-1} \matr{\Sigma}^{(h)}_{\vect{Y}\vect{Z}} \big)
    \end{split}
    \]
    
    \begin{remark}
    We can see that this approach forces us to invert $\matr{\Sigma}^{(h)}_{\vect{Y}\vect{Y}}$, a $n\times n$ matrix, which is a costly operation, of order $O(n^3)$. It also computes the complete matrix  $\matr{\Sigma}_{\sachant{\vect{Z}}{\vect{Y}}}$ whereas we only need a linear number of its coefficients: conditional variances and covariances of the form $\Covasq{\vect{Z}_{i}}{\vect{Z}_{\pa(i)}}{\vect{Y}}$. Due to the tree structure and to the Gaussian nature of the processes studied, it is possible to compute all the quantities needed in a linear time, using a ``forward-backward''-like algorithm (here,  ``upward-downward'', see \citet{lartillot2014} for a similar algorithm.). The upward step is similar to the pruning algorithm described in \citet[chap. 23]{felsenstein2004}. See also \citet{hoane2013b} for an algorithm linear in the number of iterations.
    \end{remark}

%%%%%%%%%%%%%%%%%%%%%%%%%%%%%%%%%%%%%%%%%%%%%%%%%%%%%%%%%%%%%%%%%%%%%%%
\subsection{Complete Likelihood Computation}\label{supp:likelihood}

Using the incomplete data model described in section \ref{subsec:latent_model}, we can write:
    \[
    p_{\vvect{\theta}}(\vect{X}) = p_{\vvect{\theta}}(X_1)\prod_{j=2}^{m+n}p_{\vvect{\theta}}\left(\sachant{X_j}{X_{\pa(j)}}\right)
    \]
    Taking the expectation, we get for the BM:
%     \begin{equation}\label{eq:BM_completed_log_lik}
%     \begin{split}
%     -2\log p_{\vvect{\theta}}(\vect{X}) = & (m+n)\log(2\pi) + 2\sum_{j=2}^{m+n}\log(\ell_j) + \log \gamma^2 + (m+n-1) \log \sigma^2 \\
%       & + \frac1{\gamma^2} \left(X_1 - \mu\right)^2 + \frac1{\sigma^2} \sum_{j = 2}^{m+n} \ell_j^{-1} \left(X_j - X_{\pa(j)}- \sum_k \Ibb\{\tau_k = b_j\} \delta_k\right)^2 \\
%     \end{split}
%     \end{equation}
%     and, for the OUsun:
%     \begin{equation}\label{eq:OU_completed_log_lik}
%       \begin{split}
%       -2\log p_{\vvect{\theta}}(\vect{X}) = &  (m+n)\log(2\pi) + 2\sum_{j=2}^{m+n}\logc_j(\alpha) + (m+n) \log (\gamma^2) \\
%   & + \frac1{\gamma^2} \left(X_1 - \mu\right)^2 + \frac{1}{\gamma^2} \sum_{j=2}^{m+n} c_j(\alpha)^{-1}  \left(  X_j - X_{\pa(j)}e^{-\alpha \ell_j} - \beta^{j}\left(1 - e^{-\alpha \ell_j}\right)\right)^2\\
%       \end{split}
%      \end{equation}
%     Taking the expectation, we get:
    \begin{equation} \label{eq:BM_expectation_completed_log_lik}
      \begin{split}
	-2\Espesq{\log p_{\vvect{\theta}}(\vect{X})}{\vect{Y}}
	 & =  A + \log \gamma^2 + \frac{1}{\gamma^2} \left( \Varisq{X_1}{\vect{Y}} + \left(\Espesq{X_1}{\vect{Y}} - \mu\right)^2\right) \\
	  & + (m+n-1) \log \sigma^2 + \frac1{\sigma^2} \sum_{j=2}^{m+n} \ell_j^{-1} \Varisq{X_j - X_{\pa(j)}}{\vect{Y}}\\
	  % & + \frac1{\sigma^2} \sum_{j=2}^{m+n} C_j^{BM}(\vvect{\tau}, \vvect{\delta}) \\
	  & + \frac1{\sigma^2} \sum_{j=2}^{m+n} C_j^{BM}(\PB{\vect{\Delta}}) \\
	\end{split}
%  \raisetag{-2.5 cm}
    \end{equation}
    and, for the OUsun:
    \begin{equation}\label{eq:OU_expectation_completed_log_lik}
      \begin{split}
	-2\Espesq{\log p_{\vvect{\theta}}(\vect{X})}{\vect{Y}} & = B + \sum_{j=2}^{m+n}\log c_j(\alpha) + \frac{1}{\gamma^2} \Varisq{X_1}{\vect{Y}} + (m+n) \log \gamma^2\\
	  & + \frac{1}{\gamma^2} \sum_{j=2}^{m+n} c_j(\alpha)^{-1} \Varisq{X_j - X_{\pa(j)}e_j}{\vect{Y}}\\
%	  & + \frac{1}{\gamma^2}\left(\Espesq{X_1}{\vect{Y}} - \beta_0\right)^2 + \frac{1}{\gamma^2} \sum_{j=2}^{m+n} C_j^{OU}(\vvect{\tau}, \vvect{\delta}, \beta_0, \alpha)
	 & + \frac{1}{\gamma^2}\left(\Espesq{X_1}{\vect{Y}} - \beta_0\right)^2 + \frac{1}{\gamma^2} \sum_{j=2}^{m+n} C_j^{OU}(\alpha, \PB{\vect{\Delta}})
	\end{split}
%  \raisetag{-2.5 cm}
     \end{equation}
    where $A$ and $B$ are constants, and for each node $j$, $j \in \intervalleentier{2}{m+n}$, we define an actualization factor $c_j(\alpha) = 1-e_j(\alpha)^2$, with $e_j(\alpha) = e^{-\alpha\ell_j}$, and $C_j^{BM}$ and $C_j^{OU}$ are \emph{costs} associated with branch $b_j$:
    \[
      \left\{
	\begin{aligned}
%	 C_j^{BM}(\vvect{\tau}, \vvect{\delta}) & = \frac{1}{\ell_j} \left(\Espesq{X_j}{\vect{Y}} - \Espesq{X_{\pa(j)}}{\vect{Y}} - \sum_{k=1}^K \Ibb\{\tau_k = b_j\} \delta_k\right)^2\\
%	 C_j^{OU}(\vvect{\tau}, \vvect{\delta}, \beta_0, \alpha) &= \frac{1}{c_j(\alpha)} \Bigg(\Espesq{X_j}{\vect{Y}} - e_j\Espesq{X_{\pa(j)}}{\vect{Y}} - \beta_{j}\left(1 - e_j\right) \Bigg)^2
	 C_j^{BM}(\PB{\vect{\Delta}}) & = \frac{1}{\ell_j} \left(\Espesq{X_j}{\vect{Y}} - \Espesq{X_{\pa(j)}}{\vect{Y}} - \PB{\Delta_i}\right)^2\\
	 C_j^{OU}(\alpha, \PB{\vect{\Delta}}) &= \frac{1}{c_j(\alpha)} \Bigg(\Espesq{X_j}{\vect{Y}} - e_j\Espesq{X_{\pa(j)}}{\vect{Y}} - \beta_{j}\left(1 - e_j\right) \Bigg)^2
	\end{aligned}
      \right.
    \]

%%%%%%%%%%%%%%%%%%%%%%%%%%%%%%%%%%%%%%%%%%%%%%%%%%%%%%%%%%%%%%%%%%%%%%%
\subsection{M step}\label{supp:M_step}
Assuming that $p_{\vvect{\theta}^{(h)}}(\sachant{\vect{Z}}{\vect{Y}})$ is known, we need to compute $\vvect{\theta}^{(h+1)}$ by maximizing $\Esp_{\vvect{\theta}^{(h)}}[\sachant{\log p_{\vvect{\theta}}(\vect{Z},\vect{Y})}{\vect{Y}}]$. We have to deal with parameters of different nature, discrete or continuous. 
    %To choose the location $\vvect{\tau}^{(h+1)}$ and intensity $\vvect{\delta}^{(h+1)}$ of the $K$ shifts, we use a segmentation algorithm, as described below. 
    For a given \PB{vector $\vect{\Delta}^{(h+1)}$ of $K$ non-zero shifts,}
%     location $\vvect{\tau}^{(h+1)}$ and intensity $\vvect{\delta}^{(h+1)}$ of the $K$ shifts, 
we can exhibit closed formulas for $\mu^{(h+1)}$, $\sigma^{(h+1)}$ and $\gamma^{(h+1)}$, for the BM:
    \begin{equation*}
      \left\{
  \begin{aligned}
	  \mu^{(h+1)} & =  \Esp^{(h)}[ Z_1 \mid \vect{Y}] \\
	  \gamma^{2(h+1)} & =  \Var^{(h)}[Z_1 \mid \vect{Y}] \\
	  \sigma^{2(h+1)} & =
%	  	  \frac1{m+n-1} \left[ \sum_{j=2}^{m+n} \ell_j^{-1} \Var^{(h)} \left[X_j - X_{\pa(j)} \mid \vect{Y} \right] + C_j^{BM}\left(\vvect{\tau}^{(h+1)}, \vvect{\delta}^{(h+1)}\right) \right]
	  \frac1{m+n-1} \left[ \sum_{j=2}^{m+n} \ell_j^{-1} \Var^{(h)} \left[X_j - X_{\pa(j)} \mid \vect{Y} \right] + C_j^{BM}\left( \PB{\vect{\Delta}^{(h+1)}}\right) \right]
	\end{aligned}
      \right.
     \end{equation*}
    and, for the OUsun:
     \[
     \begin{split}
	(m+n) \gamma^{2(h+1)} &= \Var^{(h)}[X_1 \mid \vect{Y}]  + \sum_{j=2}^{m+n} c_j(\alpha)^{-1} \Var^{(h)} \left[X_j - X_{\pa(j)}e^{-\alpha \ell_j} \mid \vect{Y} \right]\\
%		  & + \left(\Esp^{(h)}\left[\sachant{X_1}{\vect{Y}}\right] - \beta^{(h+1)}_0\right)^2 + \sum_{j=2}^{m+n} C_j^{OU}\left(\vvect{\tau}^{(h+1)},\vvect{\delta}^{(h+1)}, \beta^{(h+1)}_0, \alpha^{(h)}\right)\\
	  & + \left(\Esp^{(h)}\left[\sachant{X_1}{\vect{Y}}\right] - \beta^{(h+1)}_0\right)^2 + \sum_{j=2}^{m+n} C_j^{OU}\left(\alpha^{(h)},  \PB{\vect{\Delta}^{(h+1)}}\right)\\
      \end{split}
      \]
    There is no such closed formula for $\alpha$. In the implementation we propose, this parameter is actualized after all the others, by doing a numerical maximization of the objective function.\par
    Finally, the \PB{vector $\vect{\Delta}^{(h+1)}$ of $K$ non-zero shifts}
%     location $\vvect{\tau}^{(h+1)}$ and intensity $\vvect{\delta}^{(h+1)}$ of the $K$ shifts
      can be chosen in an optimal way for the BM thanks to a simple algorithm explained below. In the OUsun case, we can only increase the objective function, and not maximize it. In that case, we hence use a Generalized EM algorithm \citep[GEM, see][]{dempster1977}.
    
    \paragraph{Optimal Shift Location for the BM} We want to minimize the sum of costs: 
%    \[C^{BM}(\vvect{\tau}, \vvect{\delta}) = \sum_{j=2}^{m+n}C_j^{BM}(\vvect{\tau}, \vvect{\delta})\] 
%    Each cost is associated to a branch $b_j$, $j\in\intervalleentier{2}{m+n}$, and, when the sum is minimal, $C_j^{BM}(\vvect{\tau}, \vvect{\delta})$ can only take two values: 
%    \begin{equation*}
%    \begin{cases}
%    \tilde{C}_j^{BM} = \ell_j^{-1} \left(\Esp^{(h)}\left[\sachant{X_j}{\vect{Y}}\right] - \Esp^{(h)}\left[\sachant{X_{\pa(j)}}{\vect{Y}}\right]\right)^2 & \text{if no shift on branch $b_j$} \\
%    0 & \text{if one shift on branch $b_j$}
%    \end{cases}
%    \end{equation*}
        \[C^{BM}(\vect{\Delta}) = \sum_{j=2}^{m+n}C_j^{BM}(\PB{\vect{\Delta}})\] 
    Each cost is associated to a branch $b_j$, $j\in\intervalleentier{2}{m+n}$, and, when the sum is minimal, $C_j^{BM}(\PB{\vect{\Delta}})$ can only take two values: 
    \begin{equation*}
    \begin{cases}
    \tilde{C}_j^{BM} = \ell_j^{-1} \left(\Esp^{(h)}\left[\sachant{X_j}{\vect{Y}}\right] - \Esp^{(h)}\left[\sachant{X_{\pa(j)}}{\vect{Y}}\right]\right)^2 & \text{if no shift on branch $b_j$} \\
    0 & \text{if one shift on branch $b_j$}
    \end{cases}
    \end{equation*}
%     either $\tilde{C}_j^{BM}(\vvect{\tau}, \vvect{\delta}) = \ell_j^{-1} \left(\Esp^{(h)}\left[\sachant{X_j}{\vect{Y}}\right] - \Esp^{(h)}\left[\sachant{X_{\pa(j)}}{\vect{Y}}\right]\right)^2$ if there is no shift on branch $b_j$, or $0$ if there is a shift of the right intensity (see below) on branch $b_j$.
    The sum can hence be minimized in the following way:
    \begin{enumerate}
     \item Compute $\tilde{C}_j^{BM}$ for all $j\in\intervalleentier{2}{m+n}$.
     \item Find the $K$ highest costs $(j_1, \cdots, j_K)\in\intervalleentier{2}{m+n}^K$.
%     \item Set $b^{(h+1)}_k = b_{j_k}$ and $\vvect{\delta}^{(h+1)}_k = \Esp^{(h)}\left[\sachant{X_j}{\vect{Y}}\right] - \Esp^{(h)}\left[\sachant{X_{\pa(j)}}{\vect{Y}}\right]$ for all $k\in\intervalleentier1K$.
     \item \PB{Set $\Delta^{(h+1)}_{j_k} = \Esp^{(h)}\left[\sachant{X_{j_k}}{\vect{Y}}\right] - \Esp^{(h)}\left[\sachant{X_{\pa(j_k)}}{\vect{Y}}\right]$ for all $k\in\intervalleentier1K$, and $\Delta^{(h+1)}_{j} = 0$ if $j \notin \{j_1, \cdots, j_K\}$.}
    \end{enumerate}
    This exact and fast algorithm works for the BM because all the costs are independent. Note that it would work for any Levy Process without memory, such as those proposed in \citet{landis2013} to model evolution of quantitative traits. %that can be used to model the evolution of a quantitative trait \citep[see][]{landis2013}
    
    \paragraph{GM Step for Shifts Locations for the OU} With $\alpha^{(h)}$ fixed, we want to minimize the sum of costs:
%        \[C^{OU}(\vvect{\tau}, \vvect{\delta}, \beta_0, \alpha^{(h)}) = \left(\Esp^{(h)}\left[\sachant{X_{1}}{\vect{Y}}\right] - \beta_0\right)^2 + \sum_{j=2}^{m+n}C_j^{OU}(\vvect{\tau}, \vvect{\delta}, \beta_0, \alpha^{(h)})\]
    \[C^{OU}(\alpha^{(h)}, \PB{\vect{\Delta}}) = \left(\Esp^{(h)}\left[\sachant{X_{1}}{\vect{Y}}\right] - \beta_0\right)^2 + \sum_{j=2}^{m+n}C_j^{OU}(\alpha^{(h)}, \PB{\vect{\Delta}})\]
    The previous algorithm does not work, because the costs are not independent. Solving the problem exactly would require to visit all the possible configurations, and the complexity would be too high, of order $O\left(\binom{m+n}{K}\right) = O(n^K)$. To reduce the execution time of the algorithm, we use heuristics to lower, if not minimize, the sum of costs. We use the following formulation:
%    \[
%     C^{OU}(\vvect{\tau}, \vvect{\delta}, \beta_0, \alpha^{(h)}) = \norm{\vect{F}^{(h)} - \matr{A}^{(h)}\matr{U}\vect{\Delta}}^2
%    \]
    \[
     C^{OU}(\alpha^{(h)}, \PB{\vect{\Delta}}) = \norm{\vect{F}^{(h)} - \matr{A}^{(h)}\matr{U}\vect{\Delta}}^2
    \]
    where 
    %$\vect{\Delta}$ is the vector of shifts described in subsection \ref{subsec:probabilistic_model}, 
    $\matr{U}$ the complete tree matrix given in subsection \ref{subsec:linear_model}, $\matr{A}^{(h)} = \Diag\left(1, \sqrt{\frac{1-e^{-\alpha^{(h)}\ell_j}}{1+e^{-\alpha^{(h)}\ell_j}}}; 2\leq j \leq m+n \right)$ a diagonal matrix depending on $\alpha^{(h)}$, and $\vect{F}^{(h)}$ a vector of expectations, with 
    $F^{(h)}_1 = \Esp^{(h)}\left[\sachant{X_{1}}{\vect{Y}}\right]$, and, for $2 \leq j \leq m+n$, \[F^{(h)}_j = \left(1-e^{-2\alpha^{(h)}\ell_j}\right)^{-1/2}\left(\Esp^{(h)}\left[\sachant{X_j}{\vect{Y}}\right] - \Esp^{(h)}\left[\sachant{X_{\pa(j)}}{\vect{Y}}\right]e^{-\alpha^{(h)}\ell_j}\right)\]
    We can then use a Lasso algorithm to impose sparsity constraints on $\vect{\Delta}$. If $\vect{\Delta}_{-1}$ is the vector of shifts without the initial value (intercept), then a Lasso estimator is given by, for $\lambda \geq 0$:
    \[
      \hat{\vect{\Delta}}_\lambda = \argmin_{\vect{\Delta}} \left\{ \norm{\vect{F}^{(h)} - \matr{A}^{(h)}\matr{U}\vect{\Delta}}^2 + \lambda \abs{\vect{\Delta}_{-1}}_1 \right\}
    \]
    The estimated vectors $\hat{\vect{\Delta}}_\lambda$ have a support that is sparser when $\lambda$ becomes higher. One then only need to find the right penalty factor $\lambda$ that ensure that the support has exactly $K$ non zero coordinates, plus the initial value. %The Lasso regression is done here thanks to an algorithm implemented in the \printR{R} package \printR{quadrupen} \citep{chiquet2012}.
We ensure that the $K$ shifts are allocated in a parsimonious way by checking their linear independence, using proposition \ref{prop:parsimony_linear_independence}.\par
    An other method is to take the previous solution $\vect{\Delta}^{(h)}$, and test all the configurations where only one shift has moved, and take the best one. In both methods, one also has to ensure that the objective function is increased by the new choice of shifts, so that the GEM algorithm works correctly. This step is generally the longest one in one iteration of the EM.

%%%%%%%%%%%%%%%%%%%%%%%%%%%%%%%%%%%%%%%%%%%%%%%%%%%%%%%%%%%%%%%%%%%%%%%
\subsection{Initialization}\label{supp:initialization}
Initialization is always a crucial step when using an EM algorithm. The vector of shifts $\vect{\Delta}$ is initialized thanks to a Lasso procedure. To do that, we use the linear formulation \ref{eq:BM_lin_def_X} or \ref{eq:OU_lin_def} of the main text, and we calibrate the penalty so that the initialization vector has a non zero first coordinate (initial value), and $K$ other non-zero coordinates. The variance-covariance matrix is initialized with defaults parameters, and is taken into account thanks to a Cholesky decomposition.\par
    We also initialize the selection strength $\alpha$. We use the following property: if $Y_i$ and $Y_j$ are two tips in the same group, then, under an OUsun, \( \Espe{(Y_i-Y_j)^2} = 2\gamma^2(1-e^{-\alpha d_{ij}}) \). Using regression techniques, we can get an initial estimation of $\alpha$ and $\gamma^2$ from all these couples. In practice, we first initialize the position of the shifts, and then use only pairs of tips from the same estimated group. Then, as the groups are only approximated, some of the selected pairs $(Y_i, Y_j)$ might not share the same expectation, and we use a robust regression to get more accurate initial estimates.
