# Supplementary material for: Detection of adaptive shifts on phylogenies using shifted stochastic processes on a tree
Source: arXiv:1508.00225 source file (2016-07-13)
Supplement: Supplementary file 7 [file supplementary_figures.tex]

%%%%%%%%%%%%%%%%%%%%%%%%%%%%%%%%%%%%%%%%%%%%%%%%%%%%%%%%%%%%%%%%%%%%%%%
%%%%%%%%%%%%%%%%%%%%%%%%%%%%%%%%%%%%%%%%%%%%%%%%%%%%%%%%%%%%%%%%%%%%%%%
\section{Supplementary Figures} \label{supp:SimulationAnalysis}
%%%%%%%%%%%%%%%%%%%%%%%%%%%%%%%%%%%%%%%%%%%%%%%%%%%%%%%%%%%%%%%%%%%%%%%
%%%%%%%%%%%%%%%%%%%%%%%%%%%%%%%%%%%%%%%%%%%%%%%%%%%%%%%%%%%%%%%%%%%%%%%

%%%%%%%%%%%%%%%%%%%%%%%%%%%%%%%%%%%%%%%%%%%%%%%%%%%%%%%%%%%%%%%%%%%%%%%
%%% Definition of Knitr
%%%%%%%%%%%%%%%%%%%%%%%%%%%%%%%%%%%%%%%%%%%%%%%%%%%%%%%%%%%%%%%%%%%%%%%

%%%%%%%%%%%%%%%%%%%%%%%%%%%%%%%%%%%%%%%%%%%%%%%%%%%%%%%%%%%%%%%%%%%%%%%

  %%%%%%%%%%%%%%%%%%%%%%%%%%%%%%%%%%%%%
  \subsection{Simulation Study: Sensitivity and False Positive Rate}
    \paragraph{Definition of the Scores}
    We denote by $TP$ the number of True Positives, i.e. the predicted edges on which a shift actually occurred, and $FP$ the number of False Positives.
    The sensitivity $\frac{TP}{K_t}$ is the proportion of well predicted shifts among all shifts to be predicted, and the False Positive Rate (FPR) $\frac{FP}{n + m - K_t}$ is the proportion of false positive among all edges with no shifts.\par
    Note that here, due to the possible lack of identifiability, the position of the shifts on the tree is not well defined, as a shift can be on a particular edge for one of the equivalent solutions, but not on the others (see Section \ref{subsec:identifiability}). These two scores are hence ill defined for our problem. To avoid such problems, we restrict ourselves to the $91\%$ of unambiguous configurations \PB{that occurred during the simulations}.
    %Here, $TP$ denotes the True Positives (predicted edges on which a shift actually occurred) and $FP$, $TN$, $FN$, respectively, the False Positive, True Negative, False Negative. We have $TP + FN = K_t$ the true number of shifts, and $FP + TN = n + m - 1 - K_t$ the number of edges without any shift. Similarly, $TP + FP = K_s$ the selected number of shifts, and $FN + TN = n+m-1-K_s$ the number of edges without predicted shifts.
%     \begin{itemize}
%     \item The sensitivity : $\frac{TP}{K_t}$ (proportion of well predicted shifts among all shifts to be predicted)
%     \item The False Positive Rate (FPR) : $\frac{FP}{n + m - K_t}$ (proportion of false positive among all edges with no shifts). %FPR = 1 - specificity.
%     \end{itemize}

\paragraph{Interpretation of Results}
 Figure \ref{simus:fpr} shows that the FPR are systematically worse when using the true number of shifts, indicating that the additional shifts found when compared to the selected number are misplaced. The FPR remains very low, as only a small number of shifts is to be found. Unsurprisingly, the Sensitivity is on the contrary improved when taking the real number of shifts, as shown Figure \ref{simus:sensitivity}. In addition, the sensitivity is highly degraded when $\alpha$ is small or $\gamma^2$ is high, but does not exhibit a clear tendency in the real number of shifts, and the knowledge of the true value of $\alpha$ does not seem to matter.
    
    \begin{figure}[hp]
    \begin{center}
\begin{knitrout}
\definecolor{shadecolor}{rgb}{0.969, 0.969, 0.969}\color{fgcolor}
\includegraphics[width=\maxwidth,height=0.4\textheight]{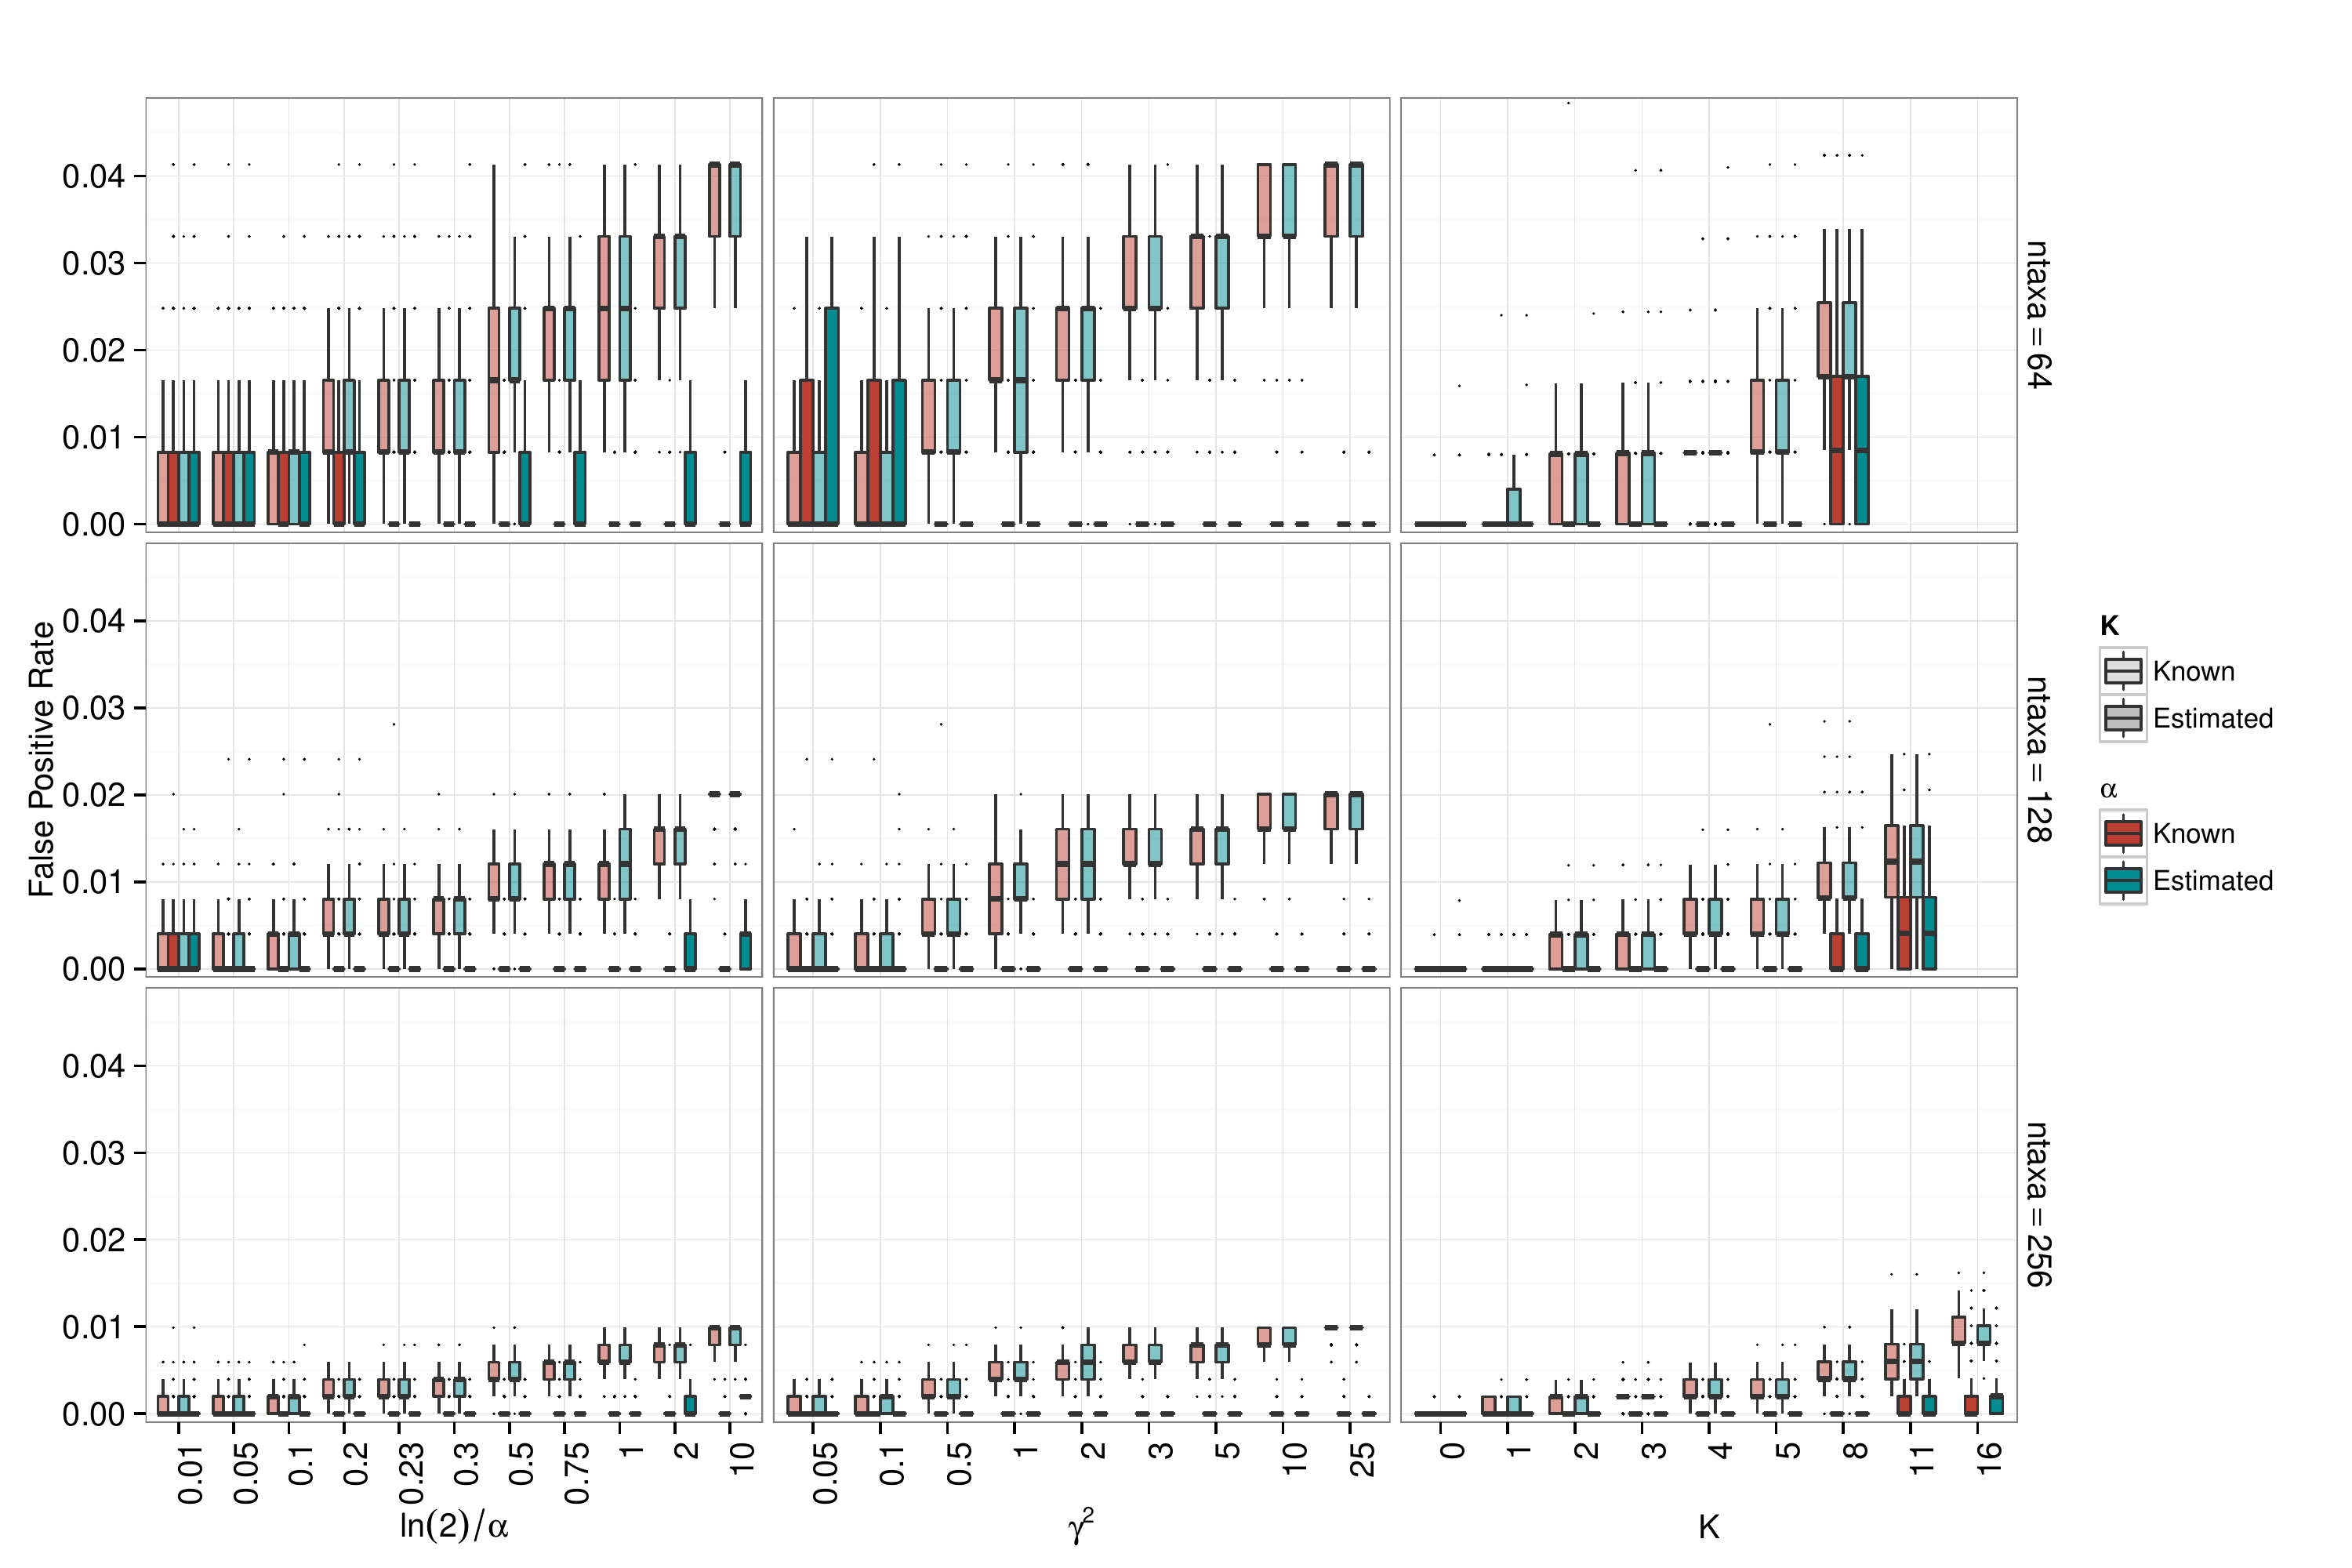} 

\end{knitrout}
    \caption{False Positive Rate computed for the different configurations. Note the $y$ scale, that only goes to $0.05$.}\label{simus:fpr}
    \end{center}

    \begin{center}
\begin{knitrout}
\definecolor{shadecolor}{rgb}{0.969, 0.969, 0.969}\color{fgcolor}
\includegraphics[width=\maxwidth,height=0.4\textheight]{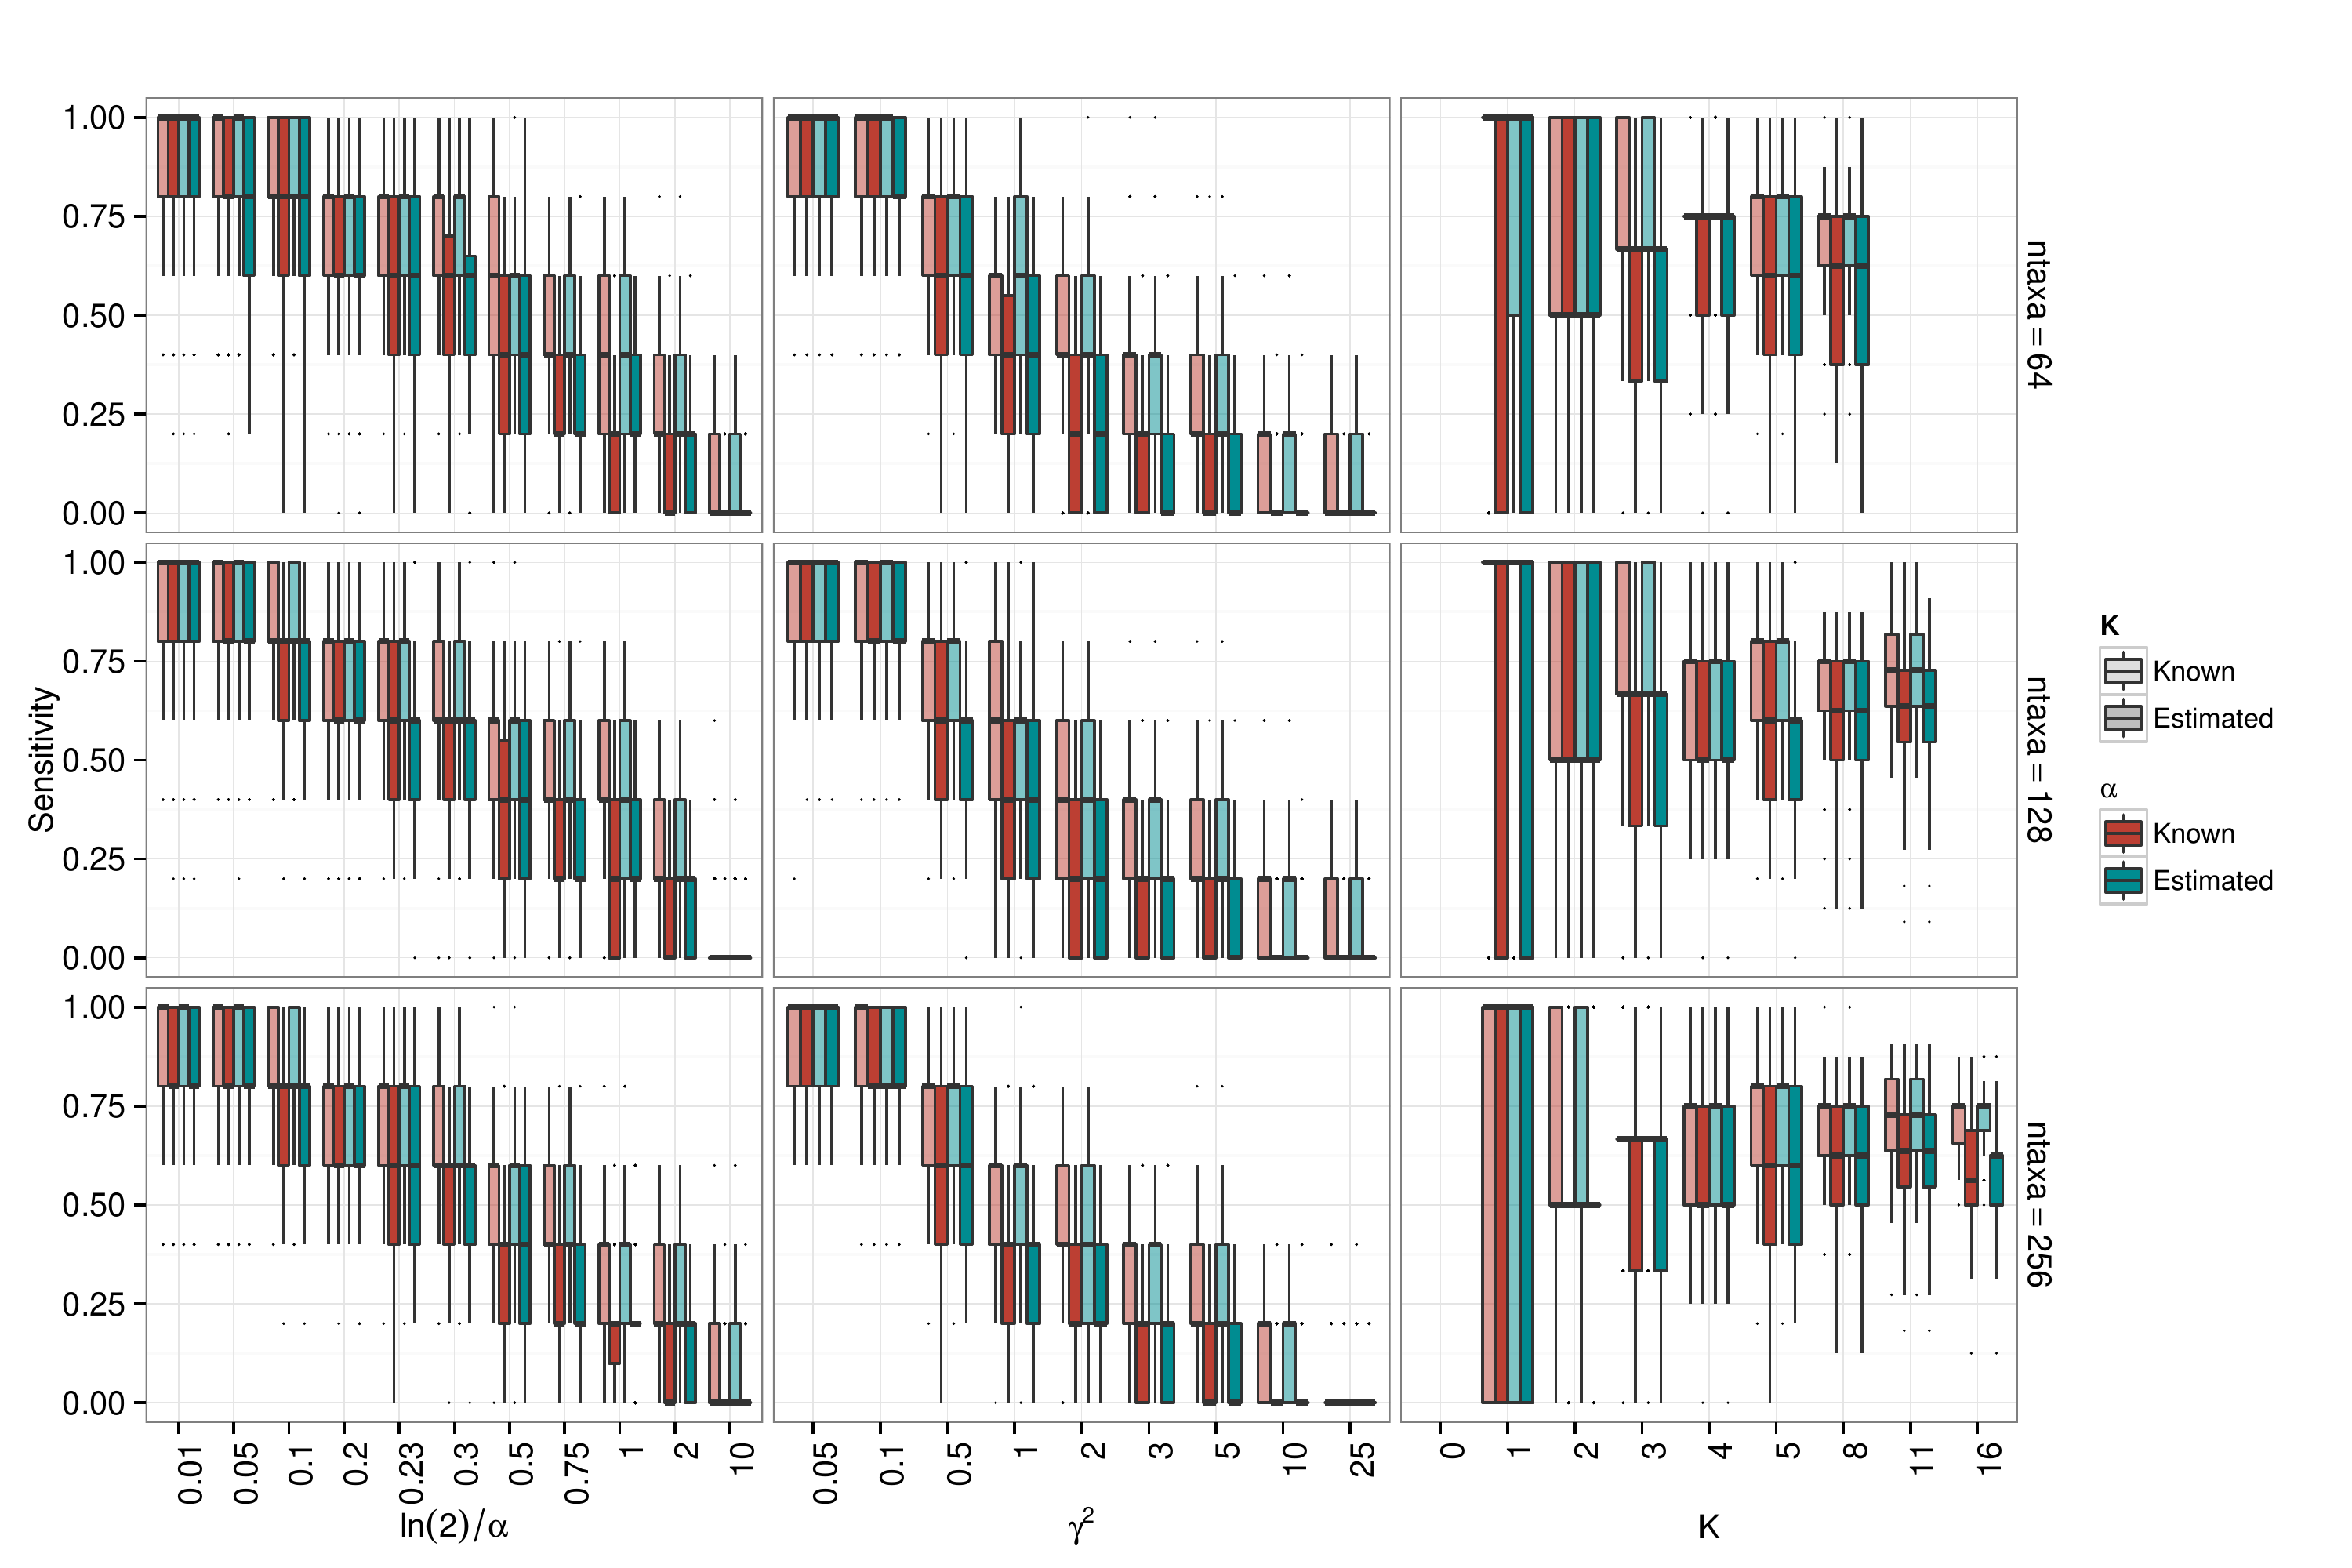} 

\end{knitrout}
    \caption{Sensitivity computed for the different configurations, with box-plots over the repetitions. 
    %The line represents a smoothing thanks to a local polynomial regression fitting.
    }\label{simus:sensitivity}
    \end{center}
    \end{figure}
    
%%%%%%%%%%%%%%%%%%%%%%%%%%%%%%%%%%%%%%%%%%%%%%%%%%%%%%%%%%%%%%%%%%%%%%%%%%%%%%%%%%
 \subsection{Simulation Study: Complementary Analysis}
 To complete the analysis conducted in the main text, 
 %we present here the \comment{complementary} plots of Figures~\ref{fig:ll_t_gamma} and~\ref{fig:beta_K_ARI}. Here, 
 Figure~\ref{fig:ll_t_gamma_rev} presents the variations of the log-likelihood, phylogenetic half-life, and root variance when $\alpha$ is estimated, and the number of shifts is known or estimated. We can see here that the likelihood is slightly higher when the number of shifts is fixed, which is coherent with the behavior of our model selection procedure, that tends to under-estimate the true number of shifts (see Figure~\ref{fig:beta_K_ARI} of the main text). We also note that knowing the true number of shifts has not a great influence on the estimation of $\alpha$ and $\gamma$, making the later worse, if anything.\par
 
 Figure~\ref{fig:beta_K_ARI_rev} shows the variations of the estimations of $\beta_1$, the number of shifts and the ARI when the number of shifts is estimated, and $\alpha$ is fixed or estimated. This confirms our earlier statement, that not knowing $\alpha$ with precision does not have a great impact on the model selection procedure \citep[see also][]{cressler2015}.
 
 \begin{figure}[hp]
\begin{center}

\includegraphics[width=\linewidth]{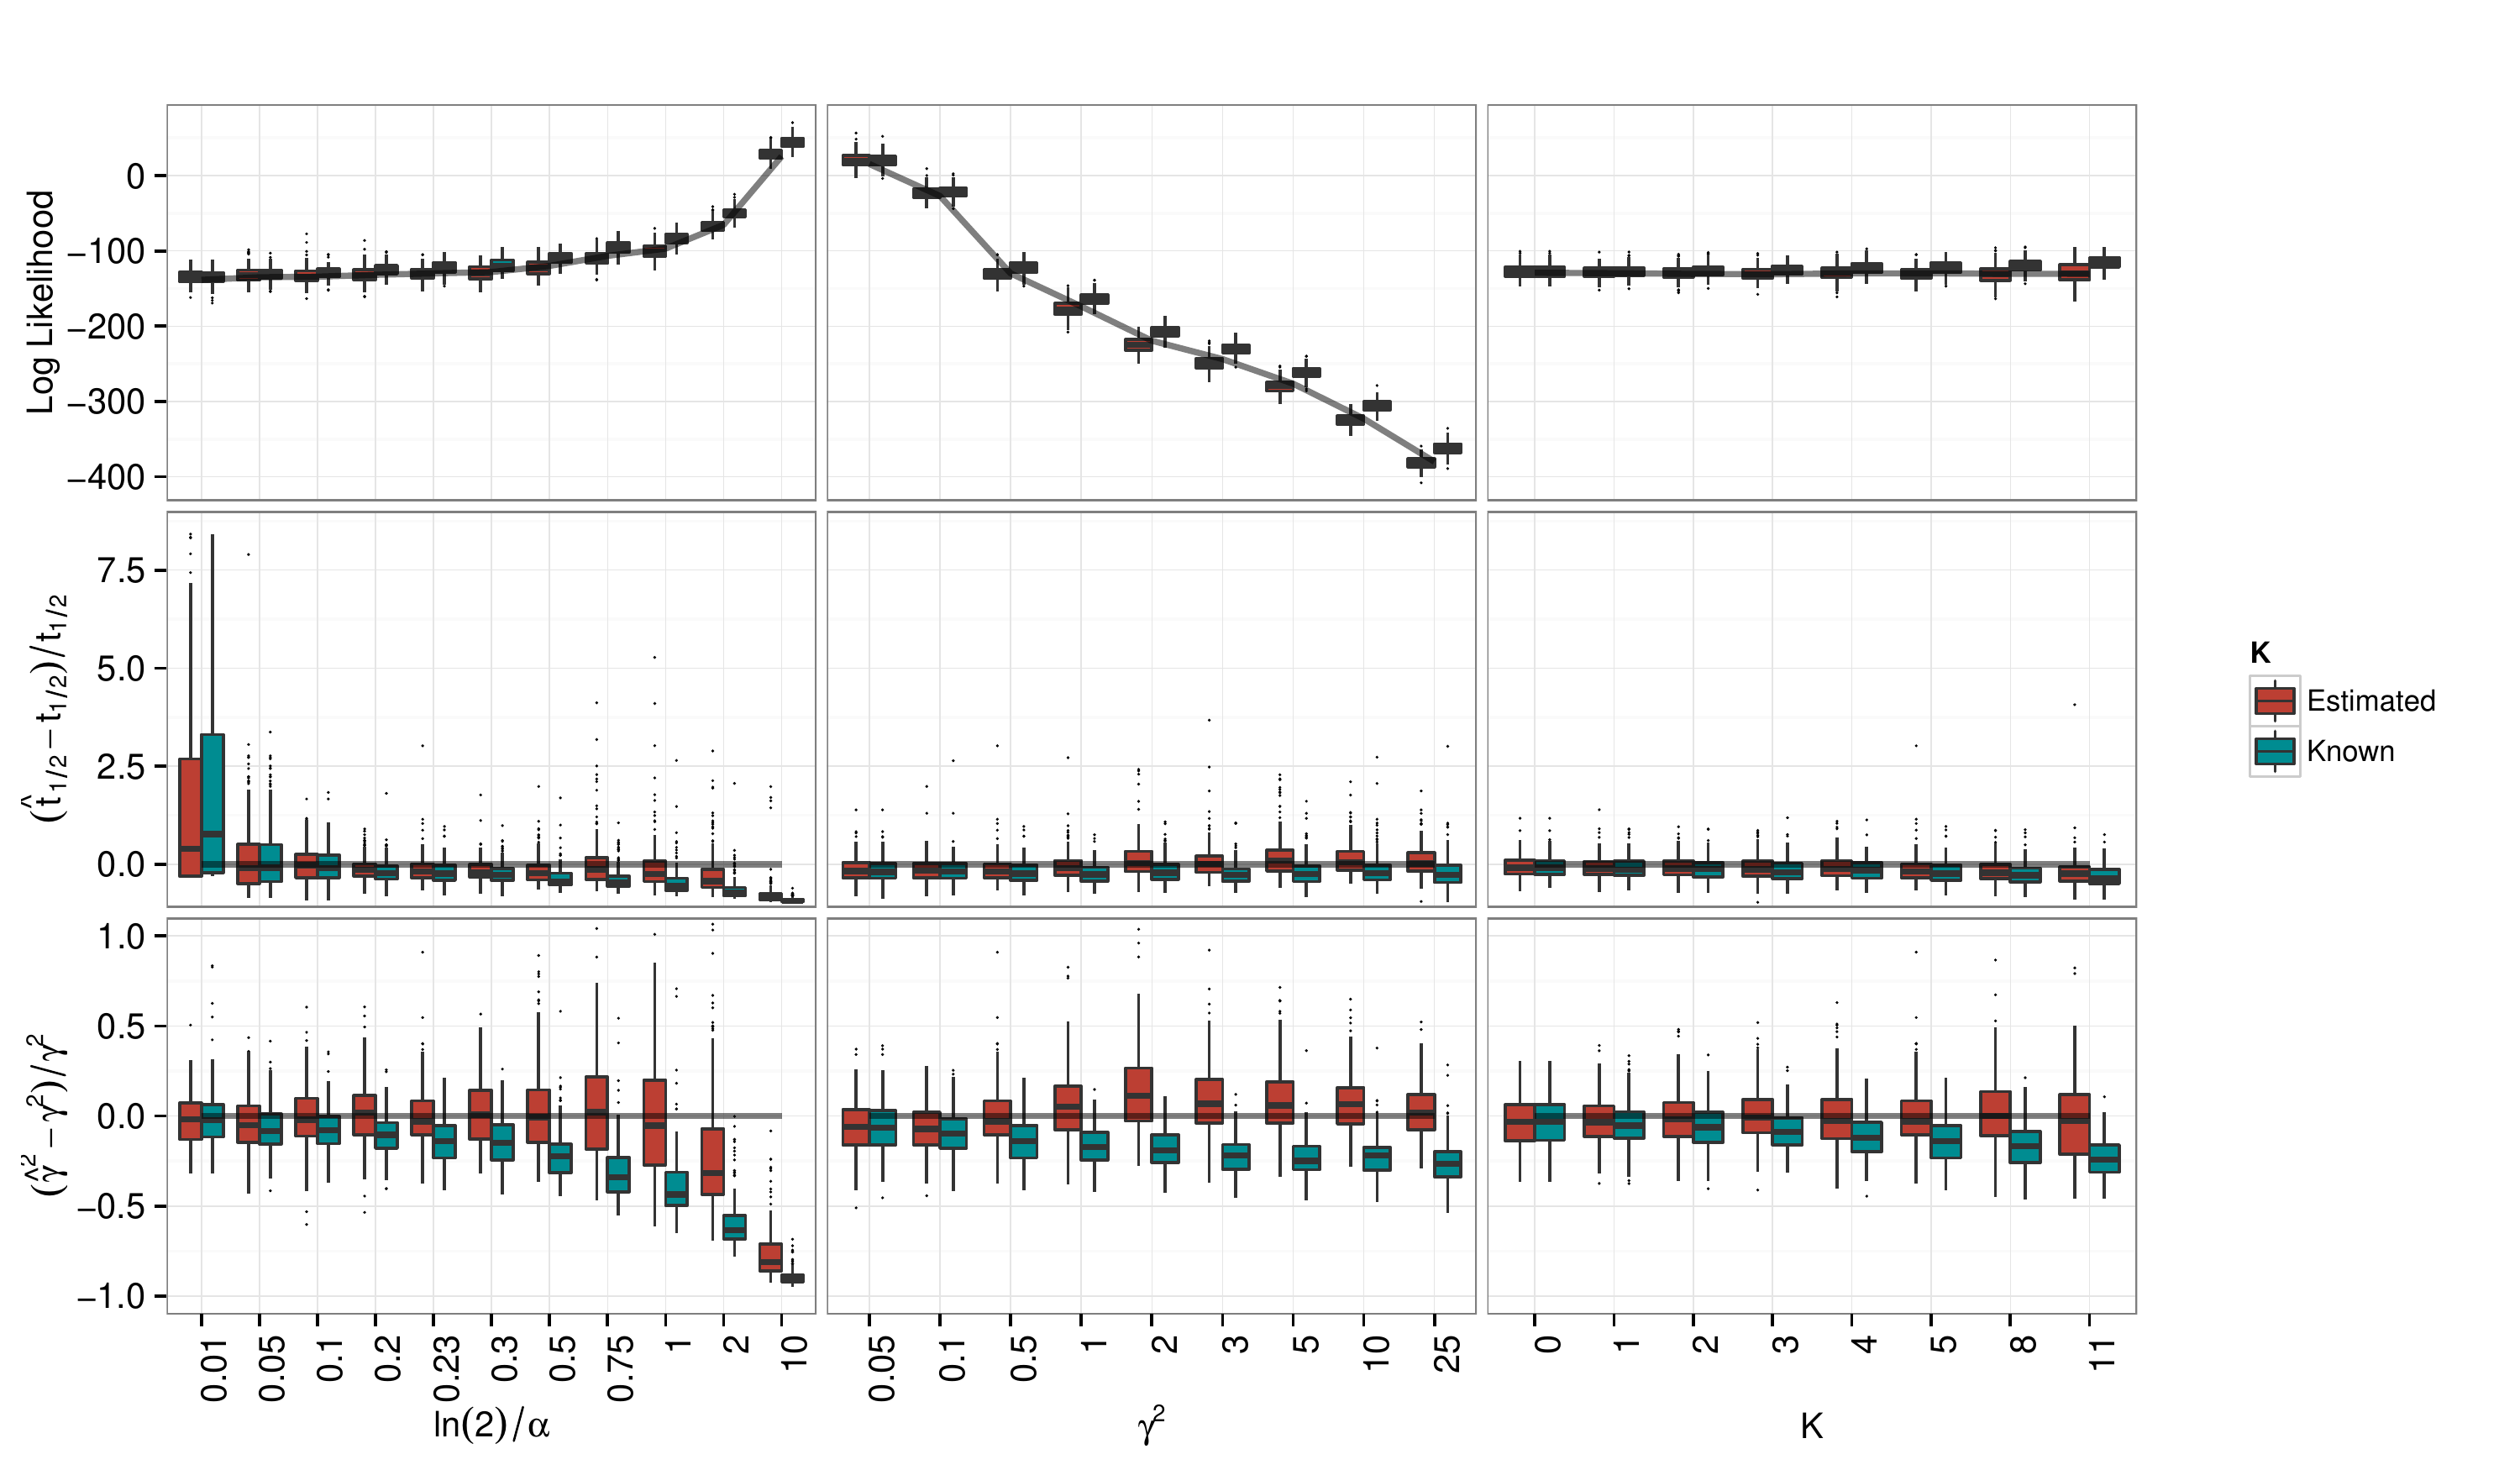} 

\caption{Box plots over the $200$ repetitions of each set of parameters, for the log-likelihood (top), phylogenetic half-life (middle) and root variance (bottom) with $\alpha$ estimated, and $K$ fixed or estimated, on a tree with $128$ taxa.}\label{fig:ll_t_gamma_rev}
\end{center}

\begin{center}

\includegraphics[width=\linewidth]{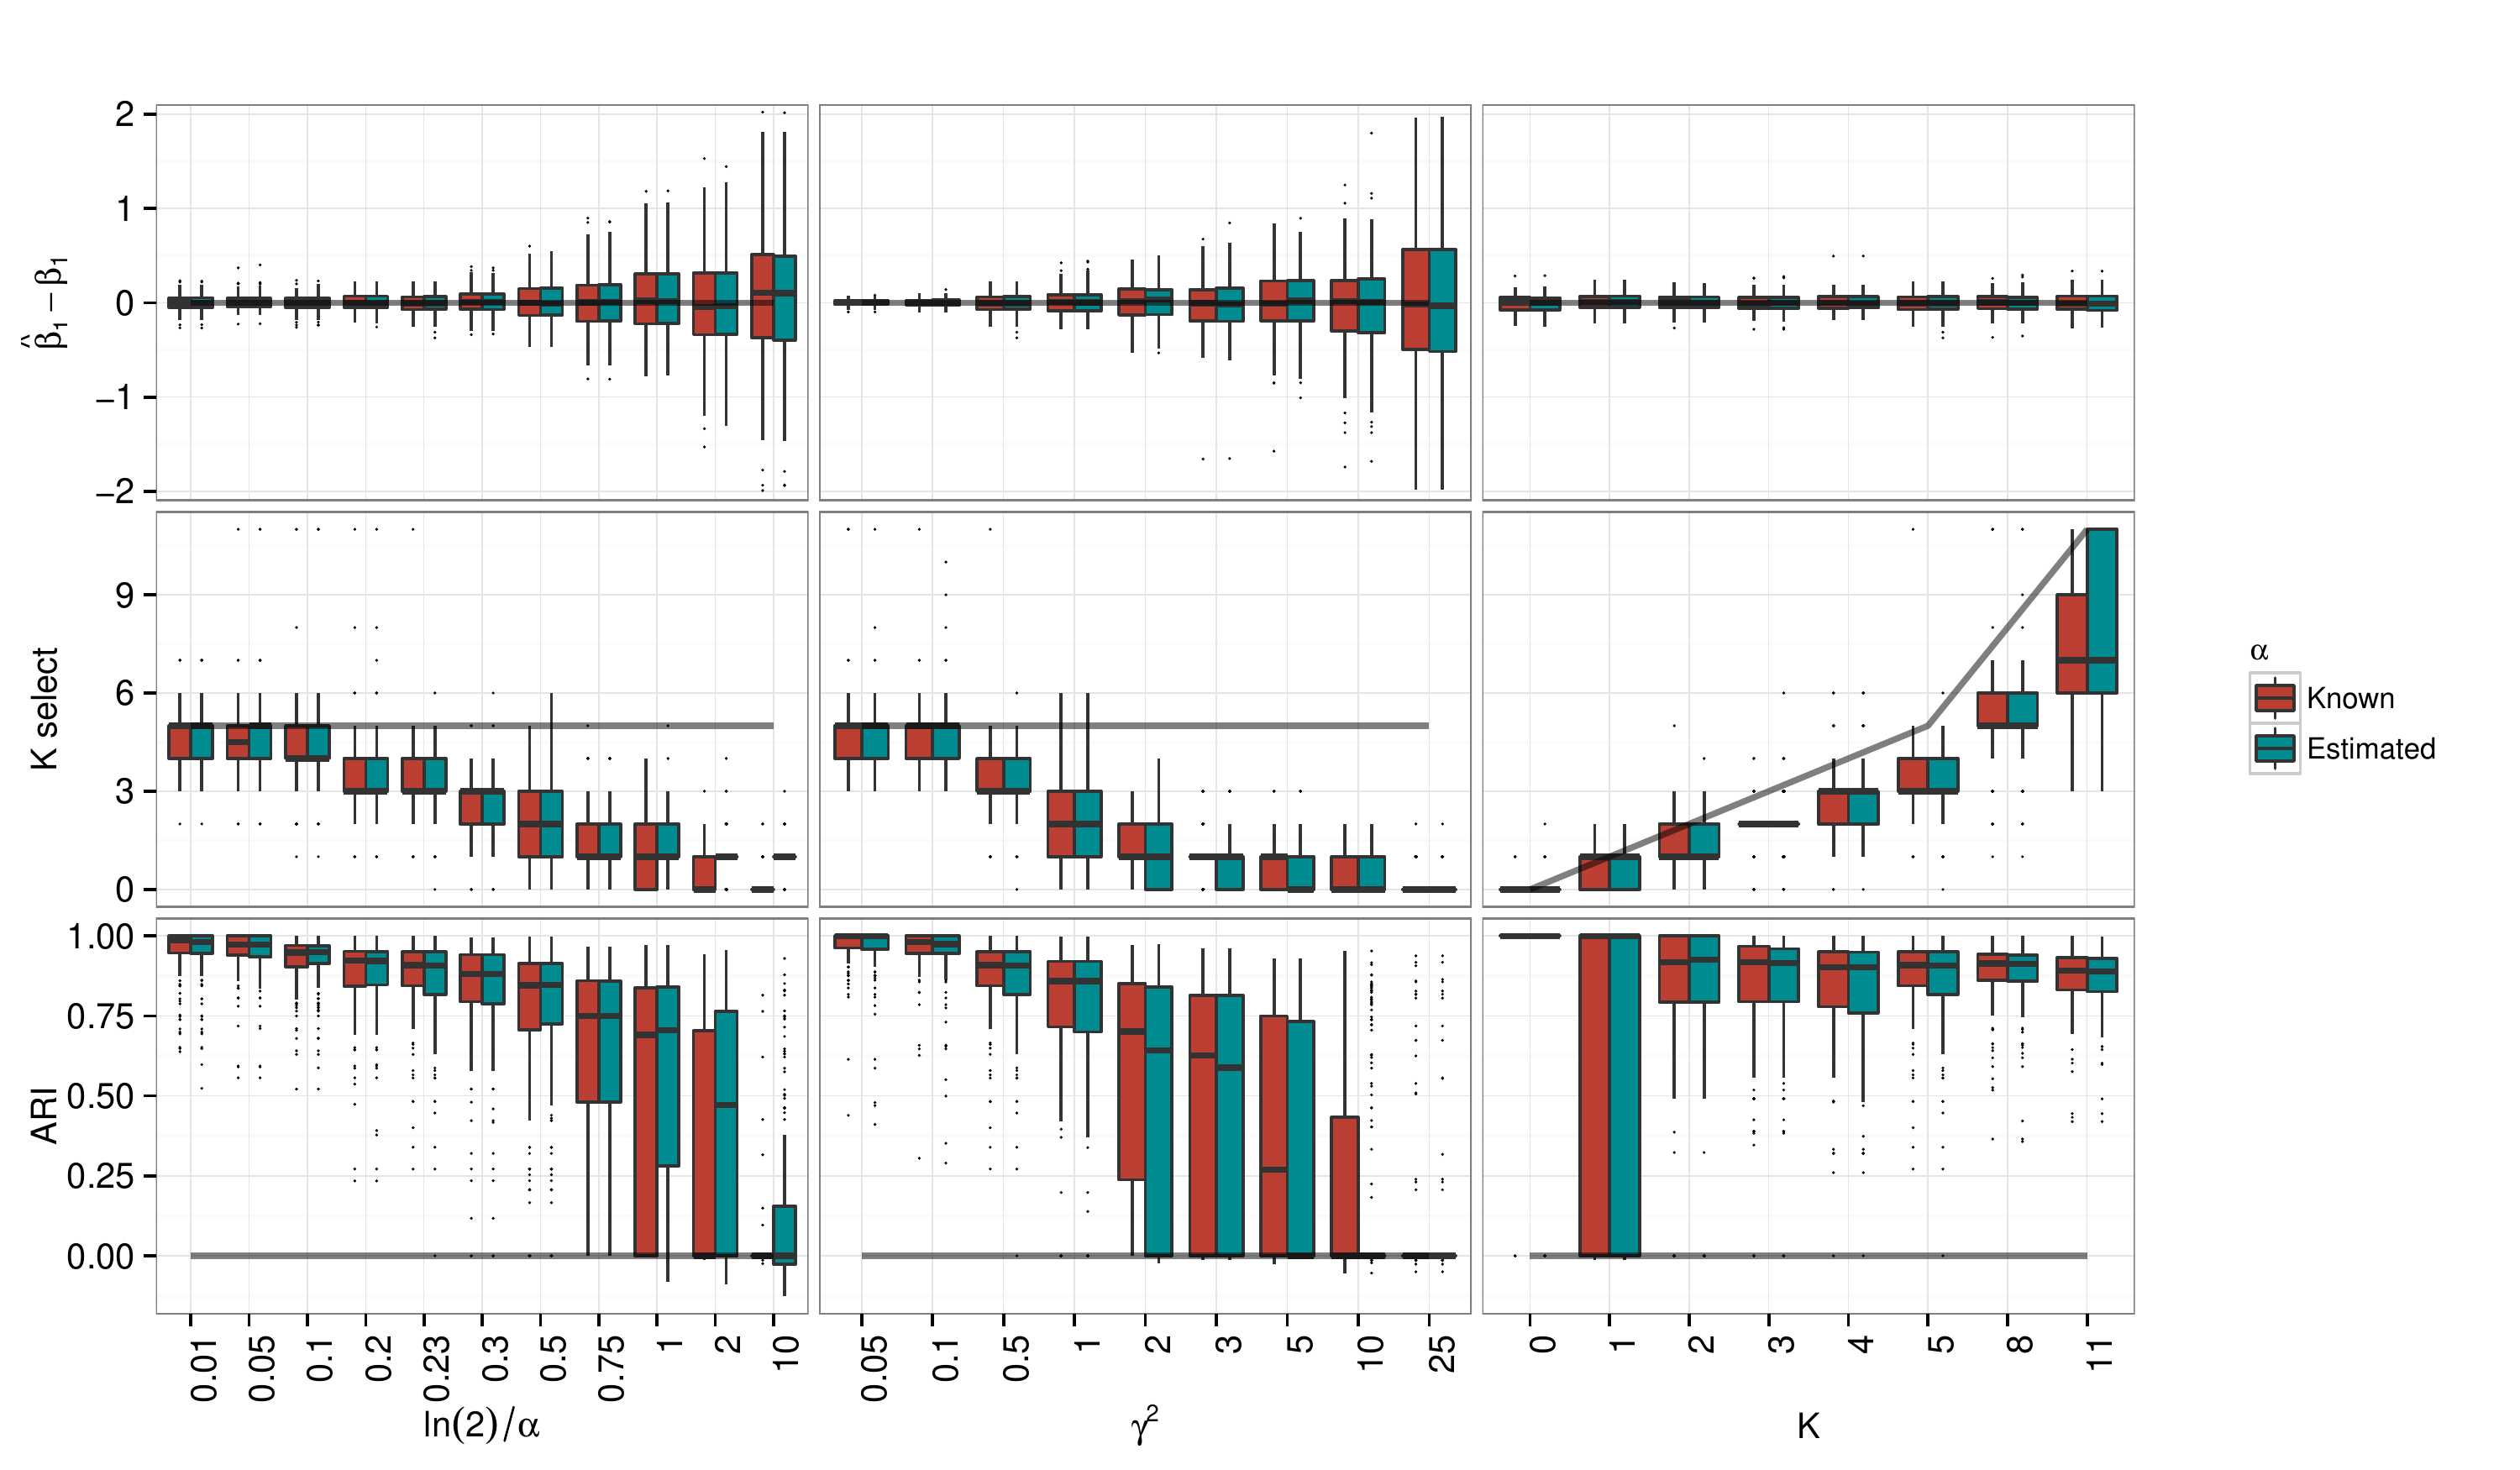} 

\caption{Same for $\beta_1$ (top), the number of shifts (middle) and ARI (bottom), with $K$ estimated, and $\alpha$ fixed or estimated.}
%Box plots for $\beta_1$ (top), the number of shifts (middle) and ARI (bottom) with the number of shifts fixed or estimated, on a tree with $128$ taxa.}
\label{fig:beta_K_ARI_rev}
\end{center}
\begin{flushleft}
For better legibility, strips with $t_{1/2}$, $\gamma^2$ and $\beta_1$ on these two figures were re-scaled, omitting some outliers (respectively, $0.21\%$, $0.27\%$ and $0.27\%$ of points are omitted). The whisker of the first box for $t_{1/2}$ goes up to $7.5$.
\end{flushleft}
\end{figure}
 
 %%%%%%%%%%%%%%%%%%%%%%%%%%%%%%%%%%%%%%%%%%%%%%%%%%%%%%%%%%%%%%%%%%%%%%%%%%%%%%%%%
 \subsection{Chelonia Dataset: Comparison of Inferred Shift Locations}\label{supp:chelonia}

  On Figure~\ref{fig:chelonia_sol_bayou}, we present and compare the shift locations found by our method, and methods \printR{bayou} and \printR{SURFACE}. The differences found are explored deeper in the main text (Section~\ref{sec:chelonia_comparison}).
 
 \paragraph{Details on the methods} In this paragraph, we give more details on the $4$ already existing methods that we compared to ours in the dataset.
 We first fitted an OU$_{habitat}$ model with fixed regimes as in \citet{jaffe2011}, using the \printR{R} package \printR{OUwie} \citep{beaulieu2012}. We tested all of the $48$ possible ways of allocating internal nodes, and took the solution with the highest likelihood. Using the package \printR{bayou} \citep{uyeda2014}, we reproduced the Bayesian analysis of the data, using two independent chains of $500000$ generations each, discarding the first $150000$ generations as burning. We assigned the priors that were used in the original study on the parameters, namely: $P(\alpha) \sim \text{LogNormal}(\ln \mu = -5, \ln \sigma = 2.5)$, $P(\sigma^2)\sim \text{LogNormal}(\ln \mu = 0, \ln \sigma = 2)$, $P(\beta_i)\sim \text{Normal}(\mu = 3.5, \sigma = 1.5)$, $P(K)\sim \text{Conditional Poisson}(\lambda = 15, K_{max} = 113)$. The computations took around $2.3$ hours of CPU time.
  \PB{We also} ran the stepwise-AIC method \citeR{SURFACE}, that relies on a forward-backward procedure. This took around $11$ hours of CPU time.
  \PB{Finally, we ran the function \printR{OUshifts} from the package \printR{phylolm}, that uses a modified BIC criterion and a heuristic stepwise procedure to detect shifts \citep{hoane2014}. Thanks to an efficient linear algorithm, detailed in \citet{hoane2013b}, this function is pretty fast, taking only about $8$ minutes of CPU time.}
  Note that the model used in these last \PB{three} methods (\printR{bayou}, \printR{SURFACE} and \printR{OUshifts}) are slightly different from ours, as they assume that the root is fixed to the ancestral optimum state, 
%  and not \PB{randomly drawn} in the stationary state.\par
\PB{and not drawn from its stationary distribution.} \par
 
   \paragraph{Note on Computation Times}
   We found that the running time for our method was similar to the running time of previous algorithms (see Table~\ref{table:chelonia} in the main text). However, our computations can be highly parallelized, as each run for a fixed number of shift is independent from the others.
  %Using \printR{R} packages \citeR{foreach} and \citeR{doParallel}, this can be easily done.
  For instance, in the previous example, the computation time could be divided by $6$, each estimation for a fixed $\alpha$ running on a different core. On the contrary, the \printR{SURFACE} method cannot be parallelized at all, and only independent chains can be parallelized for Bayesian methods, so that the computation time can only be divided by $2$ in our example.
  
 \begin{figure}[!hp]
    \begin{center} 
        \begin{minipage}{0.45\textwidth}

\includegraphics[width=\maxwidth,height=0.45\textheight]{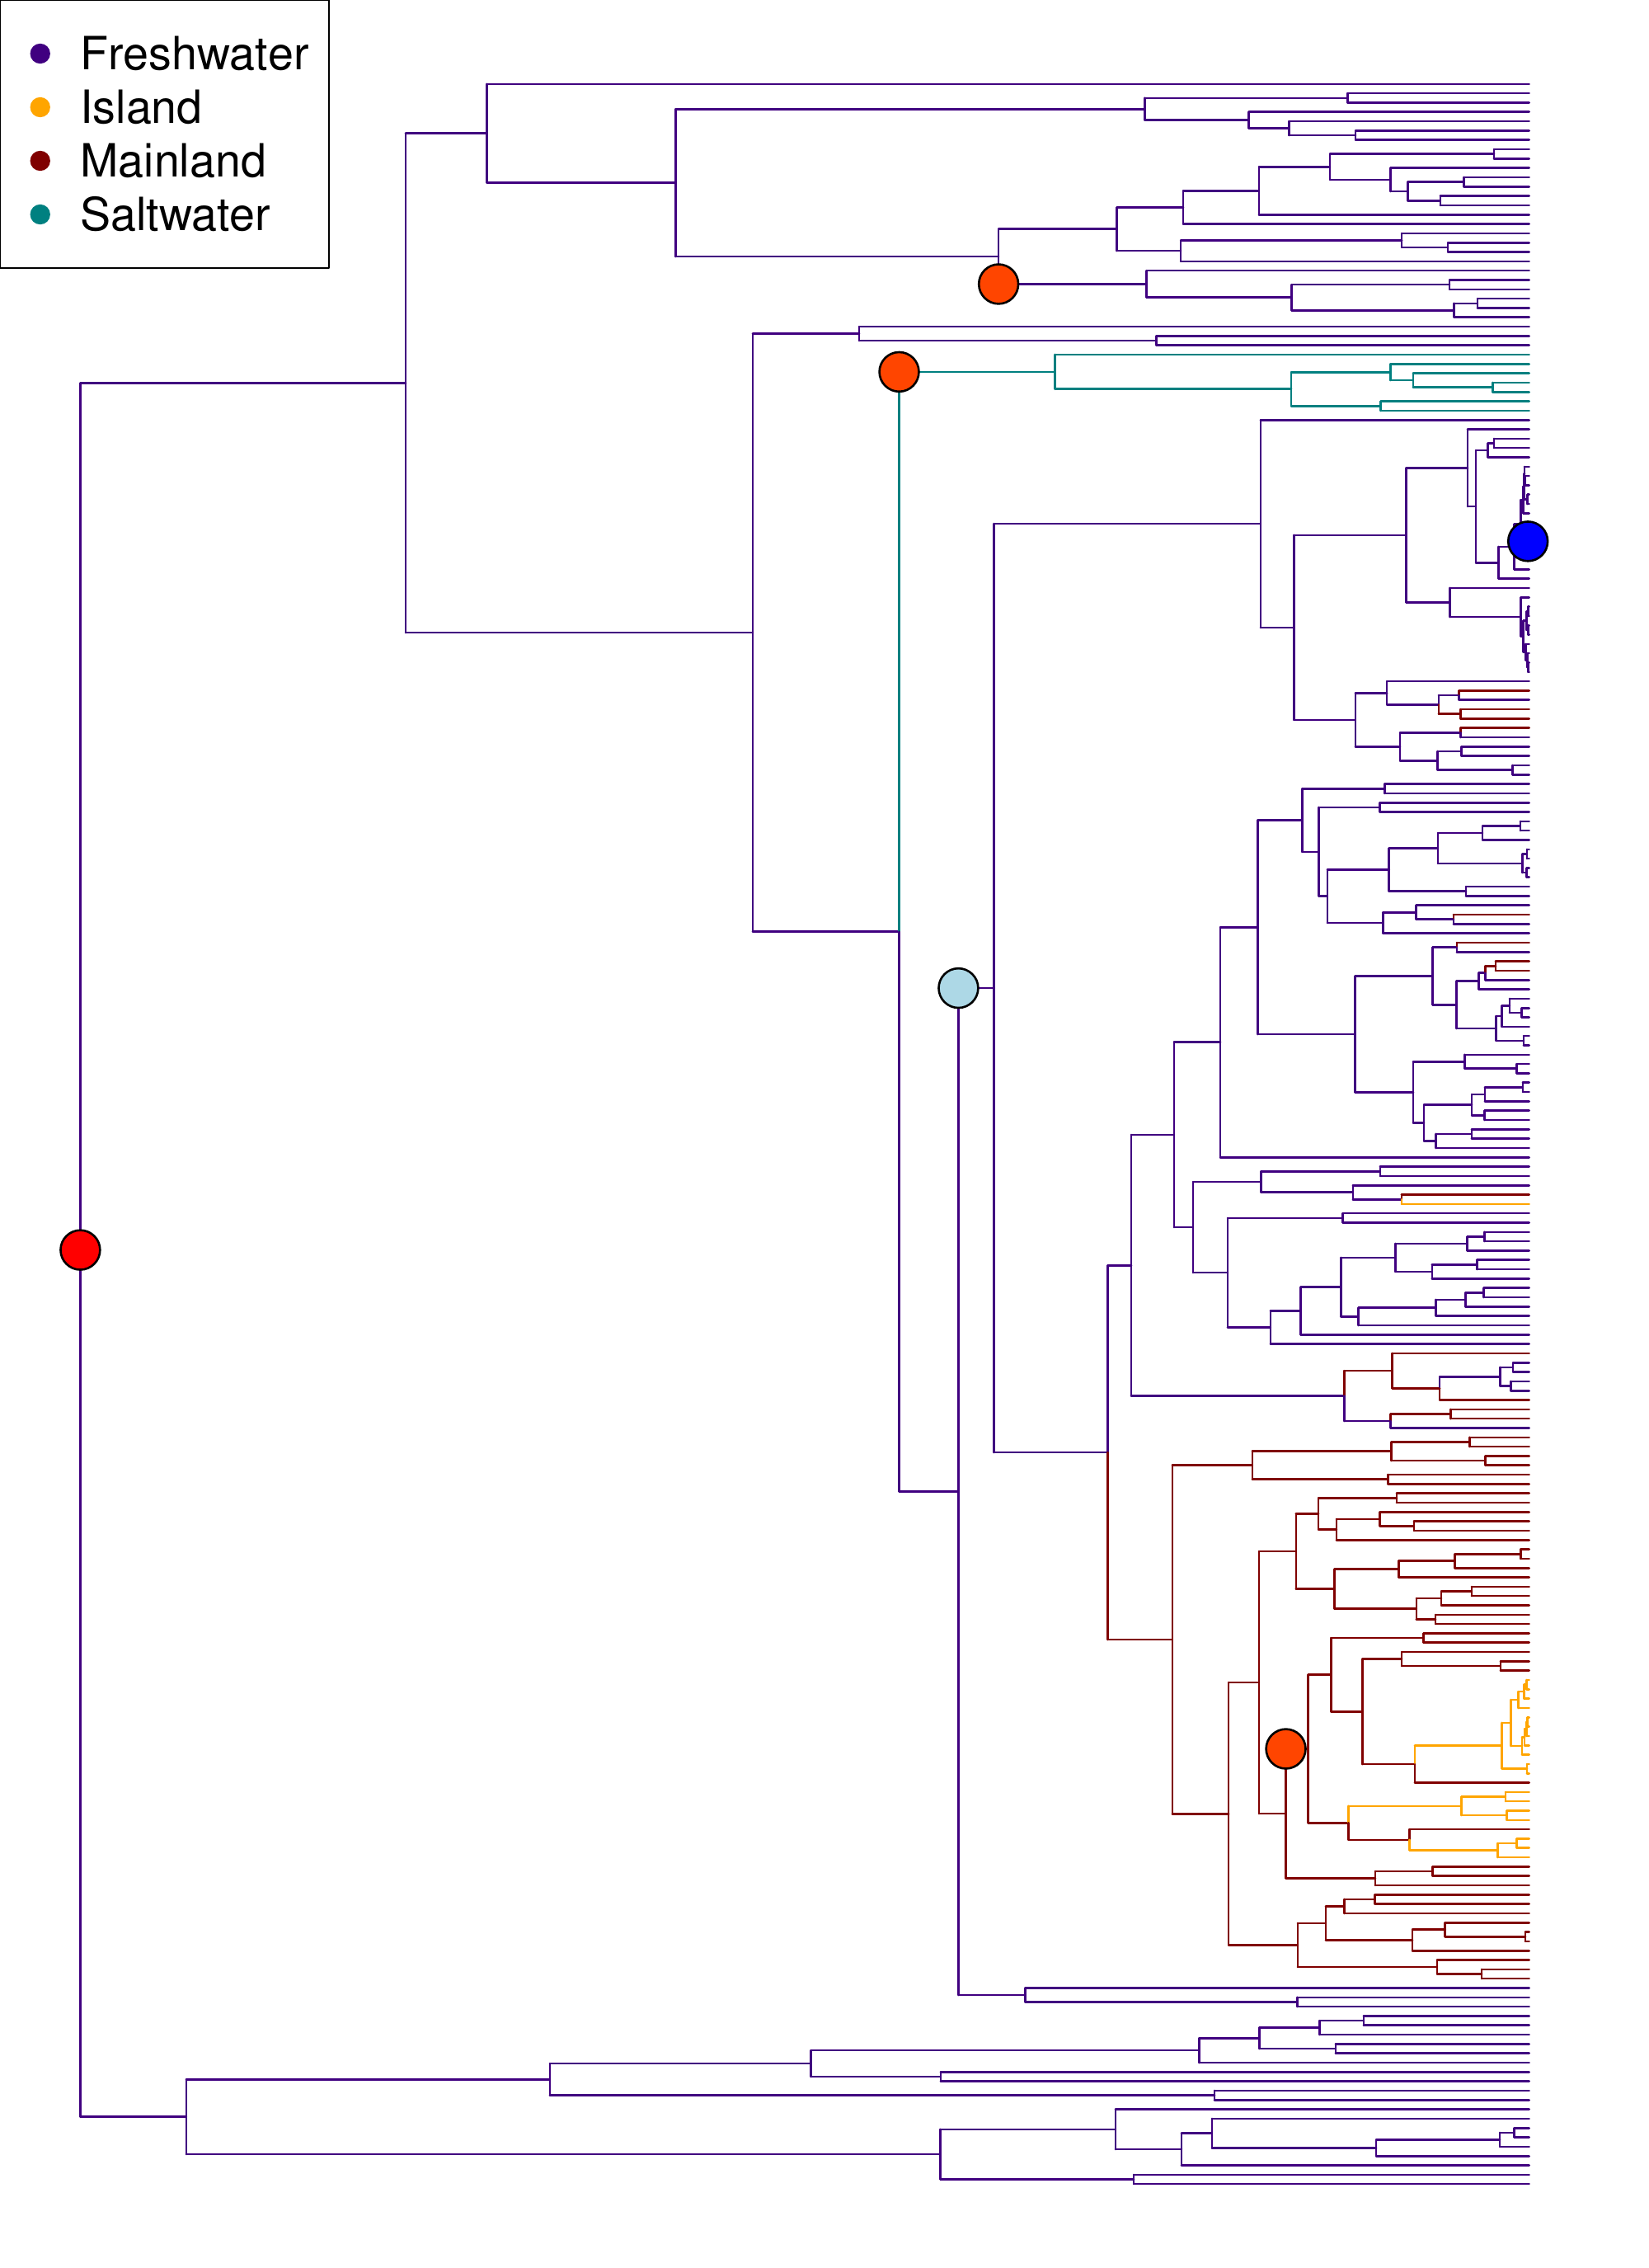} 

     {\sf \vskip -0.5cm \qquad EM}
    \end{minipage}
% \vskip - 0.5 cm
    \begin{minipage}{0.45\textwidth}

\includegraphics[width=\maxwidth,height=0.45\textheight]{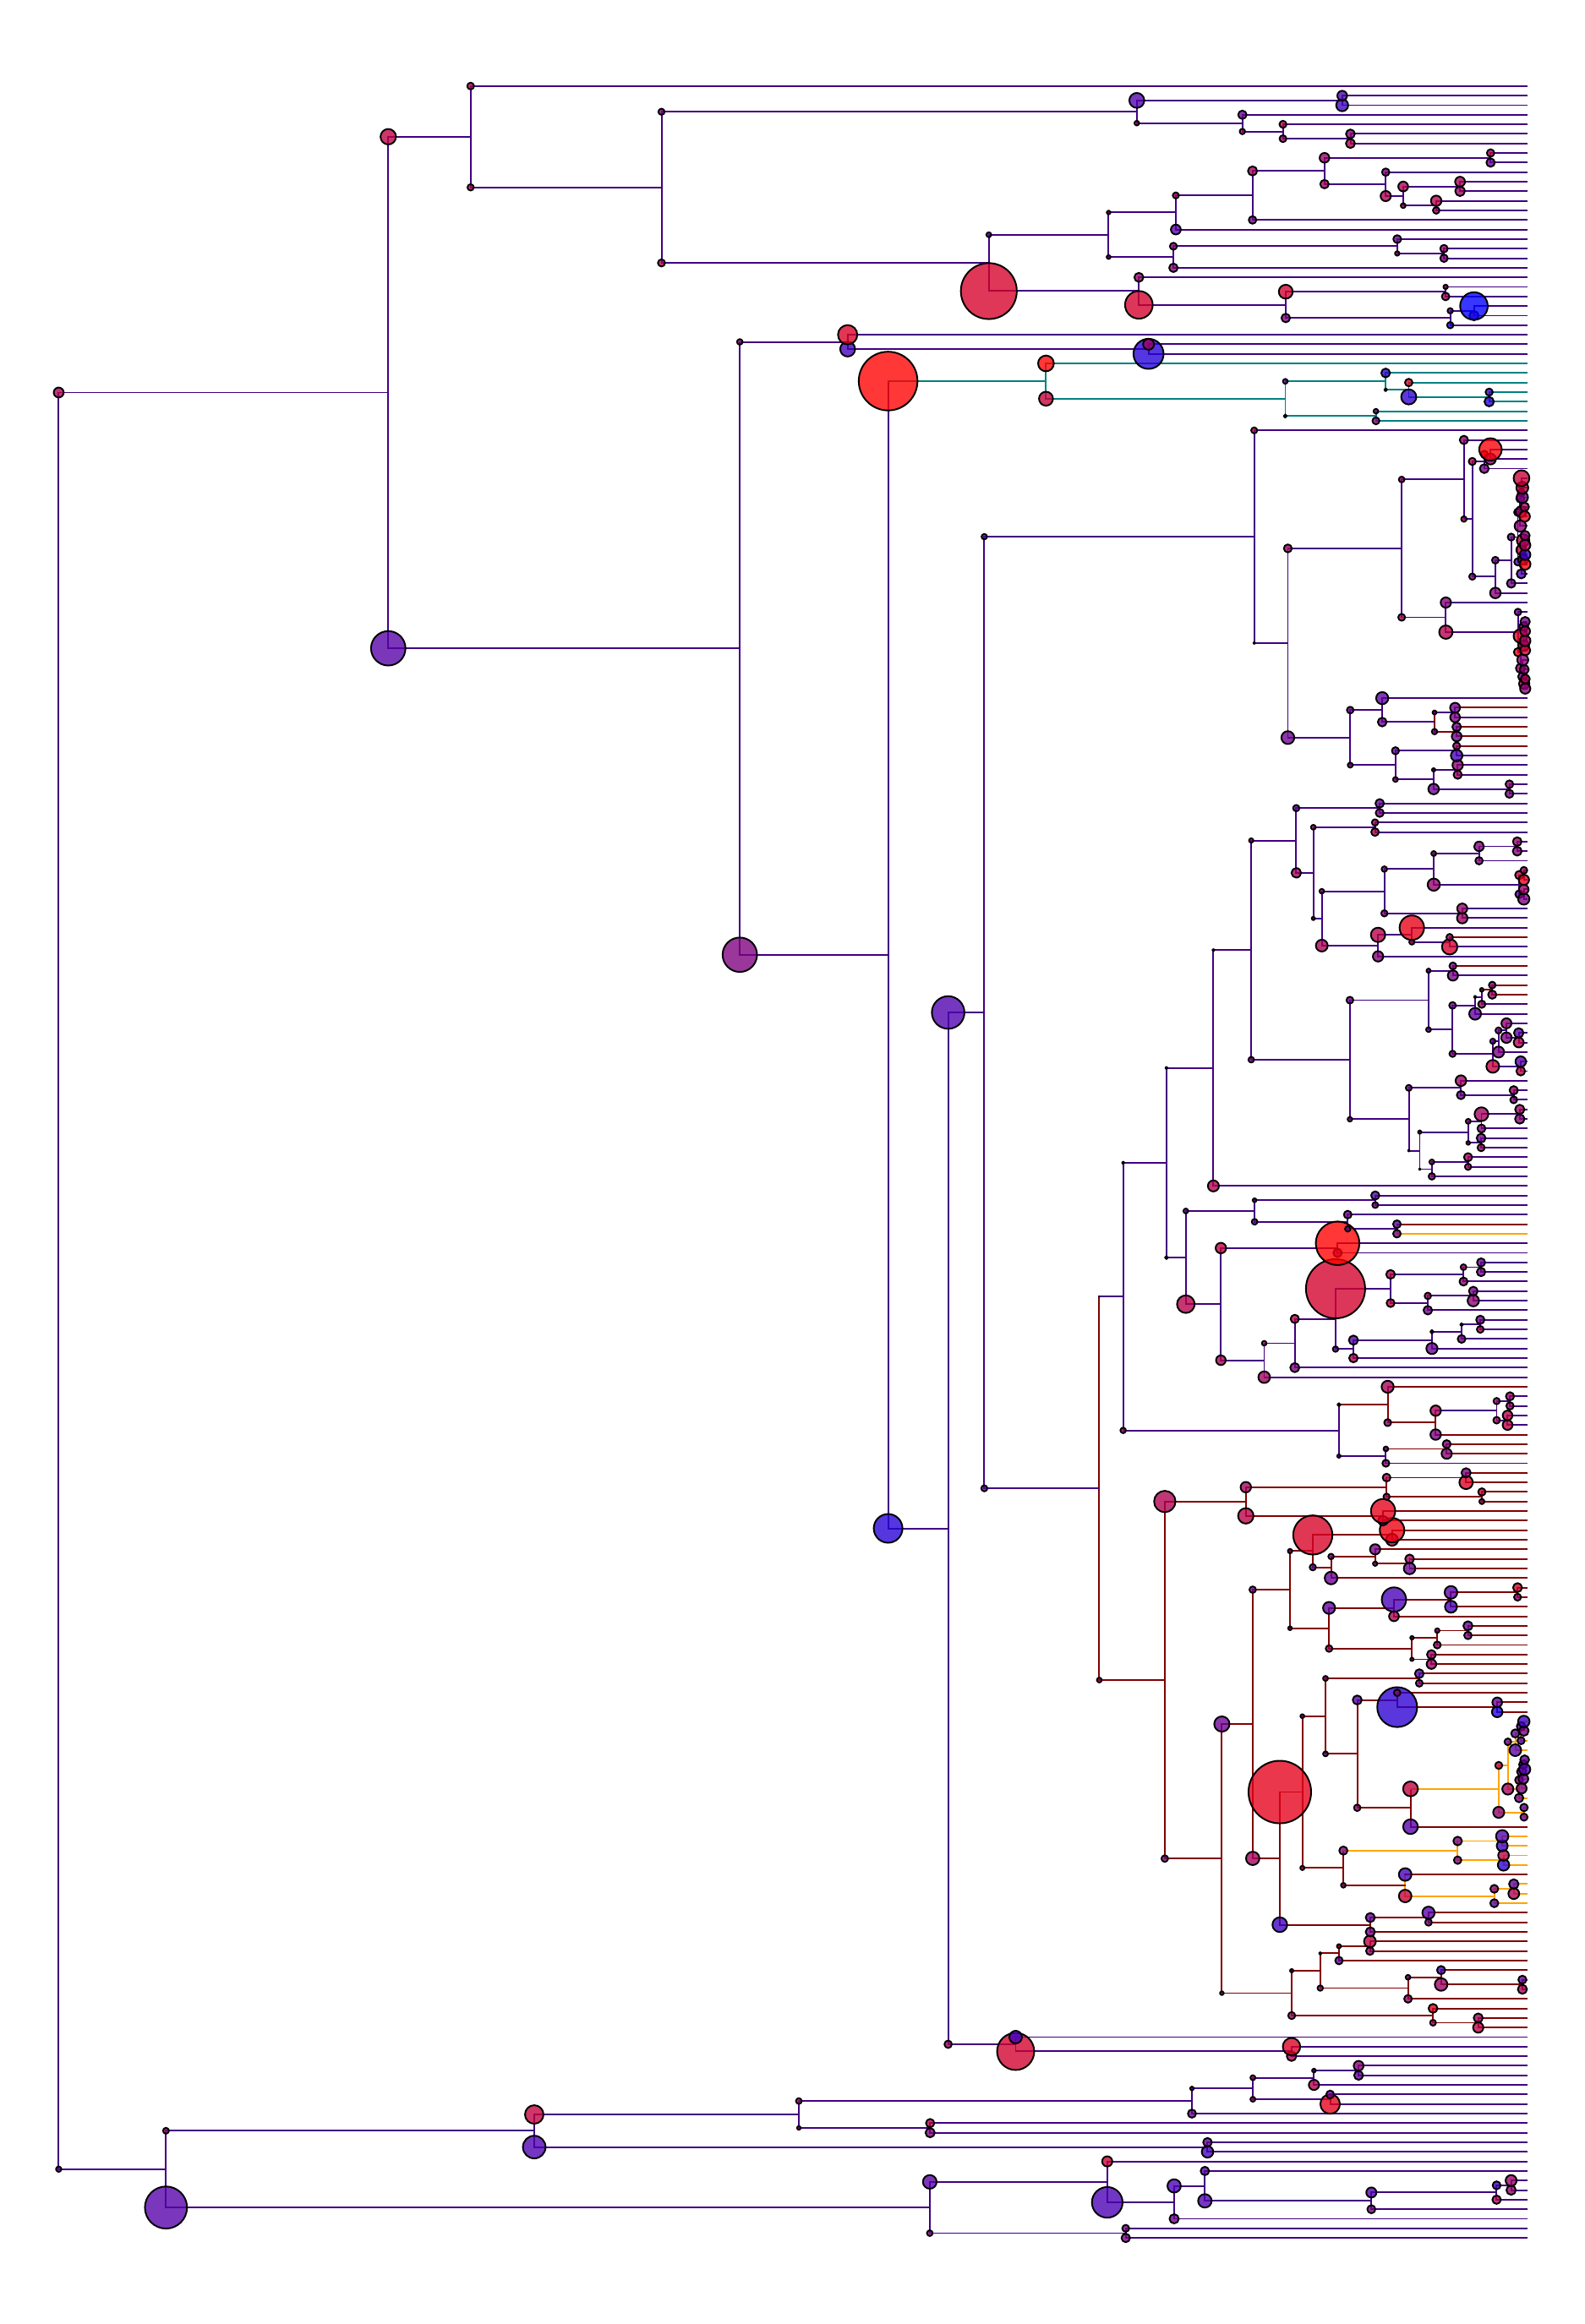} 

     {\sf \vskip -0.5cm \qquad bayou}
    %\caption{Result of the methods \printR{bayou} (circles at nodes) and \printR{SURFACE} (branch coloring). The size of the circles are proportional to their posterior probability, and their colors represents their values, from blue (negative) to red (positive). The $13$ colors on the edges represent the regimes found after convergence.}\label{fig:chelonia_sol_bayou}
\end{minipage}

    \begin{minipage}{0.45\textwidth}

\includegraphics[width=\maxwidth,height=0.45\textheight]{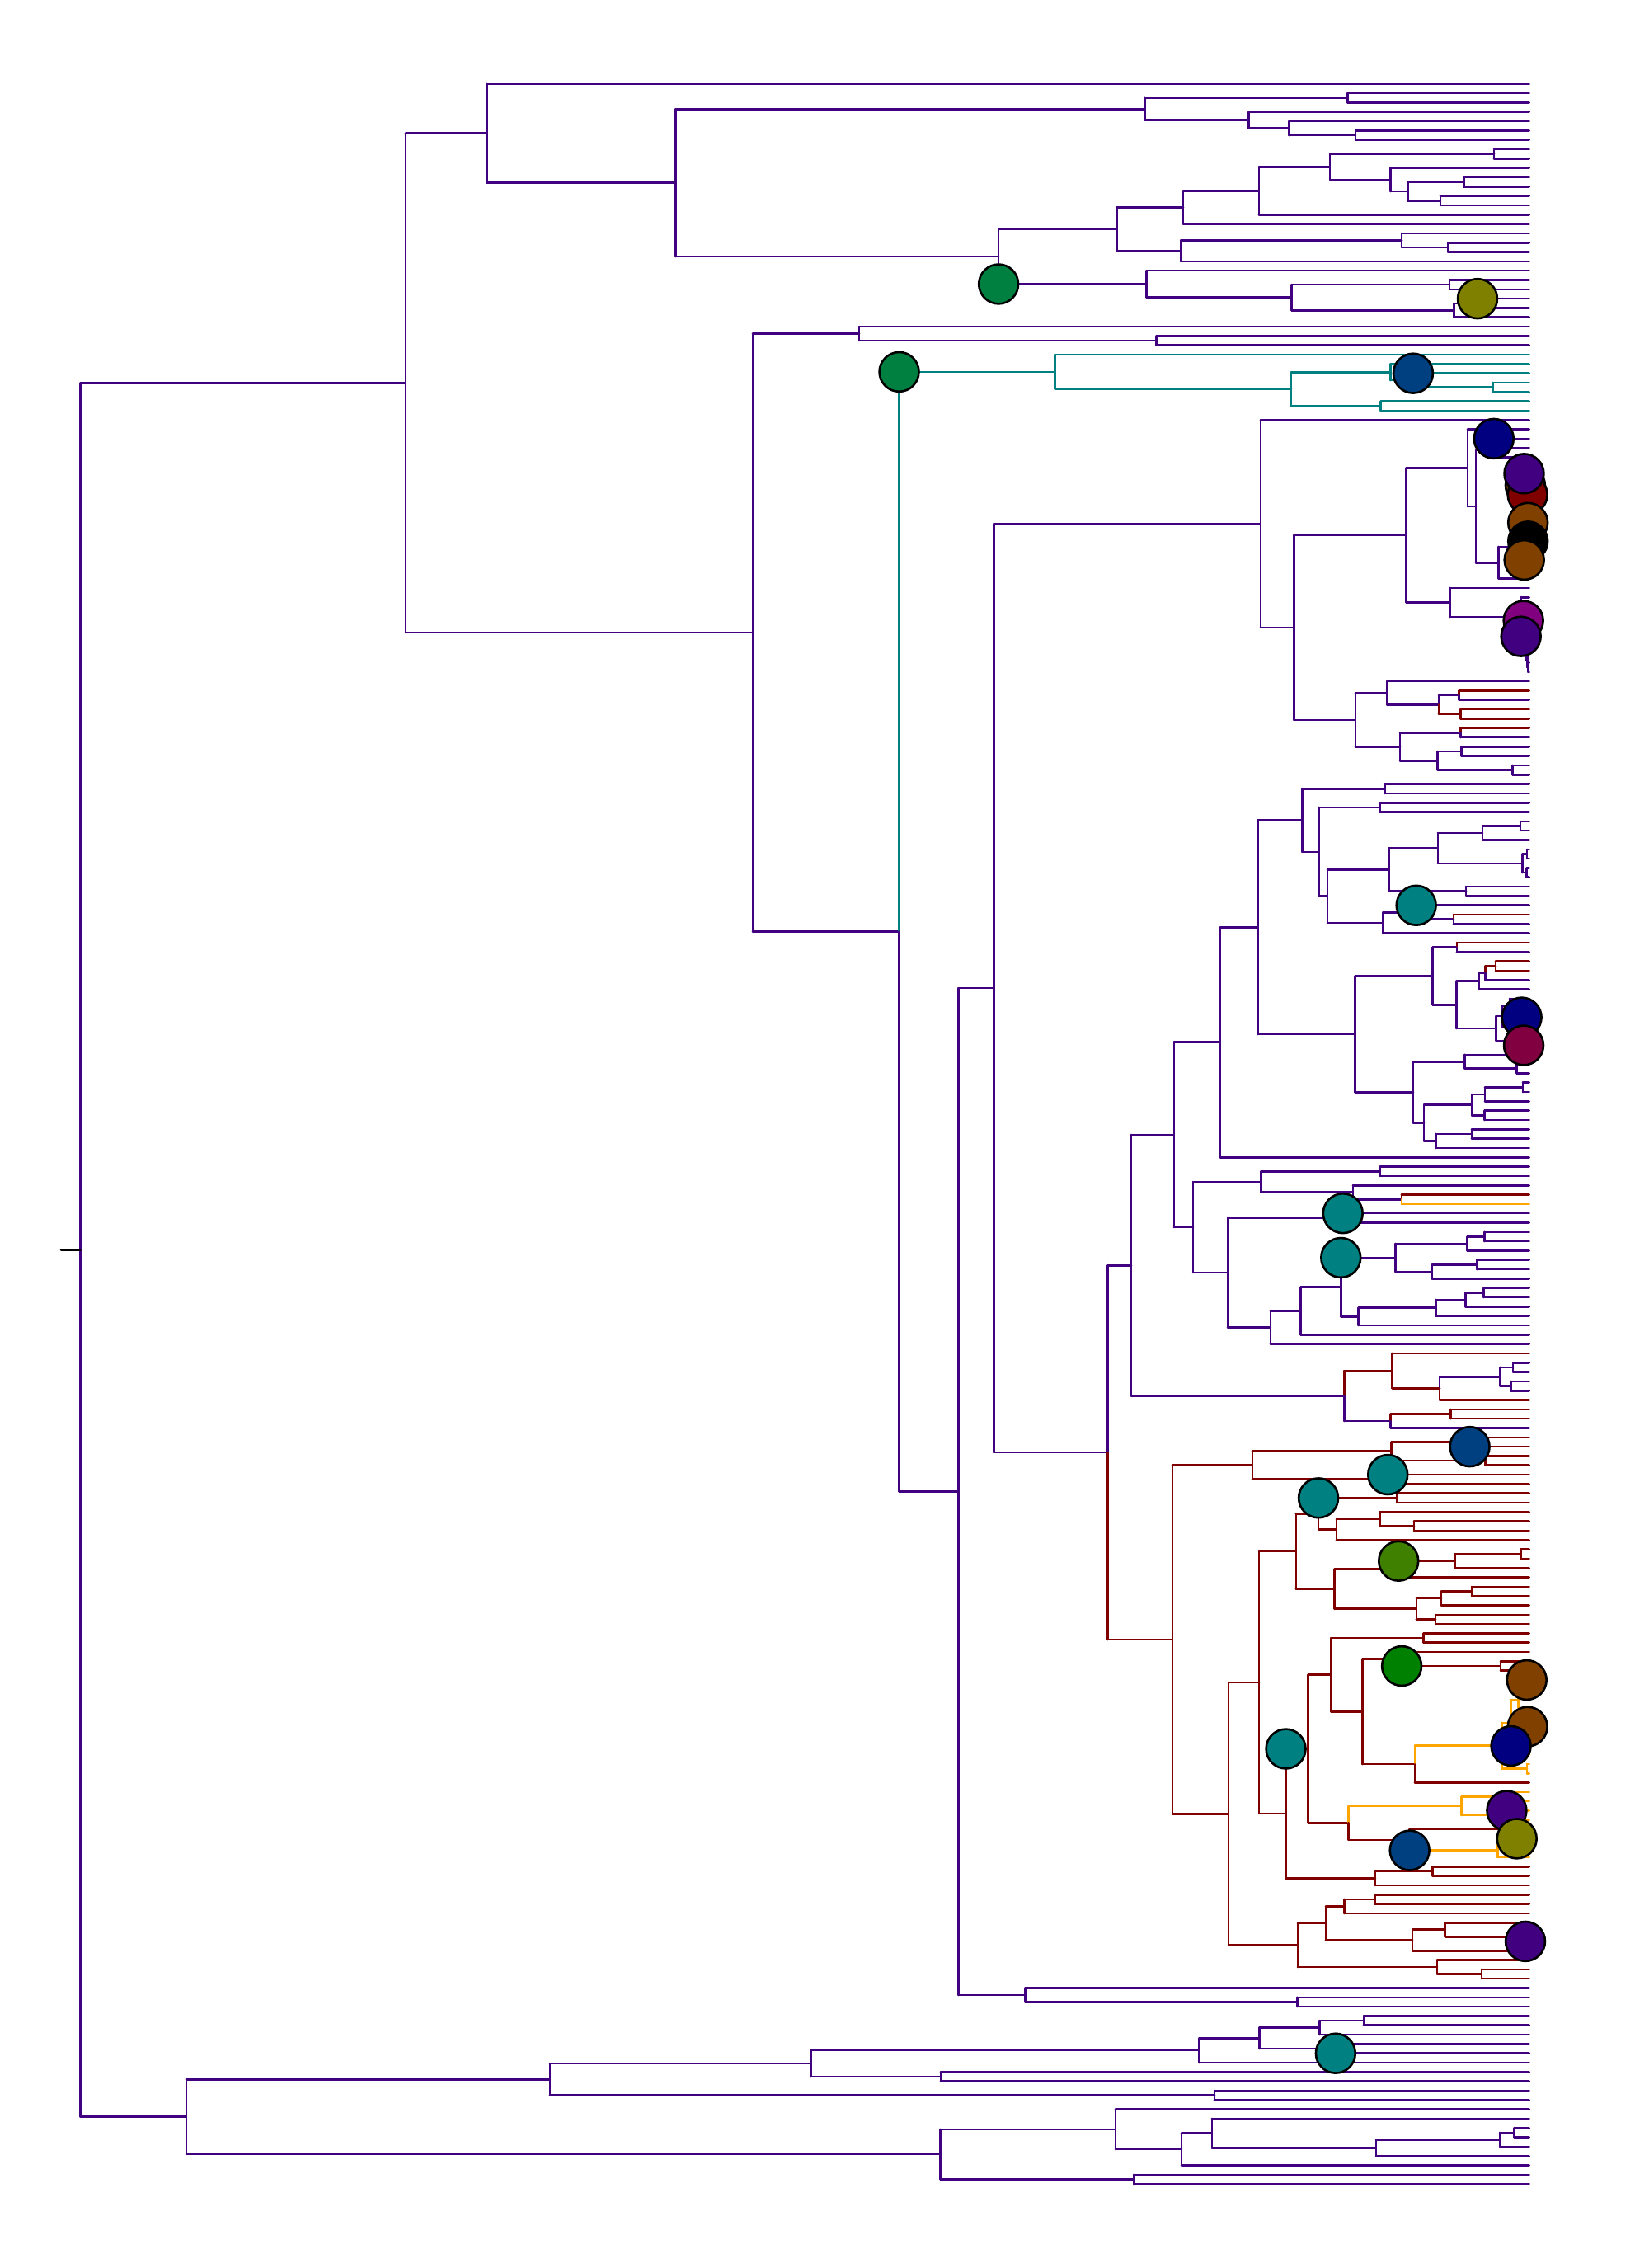} 

     {\sf \vskip -0.5cm \qquad SURFACE}
 \end{minipage}
 \begin{minipage}{0.45\textwidth}
%'     \vskip - 0.5 cm

\includegraphics[width=\maxwidth,height=0.45\textheight]{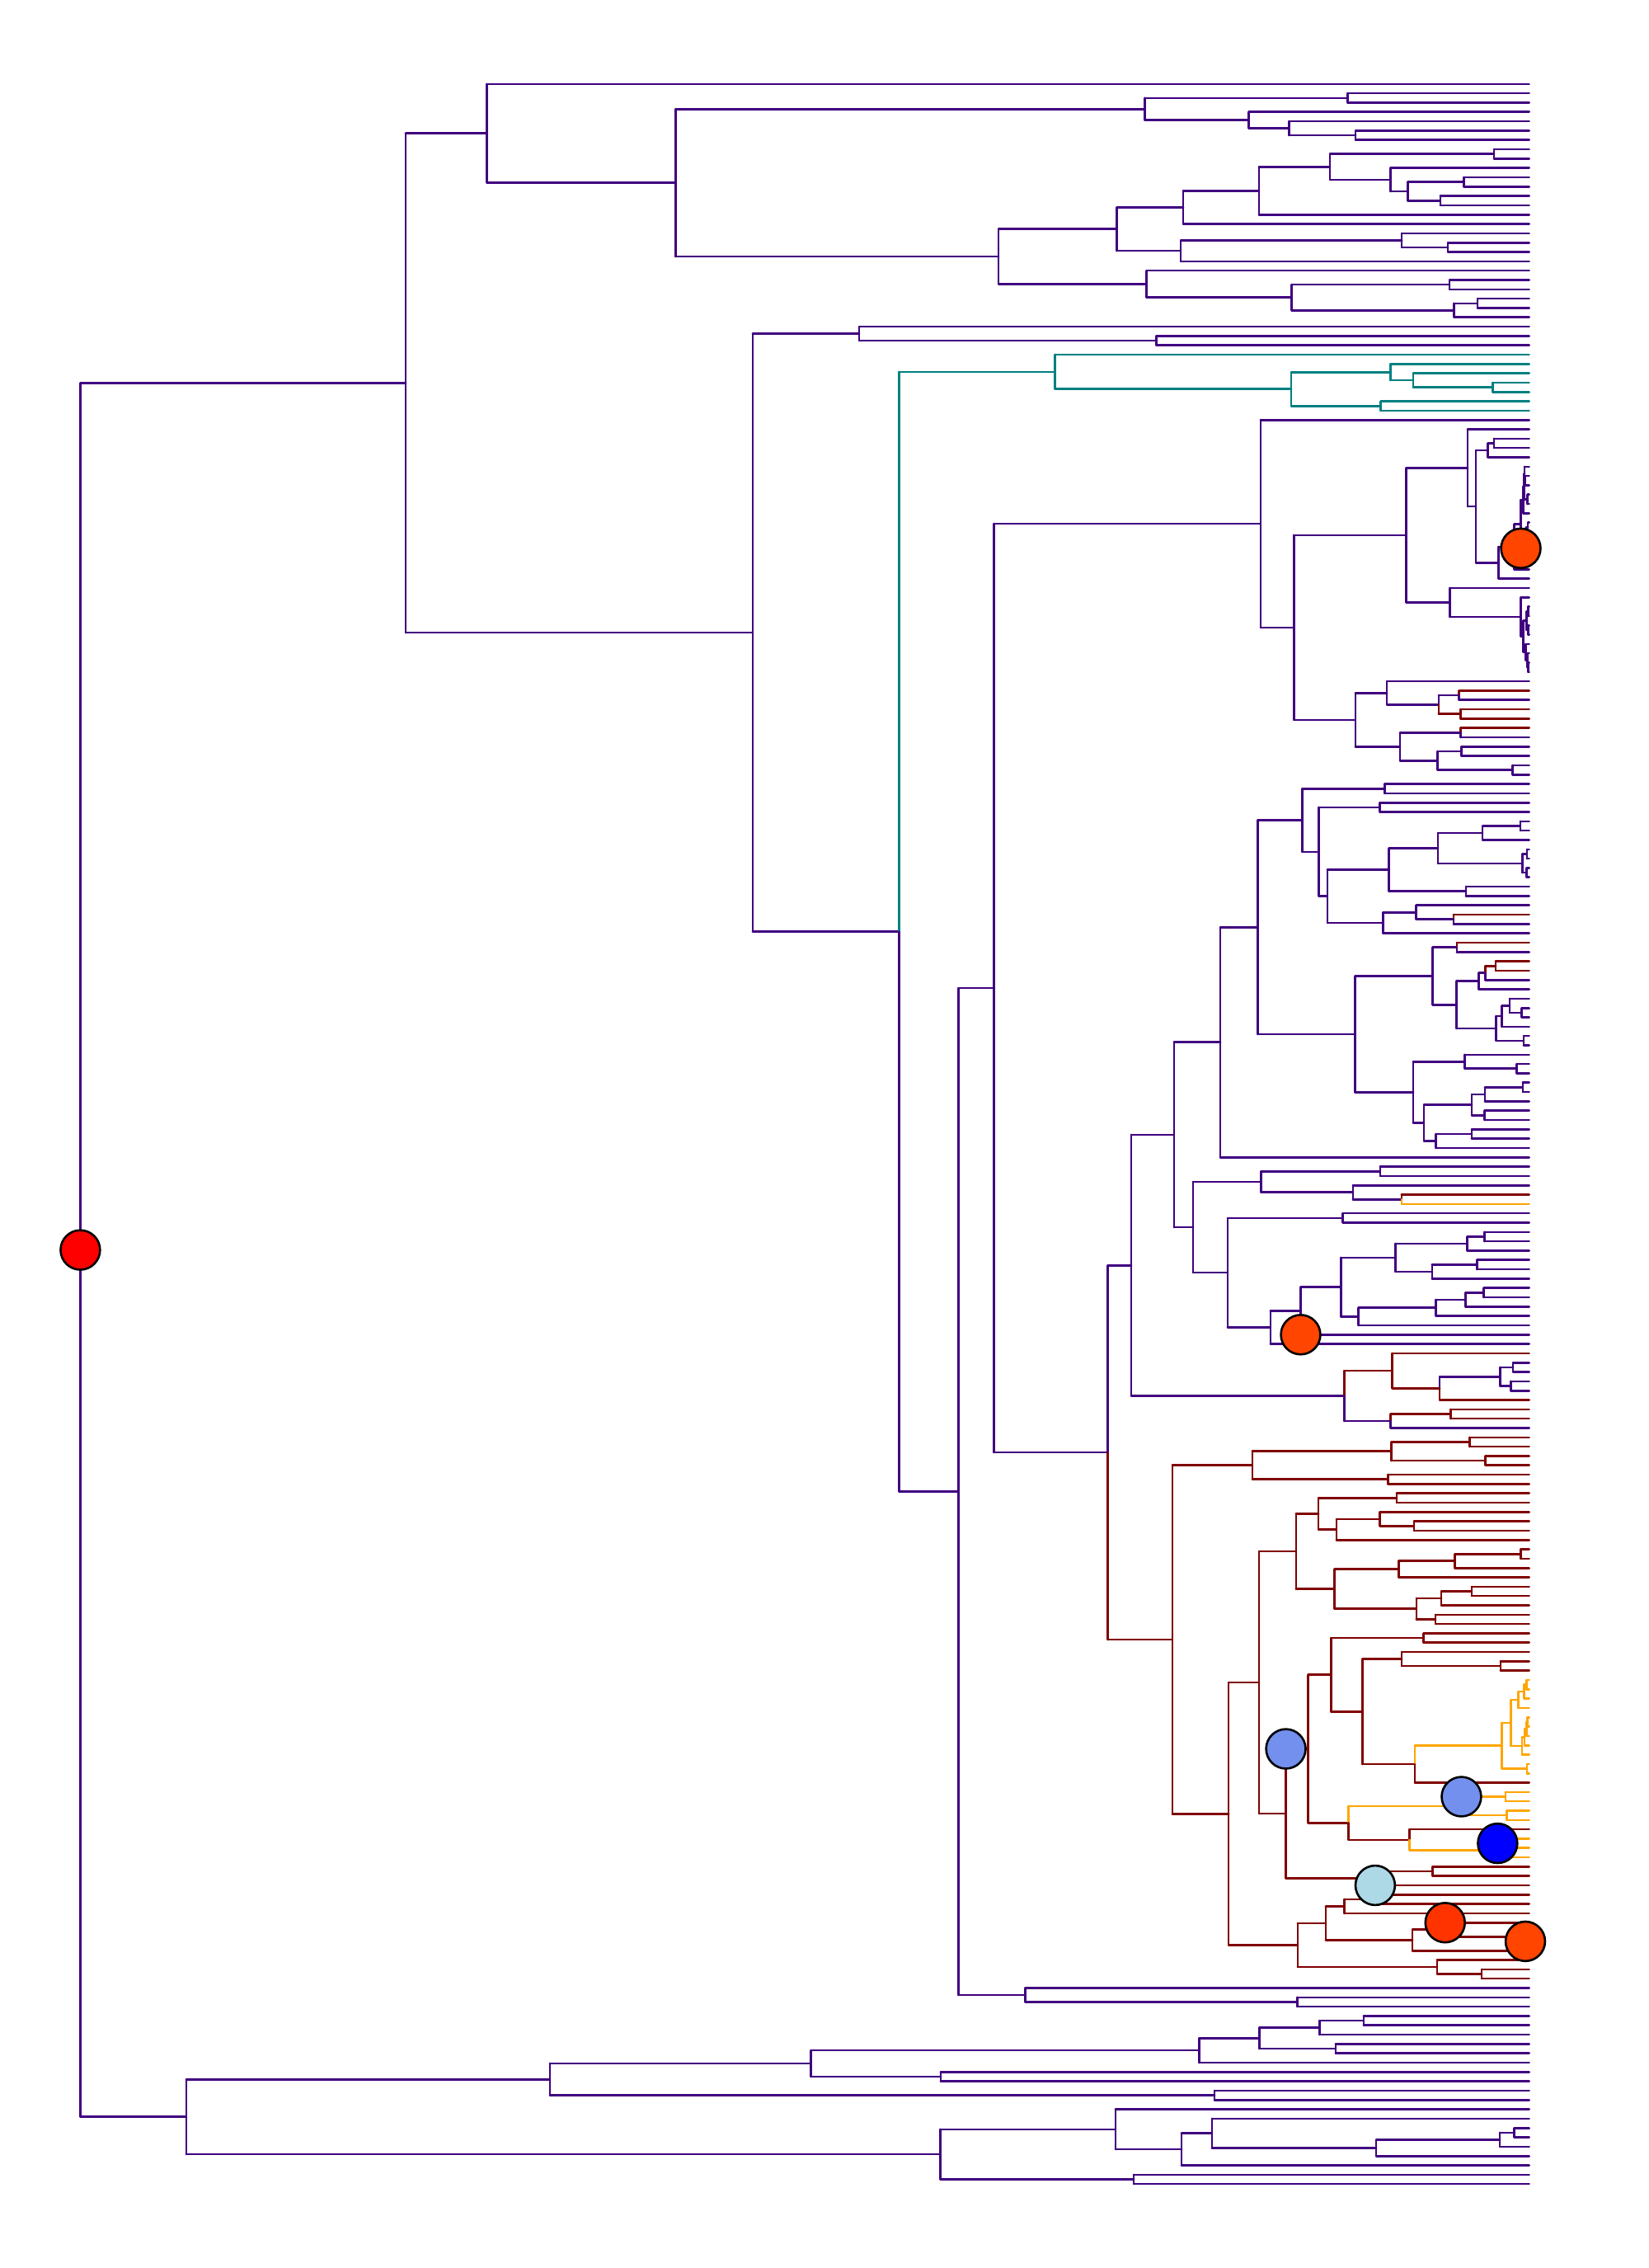} 

     {\sf \vskip -0.5cm \qquad OUshifts}
    \end{minipage}
        \caption{Solutions found by the EM (top left), \printR{bayou} (top right), \printR{SURFACE} (bottom left) and \printR{OUshifts} (bottom right). The branch coloring represents the habitats. For the EM, \printR{bayou} and \printR{OUshifts}, the shifts coloring represents their values, from blue (negative) to red (positive). For \printR{bayou}, the size of the circles are proportional to their posterior probability. For \printR{SURFACE}, the $13$ colors of the shifts represent the regimes.
}\label{fig:chelonia_sol_bayou}
 %   \caption{From top to bottom, solutions found by our method, \printR{bayou} and \printR{SURFACE}. The branch coloring represents the habitats. For our method and \printR{bayou}, the shift coloring represents their values, from blue (negative) to red (positive). For \printR{bayou}, the size of the circles are proportional to their posterior probability. For \printR{SURFACE}, the $13$ colors of the shifts represents the regimes.}

    \end{center}
  \end{figure}
