# Supplementary material for: Detection of adaptive shifts on phylogenies using shifted stochastic processes on a tree
Source: arXiv:1508.00225 source file (2016-07-13)
Supplement: Supplementary file 8 [file vandermonde.tex]

\section{A Vandermonde Like Identity}\label{supp:vandermonde}

\begin{proposition}

Let $(n,n') \in  N$ and $K \in \N$. With  the standard convention that
$\binom{n}{k} = 0$ if $n < k$, 
\begin{multline*}
\binom{n+n'-K}{K} = \sum_{k = 0}^K \binom{n-k}{k} \binom{n' - K + k}{K
  -k} \\ + \sum_{k = 0}^{K-1} \binom{(n-1)-k}{k} \binom{(n'-1) - (K-1) + k}{(K-1)
  -k}
\end{multline*}
which can be rewritten in a more symmetric way as:
\begin{multline}
  \label{eq:vandermonde_gen}
\binom{n+n'-K}{K}  =  \sum_{k,k'   \geq  0:  k+k'  =K}  \binom{n-k}{k}
\binom{n' - k'}{k'} \\ + \sum_{k,k' \geq 0: k+k' =K-1} \binom{(n-1)-k}{k} \binom{(n'-1) - k'}{k'}
\end{multline}

Similarly, 
\begin{multline*}
\binom{n+n'+1-K}{K} = \sum_{k = 0}^K \binom{n-k}{k} \binom{n' - K + k}{K
  -k} \\ + \sum_{k = 0}^{K-1} \binom{(n-1)-k}{k} \binom{n' - (K-1) + k}{(K-1)
  -k} + \binom{n-k}{k} \binom{(n'-1) - (K-1) + k}{(K-1) -k}
\end{multline*}
which can be rewritten in a more symmetric way as:
\begin{multline}
  \label{eq:vandermonde_gen_2}
\binom{n+n'+1-K}{K}  =  \sum_{k,k'   \geq  0:  k+k'  =K}  \binom{n-k}{k}
\binom{n'   -   k'}{k'}  \\   +   \sum_{k,k'   \geq   0:  k+k'   =K-1}
\binom{(n-1)-k}{k} \binom{n' - k'}{k'} + \binom{n-k}{k} \binom{(n'-1) - k'}{k'}
\end{multline}

\end{proposition}

Note that Eq~(\ref{eq:vandermonde_gen}) generalizes in some way the Vandermonde identity which states 
\begin{equation}
\label{eq:vandermonde}
\binom{n+n'}{K} = \sum_{k = 0}^K \binom{n}{k} \binom{n'}{K -k}
\end{equation}

Although  several  proofs  of   the  Vandermonde  identity  are  known
(geometric, algebraic and combinatorial),  we only provide a geometric
proof of this Vandermonde-like identity. 

Consider  a grid  of size  $(n+n') \times  K$.  We  are  interested in
grid-valued paths  that can move either  by $(1,0)$ or  by $(2,1)$. In
other words, if the $k^\text{th}$  position of a path is $(x_k, y_k)$,
then its next position $(x_{k+1}, y_{k+1})$ is either $(x_k + 1, y_k)$
or  $(x_k +  2, y_k  +1)$.   We are  interested in  paths starting  at
$(0,0)$ and ending at $(n+n', K)$.

Such a path consists of $K$ moves of type $(2,1)$ and $n+n'-2K$ moves of type
$(1, 0)$ and  is uniquely determined by the positions  of the moves of
the former type. There are $\binom {n+n'-2K + K}{K} = \binom
{n+n'-K}{K}$ distinct positions and therefore as many such paths. 

We now sort the paths according to the value $i$ they take when either
reaching  the line $x  = n$  or reaching  the line  $x =  n+1$ without
reaching the line  $x = n$ first.  We refer to  the latter paths as crossing
the line  $x = n$. Note that  this sorting induces a  partition of all
paths (see Figure~\ref{fig:vandermonde_1})

A path  reaching $x =  n$ at position  $i$ uniquely gives rise  to two
paths: one  from $(0,0)$ to $(n,  i)$ and one from  $(n,i)$ to $(n+n',
K)$  or equivalently  from $0$  to  $(n',K-i)$. There  are $\binom  {n
  -i}{i}$  different  paths  of  the  first kind  and  $\binom  {n'  -
  K-i}{K-i}$  of the second.   There are  therefore $\binom  {n -i}{i}
\binom {n' - K + i}{K - i}$ paths that pass through $(n,i)$.

A path crossing  the line $x=n$ and reaching the line  $x= n+1$ at $i$
must do so  with a last move of type $(2,  1)$.  It therefore uniquely
defines a path  from $(0,0)$ to $(n-1,i-1)$ and  a path from $(n+1,i)$
to $(n+n', K)$, or equivalently  from $(0, 0)$ to $(n'-1, K-i)$. There
are therefore $\binom {n -  i}{i - 1} \binom {n' - 1 -  K + i}{K - i}$
paths that cross the line $x = n$ and pass through $(n+1, i)$. 

Putting everything together, we get:
\begin{eqnarray*}
\binom{n+n'-K}{K} & = & \sum_{i = 0}^K \binom{n-i}{i} \binom{n'-K+i}{K-i}
+ \sum_{i = 0}^K \binom{n-i}{i - 1} \binom{n'- 1 - K+i}{K-i} \\ 
 & = & \sum_{i = 0}^K \binom{n-i}{i} \binom{n'-K+i}{K-i}
+ \sum_{i = 0}^{K-1} \binom{(n-1) -i}{i} \binom{(n'- 1) - (K-1) +i}{(K-1)-i}
\end{eqnarray*}
which is exactly Eq.~(\ref{eq:vandermonde_gen}). 

\begin{figure}
  \begin{center}    
    \includegraphics[width = 0.6\linewidth]{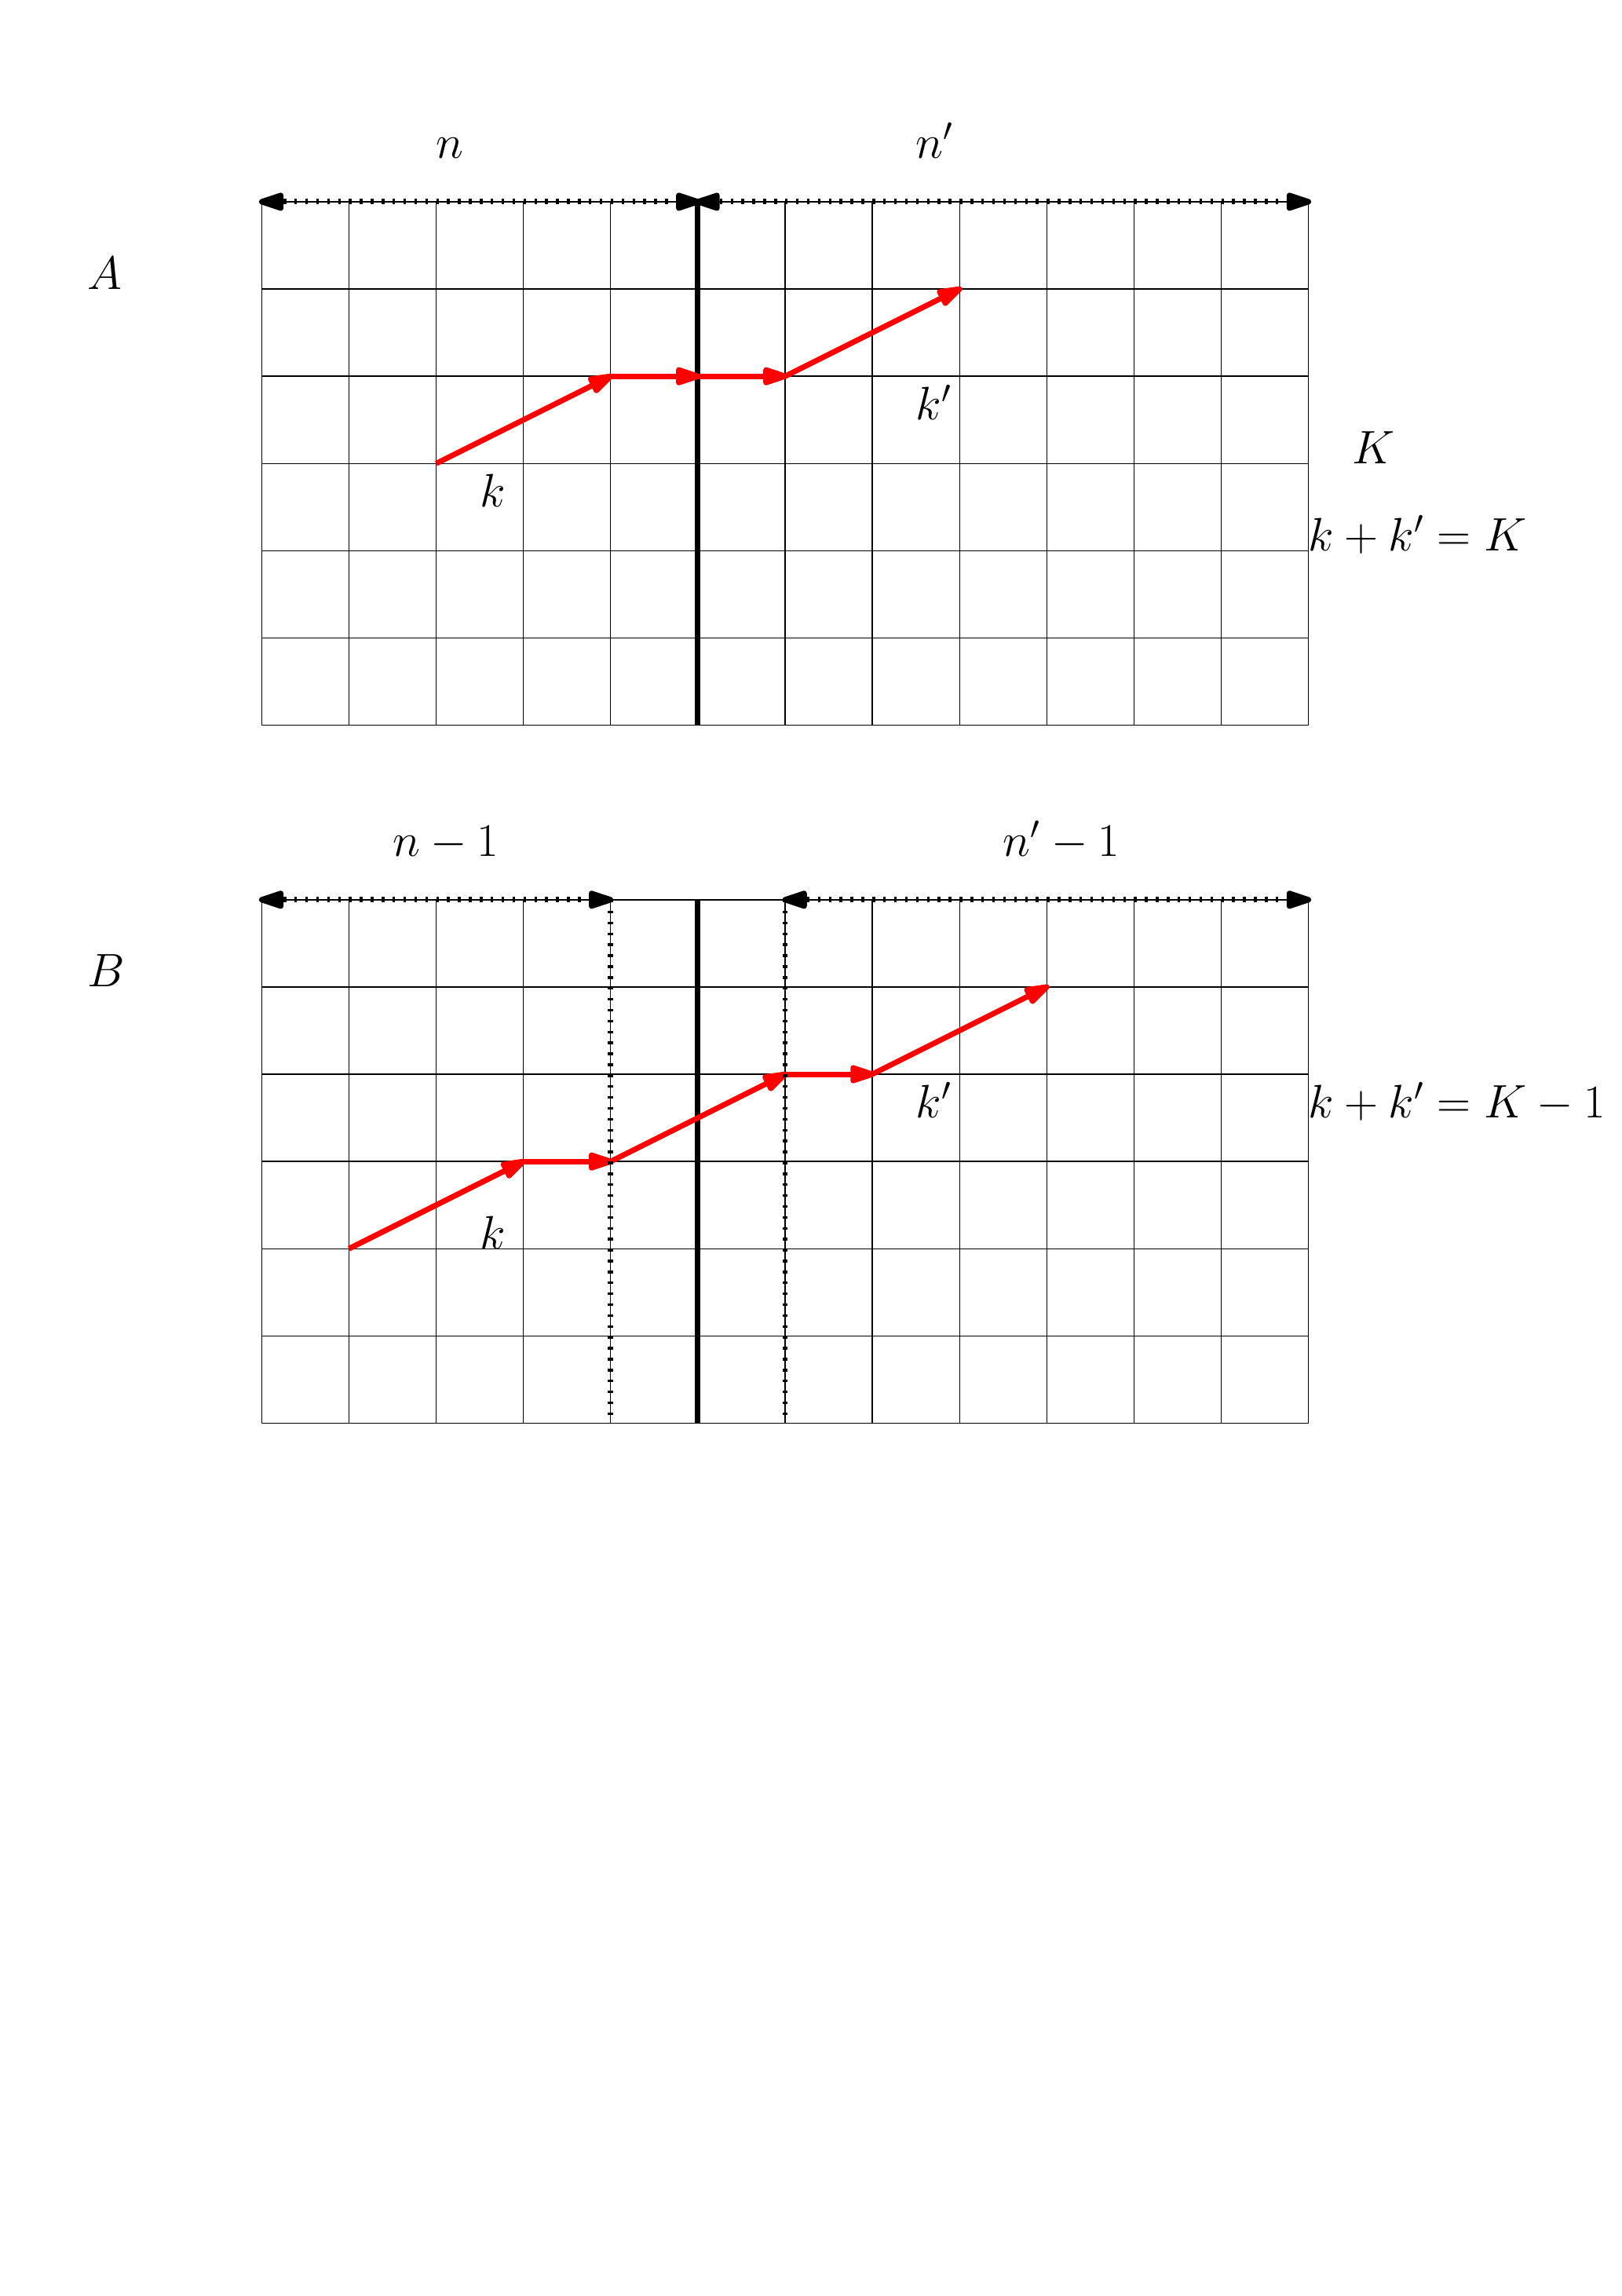}
    \caption{\label{fig:vandermonde_1}  Partition of paths  according to
      whether they reach (A) or cross (B) the line $x=n$}
  \end{center}
\end{figure}

To  prove Eq.~(\ref{eq:vandermonde_gen_2}),  we start  from a  grid of
size  $(n+n'+1)  \times K$  and  are  again  interested in  the  paths
starting from  the bottom  left corner and  ending in the  upper right
corner using  only (2, 1) and  (1, 0) moves. These  paths have exactly
$K$ moves  of type  (2, 1)  and there are  $\binom{n+n'+1 -  K}{K}$ of
them. This time, we partition paths upon the move observed between $x = n$
and $x=(n+1)$.

The move can be (see also Figure~\ref{fig:vandermonde_2}):
\begin{itemize}
\item (1, 0), in which case $k$ (resp. $k'$) moves of type $(2, 1)$
  are used in  the interval $[1, n]$ (resp.  $[n+1, n+n'1]$) such that
  $k + k' = K$;
\item (2, 1) starting from $x=n$ and therefore ending at $x=n+2$, in which case $k$
  (resp. $k'$)  moves of type $(2,  1)$ are used in  the interval $[1,
  n]$ (resp.  $[n+2, n+n'1]$) such that $k + k' = K - 1$ (one move (2,
  1) has already been consumed);
\item (2, 1) ending at $x=n+1$ and therefore starting from $x = n-1$ in which case $k$
  (resp. $k'$)  moves of type $(2,  1)$ are used in  the interval $[1,
  n-1]$ (resp.  $[n+1, n+n'1]$) such that $k + k' = K - 1$ (one move (2,
  1) has already been consumed);
\end{itemize}

Wrapping everything  together and using the same  arguments as before,
we get Eq.~(\ref{eq:vandermonde_gen_2}). 

\begin{figure}
  \begin{center}
    \includegraphics[width = 0.6\linewidth]{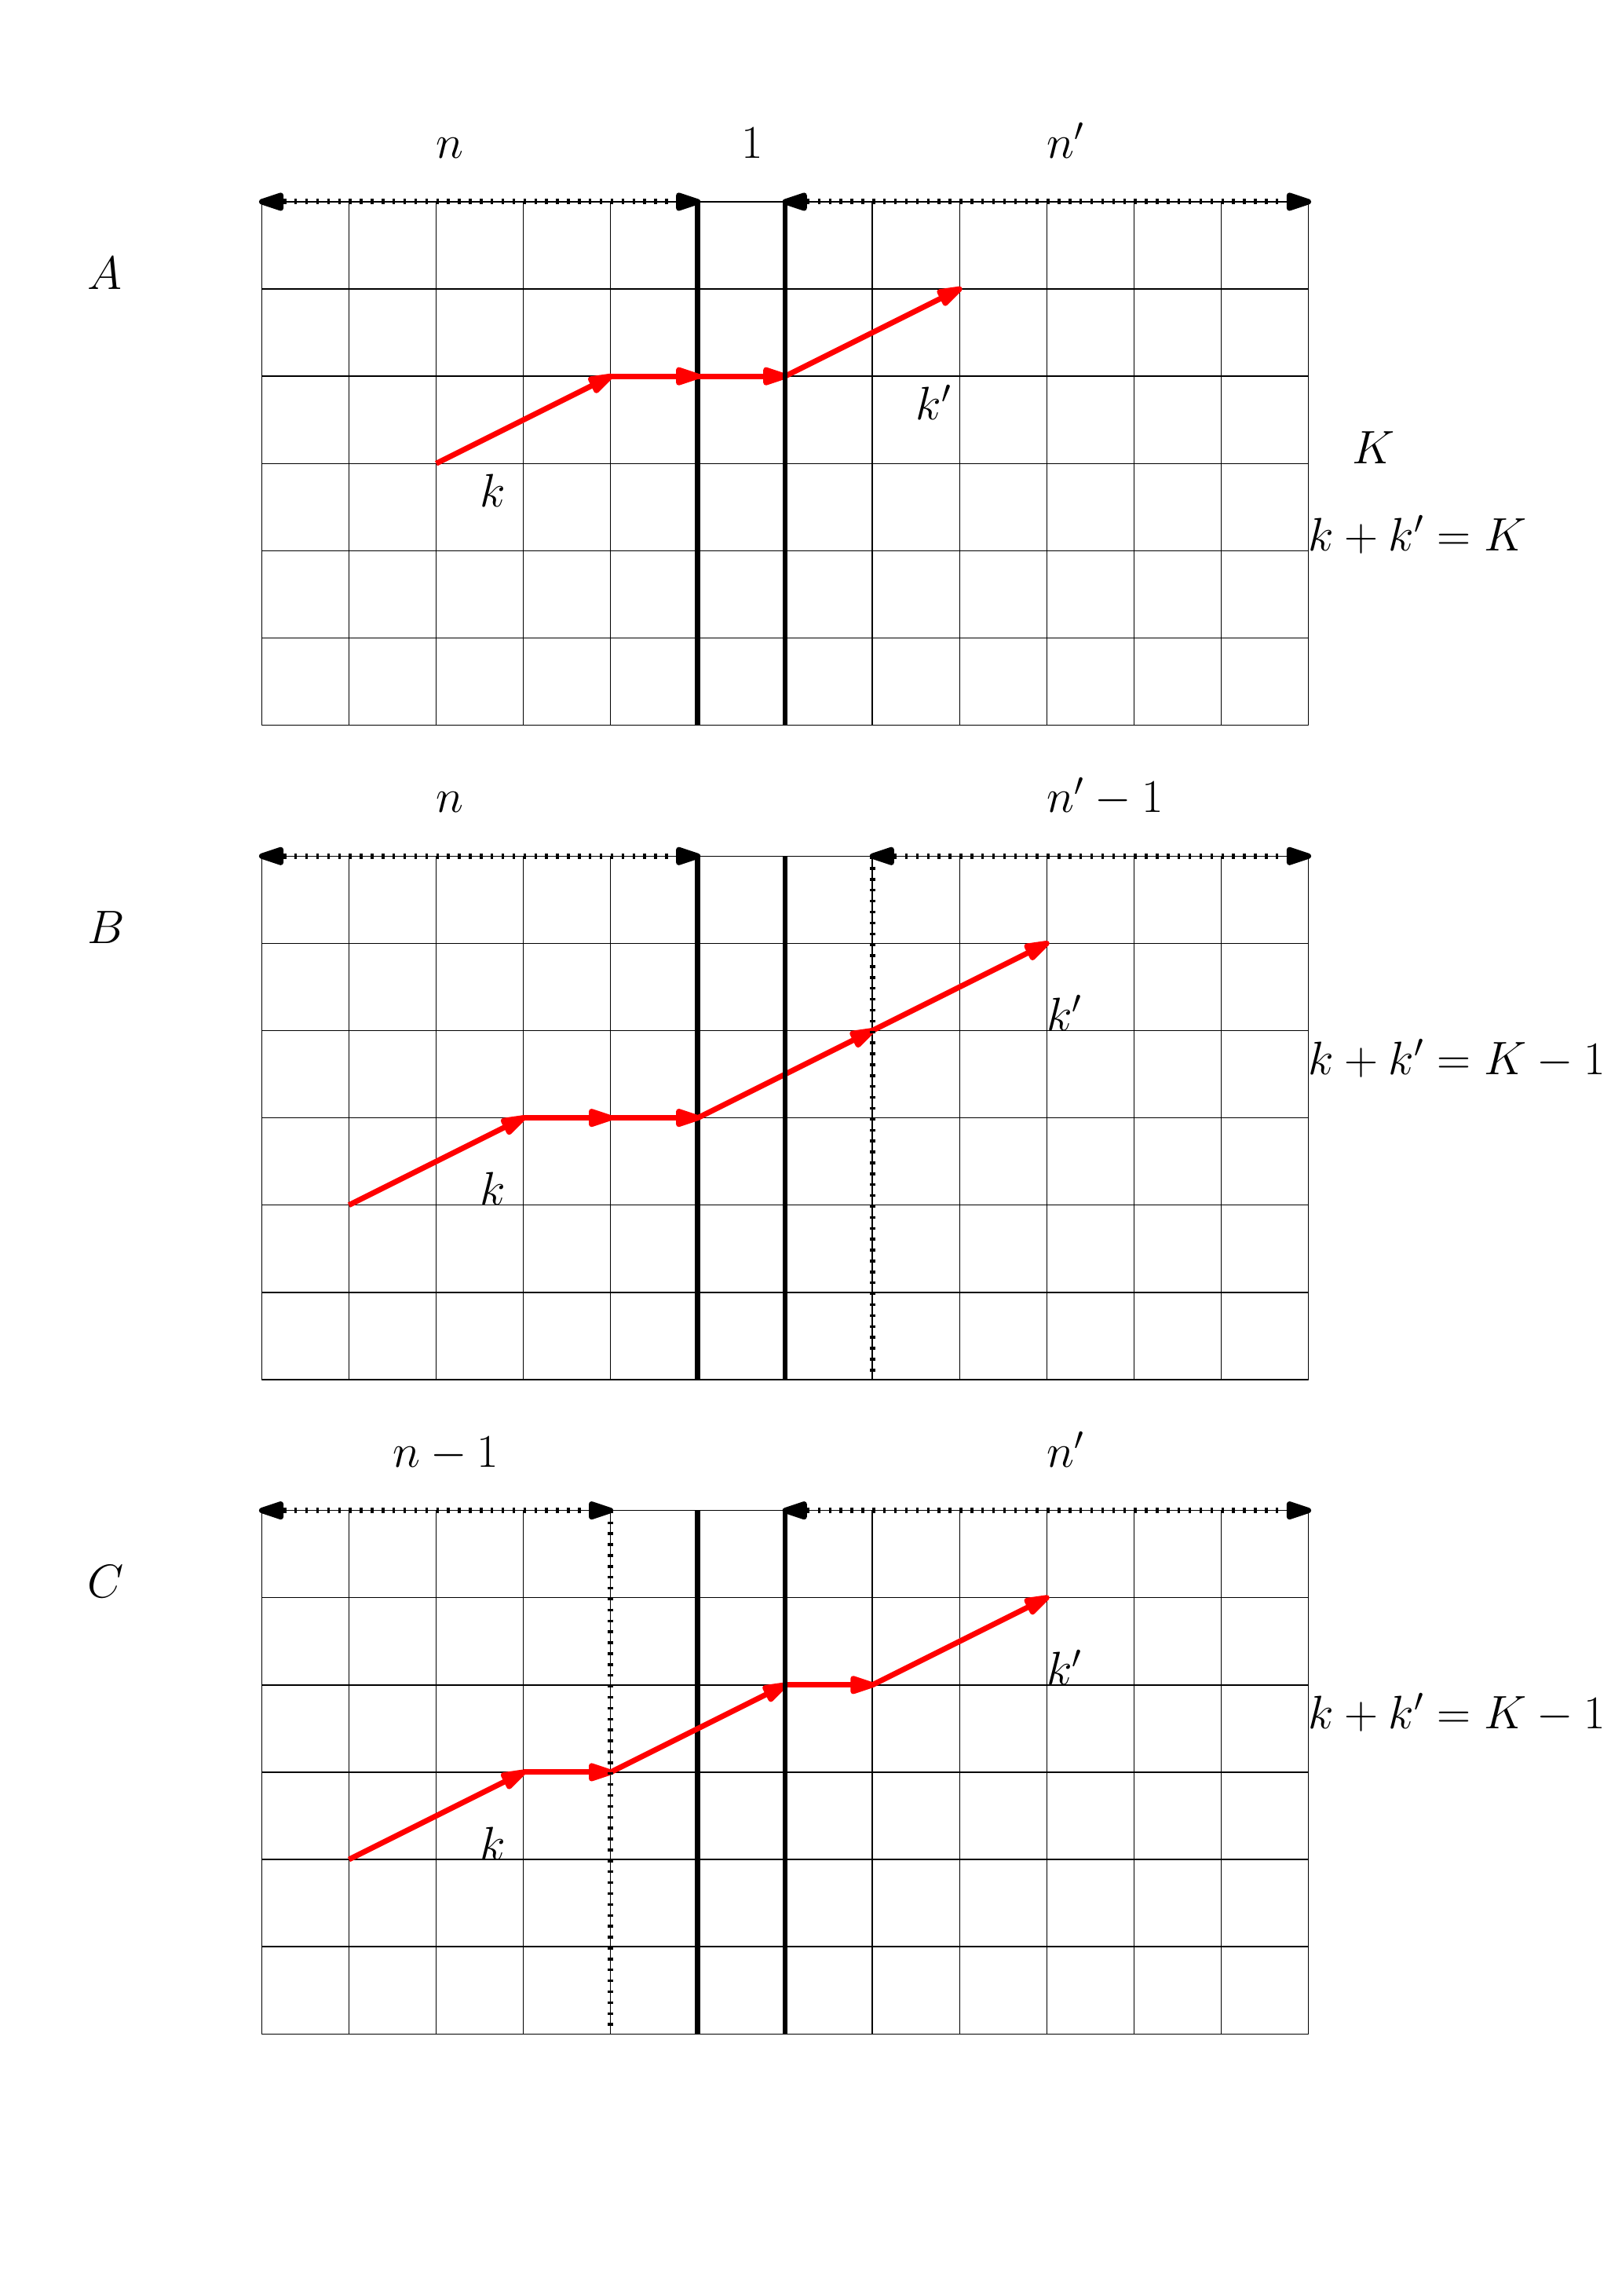}
    \caption{\label{fig:vandermonde_2}  Partition of paths  according to
      whether to  the move  used between $x=n$  and $x=n+1$. Cases  A, B
      and C correspond to the items listed in the main text.}
  \end{center}
\end{figure}
